# Supplementary material for: Online Statistical Inference for Nonlinear Stochastic Approximation with Markovian Data
Source: arXiv:2302.07690 source file (2026-08-10)
Supplement: Supplementary file 1 [file appendix.tex]

\begin{center}
{\huge \textbf{Appendices}}
\end{center}

\section{Weak convergence in metric spaces}
We will introduce some basic knowledge of weak convergence in metric spaces.
See Section 12-15 of~\citep{billingsley2013convergence} for a detailed introduction.

A Polish space is a topological space that is separable, complete, and metrizable.
Let $\BDD = \{  \ph: \text{càdlàg function}~\ph(r) \in \RB^d,r \in [0, 1]  \}$ collect all $d$-dimensional functions which are right continuous with left limits.
The $J_1$ \textit{Skorokhod topology} equips $\BDD$ with the \textit{Skorokhod metric} $\dS$ such that $(\BDD, \dS)$ is a Polish space and $\BDM$ is its Borel $\sigma$-field (the $\sigma$-field generated by all open subsets) in the Skorokhod metric. 
In particular, denoting by $\Lambda$ the class of strictly increasing continuous mappings $\lambda: [0,1] \to [0, 1]$ with $\lambda(0) =0$ and $\lambda(1) = 1$, we have for any $\ph_1, \ph_2 \in \BDD$,
\begin{equation}
	\label{eq:d0}
	\dS(\ph_1, \ph_2) = \inf_{\lambda \in \Lambda} \max\left\{
	\sup_{0\le s < t \le 1}\left|\ln\frac{\lambda(t)-\lambda(s)}{t-s}\right|, \sup_{t \in [ 0,1]}\|\ph_1(\lambda(t)) - \ph_2(t)\|
	\right\}.
\end{equation}

An important closed subset of $\BDD$ is $\BCD := \{ \ph: \text{continuous}~\ph(r) \in \RB^d,r \in [0, 1]  \}$, which collects all $d$-dimensional continuous functions defined on $[0, 1]$.
The \textit{uniform topology} equips $\BCD$ with the uniform metric $\vertiii{\ph} := \sup_{r \in [0, 1]} \|\ph(r)\|$ such that $(\BCD,\vertiii{\cdot})$ is a Polish space.
Furthermore, we have $\dS(\ph_1, \ph_2) \le \vertiii{\ph_1-\ph_2}$ for any $\ph_1, \ph_2 \in \BDD$, implying the $J_1$ Skorokhod topology is weaker than the uniform topology.
Unfortunately, $(\BDD, \vertiii{\cdot})$ is not separable and we have $\BDM \subsetneq \BCM$ with $\BCM$ the Borel $\sigma$-field in the uniform metric.
%However, a sequence $\{\ph_t\}_{t \ge 0}  \subseteq \BDD$ converges to $\ph \in \BCD$ under the Skorokhod metric $\dS$ if and only if it converges to $\ph$ under the uniform metric $\vertiii{\cdot}$.
%Hence, the Skorokhod topology relativized to $\BCD$ coincides with the uniform topology there.
%In our paper, the interested $\ph$ would be a (continuous) scaled Brownian motion and $\ph_t$ is a stage-wise constant function, implying no difference in defining convergence using the uniform topology or the $J_1$ Skorokhod topology.

Any random element $\ph_t \in \BDD$ introduces a probability measure on $\BDD$ denoted by $\LM(\ph_t)$ such that $(\BDD, \BDM, \LM(\ph_t))$ becomes a probability space.
We say a sequence of random elements $\{\ph_t\}_{t \ge 0}  \subseteq \BDD$ \textit{weakly converges} to $\ph$, if for any bounded, continuous, $\BDM$-measurable functional $f: \BDD \to \RB$, we have $\EB f(\ph_T) \to \EB f(\ph)$ as $T \to \infty$.
The condition is equivalent to that any finite-dimensional projections of $\ph_T$ converge in distribution in the sense that 
for any given integer $n \ge 1$ and any $0 \le t_1  < \cdots < t_n \le 1$, when $T$ goes to infinity,
\begin{equation}
	\label{eq:finite-proj}
	(\ph_T(t_1), \ph_T(t_2), \cdots, \ph_T(t_n))
	\overset{d}{\to} (\ph(t_1), \ph(t_2), \cdots, \ph(t_n)).
\end{equation}
%We can similarly define weakly convergence in the uniform topology by replacing $\BDD, \BDM$ with $\BCD, \BCM$. 
We denote weak convergence by $\ph_T \overset{w}{\to} \ph$.
If further $\ph \in \BCD$, we have $\ph_T \overset{w}{\to} \ph$ if and only if $\EB f(\ph_T) \to \EB f(\ph)$ for any bounded, continuous, $\BCM$-measurable functional $f: \BDD \to \RB$.
Therefore, if $\ph_T \overset{w}{\to} \ph \in \BCD$, we then have $f(\ph_T) \overset{d}{\to} f(\ph)$ for any $\vertiii{\cdot}$-continuous functional $f$.
Slutsky’s theorem also holds here; for $\ph_T^{(1)},  \ph_T^{(2)} \in \BDD$ satisfying $\ph_T^{(1)} \overset{w}{\to} \ph$ and $ \dS(\ph_T^{(2)}, \ph_T^{(1)}) \overset{d}{\to}  0 $, we have $ \ph_T^{(2)} \overset{w}{\to} \ph$.

%\paragraph{Metrics for probability measures}
%The L\'evy metric is a metric on the space of cumulative distribution functions of one-dimensional random variables.
%For two random variable $X_1, X_2 \in \RB$, the L\'evy distance between $X_1$ and $X_2$ is
%\[
%\dL(X_1, X_2) := \inf\left\{\eps: \PB(X_2 \le x-\eps) -\eps \le \PB(X_1 \le x) \le  \PB(X_2 \le x+\eps) + \eps ~\forall x \in \RB  \right\}.
%\]
%
%
%
%Since $(\C_{[0,1]}, \|\cdot\|_\infty)$ is separable, convergence of measures in the Lévy–Prokhorov metric is equivalent to weak convergence of measures.
%We relate L\'evy-Prokhorov metric with a Ky-Fan-metric-type functional $\Tilde{d}(\cdot)$ that would be frequently used latter on.
%For any continuous stochastic process $\vy\in \C_{[0,1]}$, we denote 
%\begin{equation}
%	\label{eq:kfm}
%	\Tilde{d}(\vy) := \inf\limits_\eps \eps\vee \PB(\|\vy\|_\infty > \eps).
%\end{equation}
%What's more, any $\vy$ introduces a probability measure on $(\C_{[0,1]}, \gC_{[0,1]})$, which we denote by $\PB\circ \vy^{-1}$ with definition that $\PB\circ \vy^{-1}(B) = \PB(\vy \in B)$ for any $B \in \gC_{[0,1]}$.

\section{Omitted proofs for the FCLT}
\label{proof:fclt}

\subsection{Proof of Lemma~\ref{lem:poisson}}
\label{proof:poisson}

We first introduce an important consequence from Assumption~\ref{asmp:markov-noise} that would be used frequently later.
\begin{lem}
\label{lem:geo-con}
Under Assumption~\ref{asmp:markov-noise}, for any measurable uniformly bounded function $\sh: \Xi \to \RB^d$, we  
we have for any $t \ge 0$,
\begin{equation}
	\label{eq:geo-con}
	\sup_{\xi \in \Xi}	\| \PM^t  \sh(\xi)- \EB_{\xi \sim \DM}\sh(\xi) \| \le \kappa  \rho^t \cdot \sup_{\xi \in \Xi}\|\sh(\xi)-\EB_{\xi \sim \DM}\sh(\xi)\|.
\end{equation}
\end{lem}
\begin{proof}[Proof of Lemma~\ref{lem:geo-con}]
	Define an auxiliary function $\sh_0(\xi) := \sh(\xi)-\EB_{\xi \sim \pi}\sh(\xi)$.
	Since $\sh(\cdot)$ is uniformly bounded, so is $\sh_0(\cdot)$.
	Furthermore, $\EB_{\xi \sim \pi} \sh_0(\xi) = \0$.
	By Strassen’s duality theorem, let $\xi_{\infty} \in \Xi$ denote the random variable with distribution $\pi$ that satisfies $ 	\dTV(  \PM^t(\xi, \cdot), \pi )  = \PB(\xi_t \neq \xi_{\infty}|\xi_0=\xi)$.
	Then
	\begin{align*}
		\| \PM^t  \sh_0(\xi)\|	
		&=	\| \EB[\sh_0(\xi_t)|\xi_0=\xi] \|
		=\| \EB[\sh_0(\xi_t) -\sh_0(\xi_{\infty})|\xi_0=\xi] \|\\
		&=\| \EB[(\sh_0(\xi_t) -\sh_0(\xi_{\infty})) \cdot 1_{ \xi_t \neq \xi_{\infty} }  |\xi_0=\xi] \|\\
		&\le \sup_{\xi_t, \xi_{\infty}} \|\sh_0(\xi_t) -\sh_0(\xi_{\infty}) \| \cdot \PB(\xi_t \neq \xi_{\infty}|\xi_0=\xi)\\
		&\le 2 \sup_{\xi \in \Xi}\| \sh_0(\xi)\| \cdot \dTV(  \PM^t(\xi, \cdot), \pi )\\
		&\le \kappa  \rho^t \cdot \sup_{\xi \in \Xi}\| \sh_0(\xi)\|.
	\end{align*}
\end{proof}

\begin{proof}[Proof of Lemma~\ref{lem:poisson}]
	Define 
	\[
	\sU(\x, \xi) := \sum_{t=0}^\infty \left(  \PM^t  \sH(\x, \xi) - \sg(\x) \right).
	\]
	We first claim $\sU(\x, \xi)$ is finite almost surely and thus well-defined.
	When setting $\sh_\x(\xi) = \sH(\x, \xi) - \sg(\x)$, we know that $\PM\sh_\x(\xi)=\PM\sH(\x, \xi) - \sg(\x)$ is bounded by $\sigma_{\x} := 2 L_H \|\x-\x^{\star}\| + \sigma $ uniformly over $\xi \in \Xi$ due to
	\begin{align*}
			\|\PM\sh_\x(\xi)\| 
			&\le \PM\| \sh_\x(\xi)-\sh_{\x^{\star}}(\xi)\| + \|\PM\sh_{\x^{\star}}(\xi)\|\\
			&\le \PM\|\sH(\x, \xi) -\sH(\x^{\star}, \xi)\| + \sg(\x) + \|\PM\sh_{\x^{\star}}(\xi)\|\\
			&\le 2 L_H \|\x-\x^{\star}\| + \sigma = \sigma_{\x}
	\end{align*}
where the last inequality uses Assumption~\ref{asmp:H} and Assumption~\ref{asmp:markov-noise}.
	Therefore, under Assumption~\ref{asmp:markov-noise}, we have $\EB_{\xi \sim \DM} \sh_\x(\xi) = 0$ and $\| \PM^t \sH(\x, \xi) - \sg(\x) \| \le \kappa  \rho^{t-1} \sigma_{\x}$ from Lemma~\ref{lem:geo-con}.
	As a result, we have
	\begin{align*}
		\|\sU(\x, \xi) \|  
		&\le \| \sH(\x, \xi) - \sg(\x) \|+ \sum_{t=1}^\infty \| \PM^t  \sH(\x, \xi) - \sg(\x) \|
		\\
		&\le\| \sH(\x, \xi) - \sg(\x) \| + \kappa \sum_{t=0}^\infty \rho^t \sigma_{\x}  \\
		&\le \| \sH(\x, \xi) - \sg(\x) \| +  \frac{\kappa\sigma_{\x}}{1-\rho} < \infty.
	\end{align*}
	Similarly, we can show 
	\[
	\|\PM\sU(\x, \xi) \|  
	\le \sum_{t=1}^\infty \| \PM^t  \sH(\x, \xi) - \sg(\x) \|
	\le \frac{\kappa\sigma_{\x}}{1-\rho} \le  \kappa \sigma_{\x} \tmix,
	\]
	which completes the proof for the second item.
	We then show $\sU(\x, \xi)$ is indeed a solution to~\eqref{eq:poisson} because
	\begin{align*}
		\sU(\x, \xi) - \PM\sU(\x, \xi)  
		&= \sum_{t=0}^\infty \left(  \PM^t  \sH(\x, \xi) - \sg(\x) \right) - \PM \sum_{t=0}^\infty \left(  \PM^t  \sH(\x, \xi) - \sg(\x) \right)\\
		&=\sum_{t=0}^\infty \left(  \PM^t  \sH(\x, \xi) - \sg(\x) \right) -  \sum_{t=1}^\infty \left(  \PM^t  \sH(\x, \xi) - \sg(\x) \right)\\
		&=\sH(\x, \xi) - \sg(\x).
	\end{align*}
	It is also clear that $\EB_{\xi \sim \pi} \sU(\x, \xi)=\0$ since $\pi$ is the stationary distribution of $\PM$ and the equation~\eqref{eq:g-form}.
	If there exists another solution $\sU'(\x, \xi)$ to the same equation~\eqref{eq:poisson} and satisfying $\EB_{\xi \sim \pi} \sU'(\x, \xi) = \0$ for any $\x \in \RB^d$, then there exists a function $c(\x)$ such that $ \sU'(\x, \xi) = \sU(\x, \xi) + c(\x)$ from Proposition 1.1 of~\citet{glynn1996liapounov}.
	As a result, we have $c(\x) = \0$ for any $\x \in \RB^d$, which implies the uniqueness of $\sU(\x, \xi)$.

	Finally, for any $\x, \y \in \RB^d$ and $\xi \in \Xi$, by Lemma~\ref{lem:geo-con},
	\begin{align*}
		\| \sU(\x, \xi) - \sU(\y, \xi) \|
		&= \left\|   \sum_{t=0}^\infty \left[  \PM^t \left(  \sH(\x, \xi) - \sH(\y, \xi)   \right)
		- \left( \sg(\x) -\sg(\y)  \right)
		\right]
		\right\|\\
		&\le \left\| \left(  \sH(\x, \xi) - \sH(\y, \xi)   \right)
		- \left( \sg(\x) -\sg(\y)  \right) \right\|\\
		&\qquad + \sum_{t=1}^\infty  \left\|  \PM^t \left(  \sH(\x, \xi) - \sH(\y, \xi)   \right)
		- \left( \sg(\x) -\sg(\y)  \right) \right\|\\
		&\le  \left\| \sH(\x, \xi) - \sH(\y, \xi) \right\|
		+ \left\| \sg(\x) -\sg(\y) \right\|\\
		& \qquad + 
		\frac{\kappa}{1-\rho} \sup_{\xi \in \Xi} \left\|\PM\left(  \sH(\x, \xi) - \sH(\y, \xi)   \right)-\left( \sg(\x) -\sg(\y)  \right) \right\|
		% 		&\le  2L_H\frac{1-\rho+\kappa}{1-\rho} \cdot \|\x -\y\|
	\end{align*}
	By Jensen's inequality, it follows that for the $p$ defined in Assumption~\ref{asmp:noise},
	\begin{align*}
		\| \sU(\x, \xi) - \sU(\y, \xi) \|^{\udp}
		&\le 3^{\udp-1}  \left\|  \sH(\x, \xi) - \sH(\y, \xi) \right\|^{\udp}   + 3^{\udp-1}  \left\| \sg(\x) -\sg(\y) \right\|^{\udp} \\
		& \qquad + 
		\frac{3^{\udp-1}\kappa^{\udp}}{(1-\rho)^{\udp}} \sup_{\xi \in \Xi} \left\|\PM\left(  \sH(\x, \xi) - \sH(\y, \xi)   \right)-\left( \sg(\x) -\sg(\y)  \right) \right\|^{\udp}\\
		&\le 3^{\udp-1}  \left\|  \sH(\x, \xi) - \sH(\y, \xi) \right\|^{\udp}   + \left( 3^{\udp-1} +\frac{6^{\udp-1}\kappa^{\udp}}{(1-\rho)^{\udp}} \right) \cdot \left\| \sg(\x) -\sg(\y) \right\|^{\udp} \\
		& \qquad + 
		\frac{6^{\udp-1}\kappa^{\udp}}{(1-\rho)^{\udp}} \sup_{\xi \in \Xi} \left\|\PM  \sH(\x, \xi) - \PM\sH(\y, \xi) \right\|^{\udp}.
		% 		&\le  2L_H\frac{1-\rho+\kappa}{1-\rho} \cdot \|\x -\y\|
	\end{align*}
	By Assumption~\ref{asmp:H}, it follows that $\PM\left\|  \sH(\x, \xi) - \sH(\y, \xi) \right\|^{\udp}   \le L_H^{p} \|\x-\y\|^{\udp} $ uniformly for $\xi \in \Xi$.
	Notice that have that $\EB_{\xi \sim \pi} \PM(\cdot) = \EB_{\xi \sim \pi}(\cdot)$ because $\pi$ is the (unique) stationary distribution of $\PM$.
	Therefore, by conditional Jensen's inequality,
	\begin{align*}
		\left\| \sg(\x) -\sg(\y) \right\|^{\udp}
		&= \left\|\EB_{\xi \sim \pi} \PM \left( \sH(\x, \xi) - \sH(\y, \xi) \right) \right\|^{\udp} \\
		&\le \EB_{\xi \sim \pi} \PM \left\|  \sH(\x, \xi) - \sH(\y, \xi) \right\|^{\udp}  \le L_H^{\udp} \|\x-\y\|^{\udp}.
	\end{align*}
	Similarly, we also have that
	\[
	\sup_{\xi \in \Xi} \left\|\PM \sH(\x, \xi) -\PM \sH(\y, \xi) \right\|^{\udp}
	\le 	\sup_{\xi \in \Xi} \PM \left\| \sH(\x, \xi) -\sH(\y, \xi) \right\|^{\udp} \le  L_H^{\udp} \|\x-\y\|^{\udp}.
	\]
	Putting the pieces together, we conclude that there exists a constant $L_U = \OM(L_H(1 + \kappa \tmix))$ such that
	\[
	\PM\| \sU(\x, \xi) - \sU(\y, \xi) \|^{\udp} \le L_U^{\udp} \|\x-\y\|^{\udp}.
	\]
	
\end{proof}

\subsection{Proof of Lemma~\ref{lem:error-analysis}}
\label{proof:error-analysis}
\begin{proof}[Proof of Lemma~\ref{lem:error-analysis}]
	In the following, we use $a \precsim b$ to denote $a \le C b$ for an unimportant positive constant $C > 0$ that doesn't depends on $p$ for simplicity.
	 Let $C_{U, \x_t} =  \kappa \tmix \cdot (2L_H \|\x_t-\x^{\star}\|+\sigma)$.
	By~\ref{lem:U-bounded} in Lemma~\ref{lem:poisson}, we have $\| \PM \sU(\x_t, \xi_{t-1})\| \le C_{U, \x_t}$.
	\begin{enumerate}[(i)]
		\item
		By Assumption~\ref{asmp:nonlinear}, it implies that
		\begin{align*}
			\| \sr_t\| &= \|\sg(\x_t) - \sG \De_t\|\\
			&\le \|\sg(\x_t) - \sG (\x_t -\x^{\star})\| + \eta_t \| \PM \sU(\x_t, \xi_{t-1})\|\\
			&\le 
			\left\{ \begin{array}{ll}
				L_G \cdot\|\x_t -\x^{\star}\|^2 + \eta_t C_{U, \x_t}&  \text{if} \ \|\x_t -\x^{\star}\| \le \delta_G\\
				(L_H +  \| \sG\|  )\cdot \| \x_t -\x^{\star}\| + \eta_t C_{U, \x_t}& \text{if} \ \|\x_t -\x^{\star}\| \ge \delta_G
			\end{array}
			\right.\\
			&\le \max\left\{L_G , \frac{L_H +  \| \sG\|}{\delta_G}\right\}\|  \x_t -\x^{\star}  \|^2 + \eta_t C_{U, \x_t}.
		\end{align*}
		Since $\{\x_t\}_{t \ge 0}$ satisfies the $(L^2, (1+\log t)\sqrt{\eta_t})$-consistency (from Assumption~\ref{asmp:x}), $\EB\|\x_t -\x^{\star}\|^2 \precsim  \eta_t \log t $.
		As a result, when $T \to \infty$,
		\[
		\frac{1}{\sqrt{T}} \sum_{t=0}^T \EB \| \sr_t\|
		\precsim \frac{1}{\sqrt{T}}  \sum_{t=0}^T\EB\|\x_t -\x^{\star}\|^2 + \frac{1}{\sqrt{T}}  \sum_{t=0}^T \eta_t
		\precsim \frac{\log T}{\sqrt{T}}  \sum_{t=0}^T  \eta_t \to 0.
		\]
		
		\item By~\eqref{eq:u}, we have $\EB[\sU(\x_t, \xi_t)|\FM_{t-1}] = \PM \sU(\x_t, \xi_{t-1})$ where $\FM_{t}$ is the $\sigma$-field defined by $\FM_t := \sigma(\{ \xi_\tau \}_{0 \le \tau \le t})$.
		Hence, $\{ \su_t \}_{t \ge 0}$ is a martingale difference sequence.
		By~\ref{lem:U-bounded} in Lemma~\ref{lem:poisson} and Assumption~\ref{asmp:noise}, $\sum_{t=1}^{\floor{Tr}} \su_t $ is square integrable for all $r \in [0, 1]$.
		By~\eqref{eq:u}, we decompose $\su_t$ into two parts  
		$\su_t = \su_{t,1} + \su_{t,2}$ where
		\begin{align}
			\begin{split}
				\label{eq:U-12}
				\su_{t, 1} &=  \left[  \sU(\x_t, \xi_t) - \PM \sU(\x_t, \xi_{t-1}) \right] - \left[  \sU(\x^{\star}, \xi_t) - \PM \sU(\x^{\star}, \xi_{t-1}) \right],\\
				\su_{t, 2}&=  \left[  \sU(\x^{\star}, \xi_t) - \PM \sU(\x^{\star}, \xi_{t-1}) \right].
			\end{split}
		\end{align}
		It's clear that both $\{ \su_{t,1} \}_{t \ge 0}$ and $\{ \su_{t,2} \}_{t \ge 0}$ are also martingale difference sequences.
		We assert that $\frac{1}{\sqrt{T}} \sum_{t=1}^{\floor{Tr}} \su_t$ has the same asymptotic behavior as $\frac{1}{\sqrt{T}} \sum_{t=1}^{\floor{Tr}} \su_{t,2}$ due to
		\[
		\EB \sup_{r \in [0, 1]} \left\|\frac{1}{\sqrt{T}} \sum_{t=1}^{\floor{Tr}} \su_t- \frac{1}{\sqrt{T}} \sum_{t=1}^{\floor{Tr}} \su_{t,2} \right\|^2=
		\EB \sup_{r \in [0, 1]} \left\|\frac{1}{\sqrt{T}} \sum_{t=1}^{\floor{Tr}} \su_{t,1} \right\|^2= o(1).
		\]
		This is because from Doob's martingale inequality,
		\[
		\EB \sup_{r \in [0, 1]} \left\|\frac{1}{\sqrt{T}} \sum_{t=1}^{\floor{Tr}} \su_{t,1} \right\|^2
		\le \frac{1}{T} \sum_{t=0}^T\EB\|\su_{t,1}\|^2
		\precsim \frac{\log T}{T} \sum_{t=0}^T \eta_t \to 0,
		\]
		where the last inequality uses the following result
		\begin{align*}
			\EB\|\su_{t,1}\|^2
			&\le 2 \EB \| \sU(\x_t, \xi_t)-\sU(\x^{\star}, \xi_t)\|^2
			+2 \EB \|\PM \sU(\x_t, \xi_{t-1})- \PM \sU(\x^{\star}, \xi_{t-1})\|^2\\
			&= 2 \EB \PM \| \sU(\x_t, \xi_{t-1})-\sU(\x^{\star}, \xi_{t-1})\|^2+
			2 \EB \|\PM \sU(\x_t, \xi_{t-1})- \PM \sU(\x^{\star}, \xi_{t-1})\|^2\\
			&\overset{(a)}{\le}  4\EB \PM \| \sU(\x_t, \xi_{t-1})-\sU(\x^{\star}, \xi_{t-1})\|^2 \\
			&\overset{(b)}{\le}  4\EB (\PM \| \sU(\x_t, \xi_{t-1})-\sU(\x^{\star}, \xi_{t-1})\|^\udp)^{\frac{2}{\udp}}
			\overset{(c)}{\le} 4 L_U^2 \cdot \EB\|\x_t - \x^{\star}\|^2 	\overset{(d)}{\precsim} \eta_t \cdot \log t .
		\end{align*}
		Here $(a)$ follows from conditional Jensen's inequality, $(b)$ follows from conditional Holder's inequality, $(c)$ uses ~\ref{lem:U-continous} in Lemma~\ref{lem:poisson}, and $(d)$ uses $\EB\|\x_t-\x^{\star}\|^2 \precsim \eta_t \cdot \log t $ from Assumption~\ref{asmp:x}.
		
		We then focus on the partial-sum process $\frac{1}{\sqrt{T}} \sum_{t=1}^{\floor{Tr}} \su_{t,2}$.
		For one thing, by Assumption~\ref{asmp:noise}, $\{\su_{t,2}\}_{t\ge 0}$ has uniformly bounded $p > 2$ moments, which is because
		\[
		\sup_{t \ge 0}\EB\|\su_{t,2}\|^p \le 2^{p-1}\sup_{t \ge 0} \left[ \EB\| \sU(\x^{\star}, \xi_t)\|^p  + \EB\|\PM\sU(\x^{\star}, \xi_{t-1})\|^p \right] < \infty.
		\]
		As a result, for any $\eps > 0$, as $T$ goes to infinity,
		\begin{align*}
			\EB \left\{
			\sum_{t=0}^{T} \EB\left[  \left\| \frac{\su_{t,2}}{\sqrt{T}} \right\|^2 \mathds{1}_{\{\|\su_{t,2}\| \ge \sqrt{T}\eps \} }\bigg| \FM_{t-1}  \right]\right\}
			&\le \frac{1}{\eps^{\frac{p}{2}-1}T^\frac{p}{2}}	\EB \left\{\sum_{t=0}^{T} \EB\left[  \left\| \su_{t,2}\right\|^p \bigg| \FM_{t-1}  \right] \right\} \\
			&\le \frac{\sup_{t \ge 0}\EB\|\su_{t,2}\|^p}{\eps^{\frac{p}{2}-1}T^{\frac{p}{2}-1}}   \to 0,
		\end{align*}
		which implies
		\[
		\sum_{t=0}^{T} \EB\left[  \left\| \frac{\su_{t,2}}{\sqrt{T}} \right\|^2 \mathds{1}_{\{\|\su_{t,2}\| \ge \sqrt{T}\eps \} }\bigg| \FM_{t-1}  \right] \overset{p}{\to} 0.
		\]
		% 	\begin{align*}
			% 		\EB\|\EB[\su_{t, 1}\su_{t, 1}^\top|\FM_{t-1}] \|
			% 	\le\EB\|\su_{t, 1}\su_{t, 1}^\top \| = \EB\|\su_{t, 1}\|^2 \le 4 L_U^2 \EB\|\x_t -\x^{\star}\|^2 \precsim \eta_t \to 0
			% 	\end{align*}
		% which implies $\EB[\su_{t, 1}\su_{t, 1}^\top|\FM_{t-1}] = o_{\PB}(1)$ and $\EB[\|\su_{t, 1}\|^2|\FM_{t-1}] = o_{\PB}(1)$.
		% By the same argument, we have $\EB[\|\su_{t, 2}\|^2|\FM_{t-1}] = O_{\PB}(1)$. 
		% As a result,
		% \[
		% \|\EB[\su_{t, 1}\su_{t, 2}^\top|\FM_{t-1}] \|^2 
		% \le \EB[\|\su_{t, 1}\su_{t, 2}^\top\||\FM_{t-1}]^2
		% \le \EB[\|\su_{t, 1}\|^2|\FM_{t-1}]  \cdot \EB[\|\su_{t, 2}\|^2|\FM_{t-1}] 
		% = o_{\PB}(1)
		% \]
		% where the last inequality uses Cauchy-Schwarz inequality for conditional expectations.
		For another thing, we notice that
		\begin{align*}
			&\EB \left[  \left[  \sU(\x^{\star}, \xi_t) - \PM \sU(\x^{\star}, \xi_{t-1}) \right]  \left[  \sU(\x^{\star}, \xi_t) - \PM \sU(\x^{\star}, \xi_{t-1}) \right]^\top \bigg|\FM_{t-1}   \right]\\
			=& \EB \left[\sU(\x^{\star}, \xi_t)\sU(\x^{\star}, \xi_t)^\top \bigg|\FM_{t-1}   \right] -  \PM \sU(\x^{\star}, \xi_{t-1}) \PM \sU(\x^{\star}, \xi_{t-1})^\top \\
			=& \PM \sU(\x^{\star}, \xi_{t-1})\sU(\x^{\star}, \xi_{t-1})^\top -  \PM \sU(\x^{\star}, \xi_{t-1}) \PM \sU(\x^{\star}, \xi_{t-1})^\top
		\end{align*}
		which together with Birkhoff's ergodic theorem (Theorem 7.2.1 in~\citet{durrett2013probability}) implies
		\begin{align*}
			\frac{1}{T} &\sum_{t=1}^T \left[ \PM \sU(\x^{\star}, \xi_{t-1})\sU(\x^{\star}, \xi_{t-1})^\top -  \PM \sU(\x^{\star}, \xi_{t-1}) \PM \sU(\x^{\star}, \xi_{t-1})^\top\right]
			\\
			& \overset{p}{\to} \sS = \EB_{\xi \sim \pi} \left[ \PM \sU(\x^{\star}, \xi)\sU(\x^{\star}, \xi)^\top -  \PM \sU(\x^{\star}, \xi) \PM \sU(\x^{\star}, \xi)^\top\right].
		\end{align*}
		Because $\int_{\Xi} \PM(\xi,  \xi') \pi(d\xi)= \pi(\xi')$ by the definition of the stationary distribution $\pi$, we have 
		\[
		\EB_{\xi \sim \pi}  \PM \sU(\x^{\star}, \xi)\sU(\x^{\star}, \xi)^\top
		= \EB_{\xi \sim \pi} \sU(\x^{\star}, \xi)\sU(\x^{\star}, \xi)^\top
		\]
		Hence, we have
		\[
		\frac{1}{T} \sum_{t=1}^T \EB[\su_{t, 2}\su_{t, 2}^\top|\FM_{t-1}] \overset{p}{\to} \sS = \EB_{\xi \sim \pi} \left[ \sU(\x^{\star}, \xi)\sU(\x^{\star}, \xi)^\top -  \PM \sU(\x^{\star}, \xi) \PM \sU(\x^{\star}, \xi)^\top\right].
		\]
		Hereto, we have shown $\{\su_{t,2}\}_{t \ge 0}$ satisfies the Lindeberg-Feller conditions for martingale central limit theorem.
		Then the martingale FCLT follows from Theorem 4.2 in~\citet{hall2014martingale} (or Theorem 8.8.8 in~\citet{durrett2013probability}, or Theorem 2.1 in~\citet{whitt2007proofs}).
		Therefore, we have
		\[
		\frac{1}{\sqrt{T}} \sum_{t=1}^{\floor{Tr}} \su_{t,2} \overset{w}{\to} \sS^{1/2} \sW(r)
		\ \text{and} \ 		\frac{1}{\sqrt{T}} \sum_{t=1}^{\floor{Tr}} \su_{t} \overset{w}{\to} \sS^{1/2} \sW(r).
		\]

		Finally, by~\ref{lem:U-continous} in Lemma~\ref{lem:poisson} and conditional Jensen's inequality, we have
		\begin{align*}
			\EB\|\su_{t, 1}\|^\udp
			&\le 2^{\udp-1} \left[ \EB \| \sU(\x_t, \xi_t)-\sU(\x^{\star}, \xi_t)\|^\udp
			+2 \EB \|\PM \sU(\x_t, \xi_{t-1})- \PM \sU(\x^{\star}, \xi_{t-1})\|^\udp \right]\\
			&\le 2^\udp  \EB \| \sU(\x_t, \xi_t)-\sU(\x^{\star}, \xi_t)\|^\udp
			\le 2^\udp L_U^\udp \EB \| \x_t-\x^{\star}\|^\udp.
		\end{align*}
		As a result, we have $\sup_{t\ge 0}\EB \|\su_{t, 1}\|^\udp
		\precsim \sup_{t\ge 0} \EB \|\x_t-\x^{\star}\|^\udp < \infty$ from Assumption~\ref{asmp:x}.
		% On the other hand, notice that $\sup_{t \ge 0}(\EB \|\su_{t,2}\|^\udp)^{\frac{1}{\udp}} \le \sup_{t \ge 0}(\EB \|\su_{t,2}\|^p)^{\frac{1}{p}} < \infty$ due to  $\udp \le p$.
		Therefore,
		$\sup_{t\ge 0}\EB \|\su_{t}\|^\udp \le 2^{\udp-1}(\sup_{t\ge 0}\EB \|\su_{t,1}\|^\udp+\sup_{t\ge 0}\EB \|\su_{t,2}\|^\udp) < \infty$.
		By now, we complete the proof of this part.

		\item By~\eqref{eq:nu} and~\ref{lem:U-continous} in Lemma~\ref{lem:poisson}, we have 
		\begin{align}
			\label{eq:help-nu-0}
			\|\snu_t\| &= \left\| \frac{\eta_{t+1}}{\eta_t} \PM\sU(\x_{t+1}, \xi_t) - \PM \sU(\x_t, \xi_{t})\right\| \nonumber \\
			&\le  \left\|  \PM\sU(\x_{t+1}, \xi_t) - \PM \sU(\x_t, \xi_{t})\right\|
			+ \left\| \frac{\eta_{t+1}-\eta_t}{\eta_t} \PM\sU(\x_{t+1}, \xi_t) \right\| \nonumber \\
			&\le L_U \|\x_{t+1} - \x_t\| + \left| \frac{\eta_{t+1}-\eta_t}{\eta_t} \right| \cdot C_{U, \x_{t+1}}   \\
			& \precsim L_U \|\x_{t+1} - \x_t\| + o(\eta_t) \cdot \left( \|\x_{t+1}-\x^{\star}\| + \sigma  \right)\nonumber.
		\end{align} 
		From another hand, it follows that
		\begin{align*}
			\EB\|\x_{t+1} - \x_t\|  
			&\le \eta_t   \EB\| \sH(\x_t, \xi_t) \|
			\overset{(a)}{\le} \eta_t   \left[ \EB\| \sH(\x^{\star}, \xi_t) \| + L_H\|\x_t -\x^{\star}\|  \right]\\
			&\le \eta_t  \left[ L_H\EB\| \x_t -\x^{\star}\| + \sup_{t \ge 0}\EB\| \sH(\x^{\star}, \xi_t) \|\right]
			\overset{(b)}{\precsim} \eta_t
		\end{align*}
		where $(a)$ uses the following result (which mainly follows from Assumption~\ref{asmp:H}),
		\begin{align*}
			\EB\| \sH(\x_t, \xi_t) - \sH(\x^{\star}, \xi_t) \|
			&=\EB \PM \| \sH(\x_t, \xi_{t-1}) - \sH(\x^{\star}, \xi_{t-1}) \|\\
			&\le\EB (\PM \| \sH(\x_t, \xi_{t-1}) - \sH(\x^{\star}, \xi_{t-1}) \|^p)^{\frac{1}{p}}\\
			&\le L_H \EB\|\x_t -\x^{\star}\|
		\end{align*}
		and $(b)$ uses the following two inequalities, $\sup_{t \ge 0} \EB \|\sH(\x^{\star}, \xi_t) \| \le \sup_{t \ge 0}  (\EB \|\sH(\x^{\star}, \xi_t) \|^p)^{1/p} \precsim 1$ and $\EB\| \x_t -\x^{\star}\| \le \sup_{t \ge 0} \sqrt[p]{\EB\| \x_t -\x^{\star}\|^p} \precsim 1$.
		Finally, we have
		\[
		\EB\|\snu_t\| \precsim \eta_t
		\implies
		\frac{1}{\sqrt{T}} \sum_{t=0}^T \EB \| \snu_t\|
		\precsim \frac{1}{\sqrt{T}}  \sum_{t=0}^T \eta_t \to 0
		\ \text{as} \ T \to \infty.
		\]

	\end{enumerate}
\end{proof}

\subsection{Proof of Lemma~\ref{lem:residual-terms}}
\label{proof:residual-terms}
\begin{proof}[Proof of Lemma~\ref{lem:residual-terms}]
	We analyze the four separate terms $\sup_{r \in [0, 1]} \|\Bpsi_k(r)\|(0 \le k \le 3)$ respectively.
	\paragraph{For the partial-sum process of noises}
By~\ref{lem:error-u} in Lemma~\ref{lem:error-analysis}, it follows that
\[
\frac{1}{\sqrt{T}} \sum_{t=1}^{\floor{Tr}} \su_t \overset{w}{\to} \sS^{1/2} \sW(r).
\]	

\paragraph{For $\Bpsi_0$}
\ref{lem:vanish-A} in Lemma~\ref{lem:A} shows $\sA_{j}^n$ is uniformly bounded.
As $T \to \infty$,
\[
\sup_{r \in [0, 1]} \|\Bpsi_0(r)\| = 
\frac{1}{\sqrt{T} \eta_0} \sup_{r \in [0, 1]} \|\sA_0^{\floor{Tr}} \sB_0\De_0\| \le  \frac{C_0}{\sqrt{T} \eta_0}\|\sB_0\De_0\| \to 0.
\]

\paragraph{For $\Bpsi_1$}
Recall that 
$\Bpsi_1(r) = \frac{1}{\sqrt{T}} \sum_{t=0}^{\floor{Tr}} \sA_t^{\floor{Tr}} (\sr_t + \snu_t)$.
Since $\|\sA_j^n\| \le C_0$ for any $n \ge j \ge 0$, it follows that as $T \to \infty$,
\[
\EB \sup_{r \in [0, 1]} \|\Bpsi_1(r)\|  \le \frac{C_0}{\sqrt{T}} \EB \sum_{t=0}^T \left( \|\sr_t\| + \|\snu_t\| \right) \to 0
\]
where the last inequality uses~\ref{lem:error-r} and~\ref{lem:error-nu} in Lemma~\ref{lem:error-analysis}.

\paragraph{For $\Bpsi_2$}
Recall that $\Bpsi_2(r) = \frac{1}{\sqrt{T}} \sum_{t=0}^{\floor{Tr}} \left(\sA_t^T -\sG^{-1}\right)\su_t$ with $\su_t$ a martingale difference.	
In the following, we set $\sz_t = \Bpsi_2(t/T)$ (indexed by $t \in [T]$) for simplicity.
It is clear that $\{\sz_t, \FM_t \}_{t \in [T]}$ forms a square integrable martingale difference sequence.
As a result $\{ \|\sz_t\|_2, \FM_t \}_{t \in [T]}$ is a submartingale due to $\EB[\|\su_t\|_2|\FM_{t-1}] \ge \|\EB[\su_t|\FM_{t-1}] \|_2 = \|\su_{t-1}\|_2$ from conditional Jensen's inequality.
By Doob’s maximum inequality for submartingales (which we use to derive the following $(*)$ inequality), 
\begin{align*}
	\EB\sup_{r \in [0, 1]} \|\Bpsi_{2}(r)\|_2^2
	&=\EB \sup_{t \in [T]} \|\sz_t\|_2^2 
	\overset{(*)}{\le} 4 \EB\|\sz_T\|_2^2\\
	&= \frac{4}{T} \sum_{t=0}^T \EB\|\left(\sA_t^T -\sG^{-1}\right)\su_t\|_2^2 \\
	&\le  4\sup_{t \ge 0} \EB\|\su_t\|_2^2 \cdot  \frac{1}{T} \sum_{t=0}^T\|\sA_t^T -\sG^{-1}\|_2^2 \to 0
\end{align*}
where we use~\ref{lem:vanish-A} in Lemma~\ref{lem:A} and the fact $\|\sA_t^T -\sG^{-1}\|$ is uniformly bounded by $C_0 + \|\sG^{-1}\|$.
Due to the norm equivalence in $\RB^d$, $\|\cdot\|$ is equivalent to $\|\cdot\|_2$ up to universal constants.

\paragraph{For $\Bpsi_3$}
Recall that $\Bpsi_3(r) = \frac{1}{\sqrt{T}} \sum_{t=0}^{\floor{Tr}} \left(\sA_t^{\floor{Tr}} -\sA_t^{T}\right)\su_t$ with $\su_t$ a martingale difference.	
Notice that for any $n \in [T]$
\begin{equation}\label{eq:bpsi_3}
	\begin{aligned}
		\sum_{t=0}^{n}(\sA_t^T- \sA_t^{n} )\su_t
		&= \sum_{t=0}^{n} \sum_{j=n+1}^T \left(\prod_{i=t+1}^j \sB_i\right)\eta_t \su_t
		= \sum_{j=n+1}^{T} \sum_{t=0}^n \left(\prod_{i=t+1}^j \sB_i\right)\eta_t \su_t\\
		&=\sum_{j=n+1}^{T}  \left(\prod_{i=n+1}^j \sB_i\right)\sum_{t=1}^n \left(\prod_{i=t+1}^n \sB_i\right)
		\eta_t \su_t\\
		&=\frac{1}{\eta_{n+1}}\sA_{n+1}^T\sB_{n+1}\sum_{t=0}^n \left(\prod_{i=t+1}^n \sB_i\right)
		\eta_t \su_t.
	\end{aligned}
\end{equation}
From~\ref{lem:vanish-A} in Lemma~\ref{lem:A}, $\|\sA_{n+1}^T\sB_{n+1}\| \le C_0(1+\| \sG\|)$ for any  $T \ge n \ge 0$.
Hence,
\begin{align}
	\tag{\ref{eq:bpsi_30}}
	\sup_{r \in [0, 1]}\| \Bpsi_3(r)\|
	&= \sup_{n \in [T]} \left\|  \frac{1}{\sqrt{T}} \sum_{t=0}^{n} \left(\sA_t^{n} -\sA_t^{T}\right)\su_t \right\|\nonumber \\
	&\precsim \sup_{n \in [T]} \left\|  \frac{1}{\sqrt{T}}
	\frac{1}{\eta_{n+1}}\sum_{t=0}^n \left(\prod_{i=t+1}^n \sB_i\right)
	\eta_t \su_t \right\| = o_{\PB}(1)
\end{align}
where the last inequality uses Lemma~\ref{lem:error}.
We then complete the proof.
\end{proof}

\subsection{Proof of Lemma~\ref{lem:error}}
\label{proof:error}
For the proof in the part, we will consider random variables (or matrices) in the complex field $\mathbb{C}$.
Hence, we will introduce new notations for them.
For a vector $\sv \in \mathbb{C}$ (or a matrix $\sU \in \mathbb{C}^{d \times d}$), we use $\sv^\mthH$ (or $\sU^\mthH$) to denote its Hermitian transpose or conjugate transpose.
For any two vectors $\sv, \su \in \mathbb{C}$, with a slight abuse of notation, we use $\langle\sv, \su\rangle = \sv^\mthH \su$ to denote the inner product in $\mathbb{C}$.
For simplicity, for a complex matrix $\sU \in \mathbb{C}^{d \times d}$, we use $\|\sU\|$ to denote the its operator norm introduced by the complex inner product $\langle \cdot, \cdot \rangle$.
When $\sU \in\RB^{d \times d}$, $\|\sU\|$ is reduced to the spectrum norm.

\begin{proof}[Proof of Lemma~\ref{lem:error}]
	We provide the proof only for the asymptotic result; for the weak convergence rate see Lemma~\ref{lem:error1} and its proof.
	To simplify notation, we say a random sequence $\{\y_t\}_{t \ge 0}$ is \textit{uniformly ignorable} if $\frac{1}{\sqrt{T}}\sup\limits_{t\in[0,T]}\frac{\|\y_{t+1}\|}{\eta_{t+1}}\overset{p}{\to}0$ when $T\to \infty$.
	Our target is equivalent to show the defined $\{\y_t\}_{t \ge 0}$ is uniformly ignorable.
	
	We are going to prove the lemma in two steps.
	In the first step, we prove a weaker version in Lemma~\ref{lem:error0} under an additional assumption that requires $\sG$ is diagonalizable.
	The proof of Lemma~\ref{lem:error0} is deferred in Section~\ref{proof:error0}.
	Then, in the second step, we remove the added assumption via a refined analysis that relies on induction to reduce the general Hurwitz case to the established diagonalizable case by using the Jordan decomposition of $\sG$.
	
	\begin{lem}
		\label{lem:error0}
		Under the same condition of Lemma~\ref{lem:error}, if we additionally assume $\sG$ is diagonalizable, then
		\[
		\frac{1}{\sqrt{T}} \sup_{0 \le t \le T} \frac{\|\y_{t+1}\|}{\eta_{t+1}} \overset{p}{
			\to} 0.
		\]
	\end{lem}
	
	Lemma~\ref{lem:srgt_unf_op} serves a bridge to connect the general Hurwitz case with the diagonalizable case.
	Its proof is provided in Section~\ref{proof:srgt_unf_op}.
	\begin{lem}
		\label{lem:srgt_unf_op}
		Let $\{\eta_t\}_{t \ge 0}$ be the step size satisfying Assumption~\ref{asmp:eta} and $\lambda \in \mathbb{C}$ be a complex number with positive real part $\mathrm{Re}(\lambda) > 0$.
		Let $\{\omega_t\}_{t \ge 0} \subseteq \mathbb{C}$ be
		a sequence of random variables taking value in the complex field and $\frac{1}{\sqrt{T}}\sup\limits_{t\in [0,T]}\frac{|\omega_t|}{\eta_{t}}\overset{p}{\to} 0$ as $T\to \infty$.
		Consider the sequence $\{z_t\}_{t\ge0}$ defined recursively as following: $z_0 = 0$ and
		\[
		z_{t+1} = z_t -\lambda\eta_t z_t + \eta_t \omega_t.
		\]
		Then when $T\to \infty$, we have $\{z_t\}_{t\ge0}$ is also uniformly ignorable, i.e.,
		\[
		\frac{1}{\sqrt{T}}\sup\limits_{0 \le t \le T}\frac{|z_{t+1}|}{\eta_{t+1}} \overset{p}{\to}0.
		\]
	\end{lem}

	By viewing $\sG \in \RB^{d \times d}$ as a complex matrix, it has the Jordan decomposition with the Jordan canonical form denoted by $\sG = \sV\sJ\sV^{-1} = \sV\diag\{\sJ_1,\cdots,\sJ_r\}\sV^{-1}$, where $\sV$ is the non-singular matrix and $\{ \sJ_i\}_{1\le i \le r}$ collects all Jordan blocks.
	% It is well known that $\mathrm{Poly}(\sG) = \sV^{\star}\mathrm{Poly}(\sJ)\sV$ for any polynomial function $\mathrm{Poly}(\cdot)$. 
	Recall that $\{\y_t\}_{t \ge 0}$ is defined in~\eqref{eq:y}.
	Let $\widetilde{\y}_t = \sV^{-1}\y_t$, $\widetilde{\seps}_t = \sV^{-1}\seps_t$ be transformed vectors. 
	Then the recursion formula~\eqref{eq:y} becomes
	\[
	\widetilde{\y}_{t+1} = (\sI - \eta_t \sJ) \widetilde{\y}_t + \eta_t\widetilde{\seps}_t.
	\]
	Without loss of generality, we assume that $\sJ$ consists of only one Jordan block, i.e.
	\begin{equation}
		\label{eq:J}
		\sJ = \left[\begin{array}{llll}
			\lambda & 1 & & \\
			& \lambda & \ddots & \\
			& & \ddots & 1 \\
			& & & \lambda
		\end{array}\right]
	\end{equation}
	with $\lambda \in \mathbb{C}$ and $\mathrm{Re}(\lambda)>0$.
	
	Let $\left(\widetilde{\y}_t\right)_k$ denote the $k$-th coordinate of the vector $\widetilde{
		\y}_t$ and so does $\left(\widetilde{\seps}_t\right)_k$.
	Then, in order to prove that $\{\widetilde{\y}_t\}_{t \ge 0}$ is uniformly ignorable, we only needs to prove that each of its coordinates $\{\left(\widetilde{\y}_t\right)_k\}_{t \ge 0} (1 \le k\le d)$ is uniformly ignorable.
	Notice that the last coordinate process evolves as $(\widetilde{\y}_{t+1})_d = (1-\eta_t \lambda)(\widetilde{\y}_t)_d + \eta_t (\widetilde{\seps}_{t})_d$.
	Lemma \ref{lem:error0} implies that $\{(\widetilde{\y}_t)_d\}_{t \ge 1}$, as a one-dimensional process, is uniformly ignorable.
	We are going to finish the proof by induction.
	Suppose for the coordinates $k, k+1, \cdots, d$, we already have  $\{(\widetilde{\y}_t)_k\}_{t \ge 0}$ is uniformly ignorable, now we are going to prove $\{(\widetilde{\y}_t)_{k-1}\}_{t \ge 0}$ is also uniformly ignorable.
	
	Using the structure of $\sJ$ in~\eqref{eq:J}, we have
	\begin{align}\label{eq:tl_y_updt}
		(\widetilde{\y}_{t+1})_{k-1} = (1-\lambda\eta_t)(\widetilde{\y}_t)_{k-1} - \eta_t(\widetilde{\y}_t)_k + \eta_t(\widetilde{\seps}_t)_{k-1}.
	\end{align}
	To facilitate analysis, we construct a surrogate sequence $\{(\widehat{\y}_t)_{k-1}\}$ defined by
	\begin{align}\label{eq:ht_y_updt}
		(\widehat{\y}_{t+1})_{k-1} = (1 - \lambda\eta_t)(\widehat{\y}_t)_{k-1} + \eta_t(\widetilde{\seps}_t)_{k-1}.
	\end{align}
	Again, by Lemma \ref{lem:error0}, $\{(\widehat{\y}_t)_{k-1}\}_{t \ge 0}$ is uniformly ignorable.
	Let $\widetilde{\De}_t := (\widetilde{\y}_{t})_{k-1} - (\widehat{\y}_{t})_{k-1}$ be their difference.
	From \eqref{eq:tl_y_updt} $-$ \eqref{eq:ht_y_updt}, it follows that
	\begin{align*}
		\widetilde{\De}_{t+1} =  (1-\lambda\eta_t)\widetilde{\De}_t - \eta_t(\widetilde{\y}_t)_{k}.
	\end{align*}
	Thanks to Lemma \ref{lem:srgt_unf_op} and our hypothesis, $\{\widetilde{\De}_t\}_{t \ge 0}$ is uniformly ignorable.
	Finally, putting the pieces together, we have
	\begin{align*}
		\frac{1}{\sqrt{T}}\sup\limits_{t\in[0,T]}\frac{\left|(\widetilde{\y}_{t+1})_{k-1}\right|}{\eta_{t+1}} 
		&= 
		\frac{1}{\sqrt{T}}\sup\limits_{t\in[0,T]}\frac{\left|(\widehat{\y}_{t+1})_{k-1} + \widetilde{\De}_{t+1}\right|}{\eta_{t+1}} \\
		&\le  \frac{1}{\sqrt{T}}\sup\limits_{t\in[0,T]}\frac{\left|(\widehat{\y}_{t+1})_{k-1}\right|}{\eta_{t+1}}
		+ \frac{1}{\sqrt{T}}\sup\limits_{t\in[0,T]}\frac{\left|\widetilde{\De}_{t+1}\right|}{\eta_{t+1}}
		\overset{p}{\longrightarrow}0.
	\end{align*}
\end{proof}

\subsection{Proof of Lemma~\ref{lem:error0}}
\label{proof:error0}
\begin{proof}[Proof of Lemma~\ref{lem:error0}]	

	The proof is divided into three steps.
	\paragraph{Step one: Divide the time interval}
	Given a positive integer $n$, we separate the time interval $[0, T]$ uniformly into $n$ portions with $h_k=\left[\frac{k}{n}(T+1)\right] (k=0,1,\dots, n)$ the $k$-th endpoint.
	The choice of $n$ is independent of $T$, which implies that $\lim_{T \to \infty} h_k = \infty$ for any $k\ge 1$.
	Let $c_0' := c_0 \exp(c\eta_0)$ with the constants $c, c_0$ defined in~\ref{lem:bounded-X} in Lemma~\ref{lem:A}.
	For any $\eps >0$,  we define an event $\mathcal{A}$ whose complement is 
	\begin{equation}
		\label{eq:setA}
		\mathcal{A}^c
		:= \left\{ 
		\exists 0 \le k \le n \text{ s.t. } \frac{c_0'}{\sqrt{T}}\left\| \frac{\y_{h_k}}{\eta_{h_k}} \right\| \ge  \eps \right\}.
	\end{equation}
	We claim that $\limsup\limits_{T \to \infty} \PB(\AM^c) = 0$.
	For one thing,	\begin{align}
		\label{eq:bound-y}
		\begin{split}
			\EB\|\y_{t+1}\|^2 
			&= \EB\left\|   \sum_{j=0}^t \left(\prod\limits_{i=j+1}^{t}\left( \sI - \eta_i\sG \right)\right) \eta_j  \seps_j\right\|^2
			= \sum_{j=0}^t \EB\left\|\sX_{j+1}^t\eta_j  \seps_j\right\|^2\\
			&\le \sup_{j \ge 0} \EB\|\varepsi_j\|^2 \cdot \sum_{j=0}^t \eta_j^2 \exp\left( -c \sum_{t=j+1}^t \eta_i \right) \overset{(a)}{\le}  \sup_{j \ge 0} \EB\|\varepsi_j\|^2 \cdot c_1 \eta_{t} \overset{(b)}{\le} c_2\eta_{t}
		\end{split}
	\end{align}
	where $(a)$ follows from~\ref{lem:bounded-norm} in Lemma~\ref{lem:A} and $(b)$ follows by setting $c_2= c_1 \cdot  \sup_{j \ge 0} \EB\|\varepsi_j\|^2$.
	For another thing, by the union bound and Markov's inequality, 
	\begin{align}
		\label{eq:P-A-c}
		\mathbb{P}(\mathcal{A}^c)
		&\le\sum_{k=0}^{n}\PB\left( \frac{c_0'}{\sqrt{T}}\left\| \frac{\y_{h_k}}{\eta_{h_k}} \right\| \ge  \eps \right) 
		\le \frac{(c_0')^2}{T \eps^2} \sum_{k=0}^{n} \EB \left\| \frac{\y_{h_k}}{\eta_{h_k}} \right\|^2
		\overset{(a)}{\le} \frac{c_2(c_0')^2}{T\eps^2} \sum_{k=0}^{n} \frac{1}{\eta_{h_k}}
		\overset{(b)}{\le} \frac{c_2(c_0')^2(n+1)}{\eta_{T}T\eps^2}.
	\end{align}
	Here $(a)$ uses the inequality~\eqref{eq:bound-y} and $(b)$ is because $t\eta_t \to \infty$. 
	So, when $T \to \infty$, $\PB(\AM^c) \to 0$ due to $T \eta_{T} \to \infty$.
	
	Using the notation in Lemma~\ref{lem:A}, we denote $\sX_j^n :=\prod\limits_{i=j}^{n} \left( \sI - \eta_i\sG \right)$.
	Clearly $\sX_j^n$'s are exchangeable since they are polynomials of the same matrix $\sG$.  
	Hence, $\sX_{j+1}^t = (\sX_{t}^T)^{-1} \sX_{j+1}^T$.
	From~\eqref{eq:y}, if $t \in [h_k, {h_{k+1}})$ for some $k\in[n]$, we then have
	\begin{align*}
		\y_{t+1} 
		&= \sum_{j=0}^t \sX_{j+1}^t\eta_j  \seps_j 
		= (\sX_{t+1}^T)^{-1} \sum_{j=0}^t \sX_{j+1}^T\eta_j  \seps_j \\
		&=(\sX_{t+1}^T)^{-1}  \left[ \sum_{j=0}^{h_k-1} \sX_{j+1}^T\eta_j  \seps_j + \sum_{j=h_k}^t \sX_{j+1}^T\eta_j  \seps_j \right]\\
		&= \sX_{h_k}^{t} \y_{h_k} + \sum_{j=h_k}^t \sX_{j+1}^t\eta_j  \seps_j.
	\end{align*}
	When $T$ is sufficiently large ($T \ge n j_0$ is sufficient with $j_0$ defined in~\ref{lem:vanish-norm} of Lemma~\ref{lem:A}), we have
	\begin{align}
		&\PB\left(    
		\frac{1}{\sqrt{T}} \sup_{0 \le t \le T} \frac{\|\y_{t+1}\|}{\eta_{t+1}} \ge 2\eps; \AM
		\right) \nonumber \\
		&\le \sum_{k=0}^{n-1}	\PB\left(    
		\frac{1}{\sqrt{T}} \sup_{t \in [h_k , {h_{k+1}})}\frac{\|\y_{t+1}\|}{\eta_{t+1}}\ge 2\eps; \AM
		\right) \nonumber \\
		&\le \sum_{k=0}^{n-1}\PB\left(    
		\frac{1}{\sqrt{T}} \sup_{t \in [h_k,  {h_{k+1}})}\frac{1}{\eta_{t+1}}
		\left[
		\left\| \sX_{h_k}^{t} \y_{h_k} \right\| 
		+ 	\left\|  \sum_{j=h_k}^t \sX_{j+1}^{t}\eta_j  \seps_j \right\| 
		\right] \ge 2\eps; \AM
		\right) \nonumber \\
		&\le \sum_{k=0}^{n-1}\PB\left(    
		\frac{1}{\sqrt{T}} \sup_{t \in [h_k,  {h_{k+1}})}\frac{\eta_{h_k}}{\eta_{t+1}}
		\left\| \sX_{h_k}^{t}\right\| \left\|  \frac{\y_{h_k}}{\eta_{h_k}} \right\|
		\ge \eps; \AM
		\right) \nonumber \\
		& \qquad +	\sum_{k=0}^{n-1}\PB\left(    
		\frac{1}{\sqrt{T}} \sup_{t \in [h_k,  {h_{k+1}})}\frac{1}{\eta_{t+1}}	\left\|  \sum_{j=h_k}^t \sX_{j+1}^{t}\eta_j  \seps_j \right\| 
		\ge \eps; \AM
		\right)  \nonumber \\
		&\overset{(a)}{\le}\sum_{k=0}^{n-1}\PB\left(    
		\frac{1}{\sqrt{T}} \sup_{t \in [h_k,  {h_{k+1}})}\frac{1}{\eta_{t+1}}	\left\| \sum_{j=h_k}^t \sX_{j+1}^{t}\eta_j  \seps_j \right\| 
		\ge \eps; \AM
		\right)  \nonumber \\
		&\le\sum_{k=0}^{n-1}\PB\left(    
		\frac{1}{\sqrt{T}} \sup_{t \in [h_k,  {h_{k+1}})}\frac{1}{\eta_{t+1}}	\left\| \sum_{j=h_k}^t \sX_{j+1}^{t}\eta_j  \seps_j \right\| 
		\ge \eps
		\right)  := \sum_{k=0}^{n-1} \PM_k \label{eq:P-bound}
	\end{align}

	Here $(a)$ uses the following result.
	When $k \ge 1$, due to $h_k \ge \ceil{\frac{k}{n}(T+1)}$, $h_k$ could be arbitrarily large with increasing $T$ and fixed $n$.
	From~\ref{lem:bounded-X} and~\ref{lem:vanish-norm} of Lemma~\ref{lem:A}, when $h_k \ge j_0$,
	\[
	\frac{\eta_{h_k}}{\eta_{t+1}}
	\left\| \sX_{h_k}^{t} \right\| \le 	
	\exp\left( \frac{c}{2} \sum_{t=h_k}^{t+1} \eta_t \right)
	\cdot c_0 \exp\left( -c \sum_{t=h_k}^{t} \eta_t \right)
	\le c_0 \exp(c\eta_0)
	= c_0'.
	\]
	which implies $\sup_{t \in [h_k,  {h_{k+1}})}\frac{\eta_{h_k}}{\eta_{t+1}}
	\left\| \sX_{h_k}^{t} \right\| \le c_0'$ for any $ k \ge 1$.
	Notice $\frac{c_0'}{\sqrt{T}}\left\| \frac{\y_{h_k}}{\eta_{h_k}} \right\| \ge \eps$ is impossible on the event $\AM$.
	We then have
	\begin{align*}
		\PB\left(    
		\frac{1}{\sqrt{T}} \sup_{t \in [h_k,  {h_{k+1}})}\frac{\eta_{h_k}}{\eta_{t+1}}
		\left\| \sX_{h_k}^{t} \right\| \left\|  \frac{\y_{h_k}}{\eta_{h_k}} \right\|
		\ge \eps; \AM
		\right) 
		\le 	\PB\left(    
		\frac{c_0'}{\sqrt{T}} \left\|  \frac{\y_{h_k}}{\eta_{h_k}} \right\|
		\ge \eps; \AM
		\right) 
		= 0 
	\end{align*}
	When $k=0$, the above probability is clearly zero since $\y_0 = \0$.
	%	As a result, we have
	%	\[
	%	\PB\left(    
	%	\frac{1}{\sqrt{T}} \sup_{0 \le t \le T} \frac{\|\y_{t+1}\|}{\eta_{t+1}} \ge 2\eps; \AM \right)
	%	\le \sum_{k=0}^{n-1} \PM_k
	%	\ \text{with} \
	%			\PM_k := \PB\left(    
	%	\sup_{t \in [h_k,  {h_{k+1}})}\frac{1}{\eta_{t+1}}	\left\| \sum_{j=h_k}^t \sX_{j+1}^{t}\eta_j  \seps_j \right\| 
	%	\ge \sqrt{T}\eps
	%	\right). 
	%	\]
	
	\paragraph{Step two: Bound each $\PM_k$}
	The proof of Lemma~\ref{lem:P-bound} can be found in Section~\ref{proof:P-bound}.
	\begin{lem}
		\label{lem:P-bound}
		Assume $T \ge n$. For each $k \in [n]$,
		\[
		\PM_k := \PB\left(    
		\sup_{t \in [h_k,  {h_{k+1}})}\frac{1}{\eta_{t+1}}	\left\| \sum_{j=h_k}^t \sX_{j+1}^{t}\eta_j  \seps_j \right\| 
		\ge \sqrt{T}\eps
		\right) \le p^p  C_3^p \cdot n^{-\frac{p}{2}} \eps^{-p}
		\]
		where $C_3$ is a positive constant depending on the step sizes, $\sG, d$ and $\sup_{t \ge 0}\sqrt[p]{\EB\|\varepsi_t\|^p}$.
		In short, $C_3$ has nothing to do with $p$.
	\end{lem}
	\paragraph{Step three: Put pieces together}
	Therefore,
	
	\begin{align*}
		\PB\left(    
		\frac{1}{\sqrt{T}} \sup_{0 \le t \le T} \frac{\|\y_{t+1}\|}{\eta_{t+1}} \ge 2\eps
		\right)
		&\le \PB\left(    
		\frac{1}{\sqrt{T}} \sup_{0 \le t \le T} \frac{\|\y_{t+1}\|}{\eta_{t+1}} \ge 2\eps; \AM
		\right) + \PB(\AM^c)\\
		&\overset{(a)}{\le} \sum_{k=0}^{n-1} \PM_k + \frac{c_2(c_0')^2(n+1)}{\eta_{T}T\eps^2}
		\overset{(b)}{\precsim} p^p C_3^p \eps^{-p} n^{-\frac{p}{2}+1} + \frac{n}{\eta_{T}T\eps^2}.
	\end{align*}
	where $(a)$ uses~\eqref{eq:P-bound} and~\eqref{eq:P-A-c} and $(b)$ uses Lemma~\ref{lem:P-bound}.
	As a result, for any $\eps > 0$,
	\[
	\limsup_{T \to \infty}\PB\left(    
	\frac{1}{\sqrt{T}} \sup_{0 \le t \le T} \frac{\|\y_{t+1}\|}{\eta_{t+1}} \ge 2\eps
	\right) \precsim p^p C_3^p \eps^{-p} n^{-\frac{p}{2}+1}.
	\]
	Since $p>2$ and the probability of the left-hand side has nothing to do with $n$, letting $n \to \infty$ concludes the proof.
\end{proof}

\subsection{Proof of Lemma~\ref{lem:P-bound}}
\label{proof:P-bound}
\begin{proof}[Proof of Lemma~\ref{lem:P-bound}]
	Readers should keep in mind that we only have $p>2$ in this part.
	Without loss of generality, we fix $k \in [n]$.
	
	\paragraph{Step one: Diagonalization}
	Since $\sG$ is diagonalizable, there exist two non-singular matrices $\sU, \sD \in \mathbb{C}^{d \times d}$ that satisfy $\sG = \sU \sD \sU^{-1}$ and $\sD$ is a diagonal matrix with each entry the eigenvalue of $\sG$.\footnote{In this proof, with a slight abuse of notation, we use $\sU$ to denote a non-singular complex matrix. Readers should distinguish it from the bivariate function $\sU(\x, \xi)$ defined in Lemma~\ref{lem:poisson}.}
	Further, $\sD = \diag(\{\lambda_i(\sG)\}_{i \in [d]})$ and $\mathrm{Re}\lambda_i(\sG) > 0$.
	Therefore, denote $	\tsX_j^t  :=  \prod\limits_{i=j}^{t}\left( \sI - \eta_{i}\sD \right)$ and thus we have
	\[
	\sU^{-1} \sum_{j=h_k}^t \sX_{j+1}^{t}\eta_j  \seps_j  = \sum_{j=h_k}^t \left(\prod\limits_{i=j+1}^{t}\left( \sI - \eta_{i}\sD \right)\right) \eta_{j} \sU^{-1}\seps_{j} 
	= \sum_{j=h_k}^t \tsX_{j+1}^t \eta_{j} \sU^{-1}\seps_{j} 
	\]
	Hence, 
	\begin{align*}
		\PM_k 
		&= \PB\left(    
		\sup_{t \in [h_k,  {h_{k+1}})}\frac{1}{\eta_{t+1}}	\left\| \sum_{j=h_k}^t \sX_{j+1}^{t}\eta_j  \seps_j \right\| 
		\ge \sqrt{T}\eps
		\right)\\ 
		&\le  \PB\left(    
		\sup_{t \in [h_k,  {h_{k+1}})}\frac{1}{\eta_{t+1}}
		\left\|  \sum_{j=h_k}^t \tsX_{j+1}^t \eta_{j} \sU^{-1}\seps_{j} \right\| 
		\ge \frac{\sqrt{T}\eps}{\|\sU\|}
		\right)\\ 
		&\overset{(a)}{\le} \sum_{i=1}^d  \PB\left(    
		\sup_{t \in [h_k,  {h_{k+1}})}\frac{1}{\eta_{t+1}}
		\left|  \left( \sum_{j=h_k}^t \tsX_{j+1}^t \eta_{j} \sU^{-1}\seps_{j} \right)_i\right| 
		\ge \frac{\eps}{\|\sU\|}\sqrt{\frac{T}{d}}
		\right)\\ 
		&\overset{(b)}{=} \sum_{i=1}^d  \PB\left(    
		\sup_{t \in [h_k,  {h_{k+1}})}\frac{1}{\eta_{t+1}}
		\left|  \sum_{j=h_k}^t (\tsX_{j+1}^t)_{i,i} \eta_{j}  \left(\sU^{-1}\seps_{j} \right)_i\right| 
		\ge \frac{\eps}{\|\sU\|}\sqrt{\frac{T}{d}}
		\right) := \sum_{i=1}^d \PM_{k, i}
	\end{align*}
	where $(a)$ uses the notation $(\sv)_i$ denotes the $i$-th coordinate of the vector $\sv$ and $|\cdot|$ denotes the norm for complex numbers and $(b)$ uses the fact that $\sG$ is a diagonal matrix.
	The above analysis shows we only need to focus on each coordinate thanks to diagonalization.

	\paragraph{Step two: Establish tail probability bound for each coordinate}
	Without loss of generality, we fix any coordinate $i \in [d]$.
	Let $\lambda := \lambda_i(\sG)$ denotes the $i$-th eigenvalue for short (only in this part).
	With a little abuse of notation, we set $X_{j+1}^t :=	(\tsX_{j+1}^t)_{i,i}$ and $\eps_j = (\sU^{-1}\varepsi_j)_i$, both complex numbers and $X_{j+1}^t = \prod\limits_{i=j+1}^{t}\left( \sI - \eta_{i}\lambda\right)$.
	Hence, $\PM_k \le \sum_{i=1}^d \PM_{k, i}$ where
	\begin{align}
		\PM_{k, i} &=  \PB\left(    
		\sup_{t \in [h_k,  {h_{k+1}})}\frac{1}{\eta_{t+1}}
		\left|  \sum_{j=h_k}^t X_{j+1}^t \eta_{j} \eps_j\right| 
		\ge \frac{\eps}{\|\sU\|}\sqrt{\frac{T}{d}}
		\right) \nonumber \\
		&=  \PB\left(    
		\sup_{t \in [h_k,  {h_{k+1}})}\frac{1}{\eta_{t+1}}
		\left|  (X_{t+1}^T)^{-1}  \sum_{j=h_k}^t X_{j+1}^T \eta_{j} \eps_j\right| 
		\ge \frac{\eps}{\|\sU\|}\sqrt{\frac{T}{d}}
		\right) \nonumber \\
		&\overset{(a)}{=}  \PB\left(    
		\sup_{t \in [h_k,  {h_{k+1}})}\frac{1}{\eta_{t+1}} \left|(X_{t+1}^T)^{-1} \right|
		\left|   \sum_{j=h_k}^t X_{j+1}^T \eta_{j} \eps_j\right| 
		\ge \frac{\eps}{\|\sU\|}\sqrt{\frac{T}{d}}
		\right)  \nonumber \\
		&\overset{(b)}{=}  \PB\left(    
		\sup_{t \in [h_k,  {h_{k+1}})}\frac{1}{\left|\eta_{t+1}X_{t+1}^T \right|} 
		\left|   \sum_{j=h_k}^t X_{j+1}^T \eta_{j} \eps_j\right| 
		\ge \frac{\eps}{\|\sU\|}\sqrt{\frac{T}{d}}
		\right) \nonumber\\
		&=\PB\left( 
		\sup_{t \in [h_k,  {h_{k+1}})}\frac{1}{\left|\eta_{t+1}X_{t+1}^T \right|^p} 
		\left|   \sum_{j=h_k}^t X_{j+1}^T \eta_{j} \eps_j\right|^p 
		\ge \left( \frac{\eps}{\|\sU\|}\sqrt{\frac{T}{d}}\right)^{p}
		\right)
		\label{eq:P_ki}
	\end{align}
	where $(a)$ follows from $|ab| = |a|\cdot|b|$ for any $a, b \in \mathbb{C}$; and $(b)$ follows from $|a^{-1}| \cdot |a| = 1$ for any $a \neq 0 \in \mathbb{C}$.

	\begin{lem}[Chow's inequality~\citep{chow1960martingale}]
		\label{lem:chow}
		Let $\{Y_t\}_{t \ge 0} \subseteq \RB$ be a sub-martingale and $\{b_t\}_{t \ge 0}$ be a non-increasing sequence.
		Denote $Y_t^+ = \max(0, Y_t)$.
		Then for any $\eps > 0$, we have
		\[
		\eps  \cdot \PB\left( \sup_{0 \le t \le T}b_tY_t   \ge \eps\right)
		\le \sum_{t=0}^{T-1} (b_t-b_{t+1}) \EB Y_t^+ + b_T \EB Y_T^+.
		\]
	\end{lem}
	
	\begin{lem}[Burkholder's inequalities~\citep{burkholder1988sharp}]
		Fix any $p \ge 2$.
		For $\mathbb{C}$-valued martingale difference $X_1, \cdots, X_T$, each with finite $L^p$-norm, one has
		\[
		\EB\left| \sum_{t=1}^T X_t\right|^p 
		\le B_p^p \EB \left(\sum_{t=1}^T |X_t|^2 \right)^{\frac{p}{2}}
		\]
		where $B_p= \max\left\{p-1, \frac{1}{p-1}\right\}$ is a universal constant depending only on $p$.
		It together with Jensen's inequality implies
		\begin{equation}
			\label{eq:burk}
			\EB\left| \sum_{t=1}^T X_t\right|^p 
			\le B_p^p T^{\frac{p}{2}-1} \sum_{t=1}^T\EB |X_t|^{p}.
		\end{equation}
	\end{lem}
	Based on~\eqref{eq:P_ki}, we will use Chow's inequality to bound each  $\PM_{k,i }$'s.
	We first check~\eqref{eq:P_ki} satisfies the conditions in Lemma~\ref{lem:chow}.
	First, $\eta_{t+1}\left|X_{t+1}^T \right|$ is non-decreasing for when $t$ is sufficiently large.
	This is because
	\begin{equation}
		\label{eq:eta-X}
		\eta_{t}\left|X_{t}^T \right|
		=  \frac{\eta_t}{\eta_{t+1}} \left|1 - \eta_t \lambda \right|  \cdot \eta_{t+1}\left|X_{t+1}^T \right|
		\le \eta_{t+1}\left|X_{t+1}^T \right|
	\end{equation}
	for which we use 
	\[
	\frac{\eta_t}{\eta_{t+1}} \left|1 - \eta_t \lambda \right| 
	= (1+o(\eta_t))\sqrt{(1-\eta_t \mathrm{Re} \lambda)^2 + \eta_t^2(\mathrm{Im} \lambda)^2} 
	=(1+o(\eta_t))\sqrt{1-2\eta_t \mathrm{Re} \lambda + O(\eta_t^2)}
	\le 1
	\]
	when $\eta_t$ is sufficiently small, or equivalently, $t$ is sufficiently large, say larger than $t_0'$.
	Hence, $b_t := \left|\eta_{t+1}X_{t+1}^T \right|^{-p}$ is non-increasing.
	Second, let $Y_t :=	\left|   \sum_{j=h_k}^t X_{j+1}^T \eta_{j} \eps_j\right|^p$.
	It is easy to check $Y_t$ is a sub-martingale satisfying $\EB[Y_t|\FM_{t-1}] \ge Y_{t-1}$.
	What's more,~\eqref{eq:burk} implies $\EB Y_t$ is bounded by
	\begin{align}
		\label{eq:final-Y}
		\EB Y_t 
		&\le B_p^p (t-h_k+1)^{\frac{p}{2}-1}  \sum_{j=h_k}^t \EB \left|X_{j+1}^T \eta_{j} \eps_j\right|^p \nonumber \\
		&\le B_p^p \left(\frac{T}{n}\right)^{\frac{p}{2}-1} \sum_{j=h_k}^t  \left|X_{j+1}^T \eta_{j} \right|^p \EB \left|  \eps_j\right|^p \nonumber \\
		&\le p^p C_3^p \cdot \left(\frac{T}{n}\right)^{\frac{p}{2}-1} \sum_{j=h_k}^t  \left|X_{j+1}^T \eta_{j+1} \right|^p =  C_3^p \cdot \left(\frac{T}{n}\right)^{\frac{p}{2}-1} \sum_{j=h_k}^t  \frac{1}{b_j}
	\end{align}
	where $C_3 :=2 \cdot \sup_{t \ge 0, i \in [d]}\sqrt[p]{\EB |\eps_{t} |^p}$ is a constant depending only on $\sU$ and $\sup_{t \ge 0}\sqrt[p]{\EB\|\varepsi_t\|^p}$.
	
	Hence, by Lemma~\ref{lem:chow} and~\eqref{eq:final-Y}, it follows that
	\begin{align*}
		\PM_{k, i} 
		&\le \left( \frac{\eps}{\|\sU\|}\sqrt{\frac{T}{d}}\right)^{-p} \cdot p^p C_3^p \left(\frac{T}{n}\right)^{\frac{p}{2}-1}  \left[\sum_{t=h_k}^{h_{k+1}-2} \left( b_t -b_{t+1}\right) \sum_{j=h_k}^t  \frac{1}{b_j} + b_{h_{k+1}-1}  \sum_{j=h_k}^{h_{k+1}-1}  \frac{1}{b_j} \right]\\
		&= 
		\left( \frac{\sqrt{d}\|\sU\|}{\sqrt{T}\eps}\right)^{p}  \cdot p^pC_3^p \left(\frac{T}{n}\right)^{\frac{p}{2}-1}  \left[
		\sum_{j=h_k}^{h_{k+1}-2}\frac{1}{b_j} \sum_{t=j}^{h_{k+1}-2} \left( b_t -b_{t+1}\right)  + b_{h_{k+1}-1}  \sum_{j=h_k}^{h_{k+1}-1}  \frac{1}{b_j} \right]\\
		&\le  	\left( \frac{\sqrt{d}\|\sU\|}{\sqrt{T}\eps}\right)^{p} \cdot
		p^pC_3^p  \left(\frac{T}{n}\right)^{\frac{p}{2}} = p^pC_3^p 	\left( \frac{\sqrt{d}\|\sU\|}{\sqrt{n}\eps}\right)^{p}
	\end{align*}
	which implies that for any $k \ge 1$,
	\[
	\PM_k \le \sum_{i \in [d]} \PM_{k, i}  \le p^p C_3^p d^{1+\frac{p}{2}} \cdot\left( \frac{\|\sU\|}{\sqrt{n}\eps}\right)^{p}.
	\]
	For $k=0$, in order to establish~\eqref{eq:eta-X}, we can follow the same argument of bounding each $\PM_k$'s by noticing
	\begin{align*}
		\PM_0 &=  \PB\left(    
		\sup_{t \in [h_0,  {h_{1}})}\frac{1}{\eta_{t+1}}	\left\| \sum_{j=h_0}^t \sX_{j+1}^{t}\eta_j  \seps_j \right\| 
		\ge \sqrt{T}\eps
		\right)\\
		&\le   \PB\left(    
		\sup_{t \in [0,  t_0')}\frac{1}{\eta_{t+1}}	\left\| \sum_{j=0}^t \sX_{j+1}^{t}\eta_j  \seps_j \right\| 
		\ge 0.5\sqrt{T}\eps
		\right) \\
		& \qquad+ \PB\left(  \left\| \sX_{0}^{t_0'} \right\|
		\sup_{t \in [t_0',  {h_{1}})}\frac{1}{\eta_{t+1}}	\left\| \sum_{j=t_0'}^t \sX_{j+1}^{t}\eta_j  \seps_j \right\| 
		\ge 0.5\sqrt{T}\eps
		\right)\\
		&\le\frac{ 2^p }{T^{\frac{p}{2}}\eps^p} \cdot \EB\left[\sup_{t \in [0,  t_0')}\frac{1}{\eta_{t+1}}	\left\| \sum_{j=0}^t \sX_{j+1}^{t}\eta_j  \seps_j \right\| \right]^p  + p^p C_3^p 2^p \left\| \sX_{0}^{t_0'} \right\|^pd^{1+\frac{p}{2}} \cdot	\left( \frac{\|\sU\|}{\sqrt{n}\eps}\right)^{p}\\
		&\le p^p C_3^p n^{-\frac{p}{2}} \eps^{-p}
	\end{align*}
	where the last inequality redefines $C_3$ by enlarging the original $C_3$ and $T \ge n$.
	Note that the moment quantity in the first term, $\|\sX_0^{t_0'}\|, t_0', \|\sU\|$ depends on $\sG, \{\eta_t\}_{t \ge 0}$.
	$C_3$ is a quantity that depends on $\sG, d$ and $\sup_{t \ge 0}\sqrt[p]{\EB\|\varepsi_t\|^p}$.
	
	% 	Finally, we complete the proof by redefining $C_3$ to be
	% 	\[
	% 	C_3 := 2C_3 \left\| \sX_{0}^{t_0'} \right\| d^{\frac{1}{p}+\frac{1}{2}}\|\sU\| \le 4 \left\| \sX_{0}^{t_0'} \right\| d^{\frac{1}{p}+\frac{1}{2}}\|\sU\| \sqrt[p]{B_p} \cdot \sup_{t \ge 0, i \in [d]}\sqrt{\EB |(\sU^{-1}\varepsi_{t})_i |^p}
	% 	\]
	%  which is a quantity that depends on $\sG, d$ and  $\sup_{t \ge 0}\sqrt{\EB\|\varepsi_t\|^p}$.
	%  Here $o(1)$ denotes a term that converges to zero when $T$ goes to infinity.
	% The $o(1)$ can also be bounded in terms of $\OM(n^{-p/2}\varepsilon^{-p})$ due to Markov's inequality.
	% The constant hidden in the $\OM(\cdot)$ depends on $\alpha, \sup_{t \ge 0}\sqrt{\EB\|\varepsi_t\|^p}$ and $\sG$ and has nothing to do with $p$.
	% Then we can enlarge $C_3$ as before.
\end{proof}

\subsection{Proof of Lemma~\ref{lem:srgt_unf_op}}
\label{proof:srgt_unf_op}
\begin{proof}[Proof of Lemma~\ref{lem:srgt_unf_op}]
	By definition, we have that
	\[
	z_{t+1} = \ssum{j}{0}{t}\left(\prod\limits_{i=j+1}^{t}(1-\lambda\eta_i)\right)\eta_j\omega_j.
	\]
	The last equation implies that
	\begin{align*}
		\frac{1}{\sqrt{T}}\sup\limits_{t\in[0,T]}\frac{|z_{t+1}|}{\eta_t} &= 
		\frac{1}{\sqrt{T}}\sup\limits_{t\in[0,T]}\frac{1}{\eta_t}\left|\ssum{j}{0}{t}\prod\limits_{i=j+1}^t(1-\lambda\eta_j)\eta_j\omega_j\right|\\
		&\le \frac{1}{\sqrt{T}}\sup\limits_{t\in[0,T]}\frac{1}{\eta_t}\ssum{j}{0}{t}\prod_{i=j+1}^t\eta_j|1-\lambda\eta_j||\omega_j|\\
		&= \sup\limits_{t\in[0,T]}\frac{1}{\eta_t}\ssum{j}{0}{t}\eta_j^2\prod_{i=j+1}^t|1-\lambda\eta_j|\times \frac{|\omega_j|}{\eta_j\sqrt{T}}\\
		&\le \sup\limits_{t\in[0,T]}\frac{1}{\eta_t}\ssum{j}{0}{t}\eta_j^2\prod_{i=j+1}^t|1-\lambda\eta_j|\times \sup\limits_{\tau\in[0,t]}\frac{|\omega_\tau|}{\eta_\tau\sqrt{T}}\\
		&\le \left(\sup\limits_{t\in[0,T]}\frac{1}{\eta_t}\ssum{j}{0}{t}\eta_j^2\prod_{i=j+1}^t|1-\lambda\eta_j|\right)\times \left(\sup\limits_{\tau \in[0,T]}\frac{|\omega_\tau|}{\eta_\tau\sqrt{T}}\right).
	\end{align*}
	The fact that $\lambda$ has a positive real part implies when $t$ is sufficiently large, we have
	\[
	|1-\lambda\eta_t| = \sqrt{(1-\mathrm{Re}(\lambda)\eta_t)^2 + \mathrm{Im}(\lambda)^2\eta_t^2} = \sqrt{1-2\mathrm{Re}(\lambda)\eta_t + 
		|\lambda|^2\eta_t^2} \precsim 1-\mathrm{Re}(\lambda)\eta_t \precsim \exp \left(-\mathrm{Re}(\lambda)\eta_t \right).
	\]
	By \ref{lem:bounded-norm} in Lemma \ref{lem:A}, there exists $c_1 > 0$ such that
	\[
	\sup\limits_{t\in[0,T]}\frac{1}{\eta_t}\ssum{j}{0}{t}\eta_j^2\prod_{i=j+1}^t|1-\lambda\eta_j| \le c_1.
	\]
	As a result, we have
	\begin{align*}
		\frac{1}{\sqrt{T}}\sup\limits_{t\in[0,T]}\frac{|z_{t+1}|}{\eta_t} &\le \left(\sup\limits_{t\in[0,T]}\frac{1}{\eta_t}\ssum{j}{0}{t}\eta_j^2\prod_{i=j+1}^t|1-\lambda\eta_j|\right)\times \left(\sup\limits_{t\in[0,T]}\frac{|\omega_t|}{\eta_t\sqrt{T}}\right) \le c_1\times \left(\sup\limits_{t\in[0,T]}\frac{|\omega_t|}{\eta_t\sqrt{T}}\right).
	\end{align*}
	We complete the proof by using the condition that  $\frac{1}{\sqrt{T}}\sup\limits_{t\in [0,T]}\frac{|\omega_t|}{\eta_{t}}\overset{p}{\to} 0$ as $T\to \infty$ and $\eta_{t}-\eta_{t+1} = \eta_t o(\eta_t)$.
\end{proof}

\subsection{Properties of Recursion Matrices}
\begin{lem}
	\label{lem:A}
	Recall that $\sB_i := \sI - \eta_i\sG$ and $-\sG$ is Hurwitz (i.e., $\mathrm{Re} \lambda_i(\sG) > 0$ for all $i \in [d]$).
	For any $n \ge j$, define $\sX_j^n$ and $\sA_{j}^{n}$ as
	\begin{gather}
		\sX_j^n :=\prod\limits_{i=j}^{n}\sB_i \label{eq:X} \\
		\sA_{j}^n := \sum\limits_{t=j}^{n}\sX_{j+1}^t \eta_j =\sum\limits_{t=j}^{n}\left(\prod\limits_{i=j+1}^{t}\sB_i\right) \eta_j.		\label{eq:A}
	\end{gather}
	When $\{\eta_t\}_{t \ge 0}$ satisfies Assumption~\ref{asmp:eta}, it follows that
	\begin{enumerate}[(i)]
		\item \label{lem:bounded-X}
		There exist constant $c_0, c >0$ such that for any $n \ge j \ge 0$,
		\[
		\|\sX_j^n\| \le c_0 \exp\left( -c \sum_{t=j}^n \eta_t \right).
		\]
		\item \label{lem:vanish-A}
		There exist $C_0$ such that $\sA_j^n$ is uniformly bounded with respect to both $j$ and $n$ for $0 \le j \le k$ (i.e., $\|\sA_j^n\| \le C_0$ for any $n \ge j \ge 0$), and
		\[
		\frac{1}{n} \sum_{j=0}^n \|\sA_{j}^{n} - \sG^{-1}\| \to 0 
		\ \text{as} \ n \to \infty.
		\]
		\item \label{lem:vanish-norm}
		For the $c$ given in~\ref{lem:bounded-X}, there exists $j_0 >0$ such that any $n \ge j \ge j_0$,
		\[
		\frac{\eta_{j-1}}{\eta_n} 
		\le \exp\left( \frac{c}{2} \sum_{t=j-1}^{n} \eta_t \right).
		\]
		\item \label{lem:bounded-norm}
		Let $c$ be a positive constant, then there exists another constant $c_1$ such that for any $n\ge 1$,
		\[
		\sum_{j=1}^n\eta_{j-1}^2\exp\left( -c \sum_{t=j}^n \eta_t \right) \le c_1 \eta_n.
		\]
	\end{enumerate}
\end{lem}
\begin{proof}[Proof of Lemma~\ref{lem:A}]
	\begin{enumerate}[(i)]
		\item The proof can be found in the proof of Lemma 3.1.1 in~\cite{chen2002stochastic}.
		\item The proof can be found in the proof of Lemma 3.4.1 in~\cite{chen2002stochastic}.
		\item 	Due to $\frac{\eta_{t-1} - \eta_{t}}{\eta_{t-1}} =o(\eta_{t-1})$, it follows that
		\[
		\frac{\eta_{j-1}}{\eta_n} = \prod_{t=j}^{n-1} \frac{\eta_{t-1}}{\eta_t}
		= \prod_{t=j}^{n-1}(1+o(1)\eta_t)
		\le \exp\left( o(1) \sum_{t=j}^{n-1} \eta_t \right)
		\le \exp\left( o(1) \sum_{t=j}^{n} \eta_t \right)
		\]
		where $o(1)$ denotes a magnitude that tends to zero as $j \to \infty$ and the last inequality follows from $\eta_n \to 0$.
		We then find $j_0>0$ such that any $n \ge j \ge j_0$, we have $	\frac{\eta_{j-1}}{\eta_n} 
		\le \exp\left( \frac{c}{2} \sum_{t=j-1}^{n} \eta_t \right)$ with $c$ given in~\ref{lem:bounded-X}.
		\item 		Lemma 3.3.2 in~\cite{chen2002stochastic} implies that for any $c >0$, $\sum_{j=1}^n\eta_{j-1}\exp\left( -c \sum_{t=j}^n \eta_t \right)$ is uniformly bounded for $n \ge 1$.
		When $n \to \infty$, as a result of $n \eta_n  \to \infty$, we have $c\sum_{t=1}^n \eta_t + \ln \eta_n \to \infty$ and thus $\eta_n^{-1}\exp\left( -c \sum_{t=1}^n \eta_t \right)  \to 0$.
		Therefore, we can find $n_0, c_3>0$ such that any $n\ge n_0$ we have $\sum_{j=1}^{j_0}\eta_{j-1}^2\exp\left( -c \sum_{t=j}^n \eta_t \right) \le c_3 \eta_n$.
		Then as long as $n \ge \max\{j_0, n_0\}$, it follows that
		\begin{align*}
			\sum_{j=1}^n\eta_{j-1}^2\exp\left( -c \sum_{t=j}^n \eta_t \right) 
			&=	\sum_{j=1}^{j_0}\eta_{j-1}^2\exp\left( -c \sum_{t=j}^n \eta_t \right)  + \sum_{j=j_0}^{n}\eta_{j-1}^2\exp\left( -c \sum_{t=j}^n \eta_t \right) \\
			&= c_3 \eta_n + \eta_n \sum_{j=j_0}^{n}\eta_{j-1}\exp\left( - \frac{c}{2}\sum_{t=j}^n \eta_t \right) \le c_1 \eta_n.
		\end{align*}
		For $n < \max\{j_0, n_0\}$, since there is only a finite number of cases, we can enlarge $c_1$ in order to cover all $n \ge 1$.
	\end{enumerate}
\end{proof}

\section{Proof for the consistency guarantee}
\label{proof:consistency}
We mainly adapt the generalize Lyapunov Lyapunov developed by~\citet{chen2020finite,chen2021lyapunov} to our case.
In this section, we will make use of the $\ell_\bp$-norm defined in $\RB^d$ denoted by $\|\cdot\|_\bp$.
Readers should keep in mind that the $\bp$ used in this section has noting to do with that $p$ defined in Assumption~\ref{asmp:noise}.
%\citet{chen2020finite,chen2021lyapunov} choose a proper value of $\bp$ in order to obtain a tight dependence on the ambient dimension $d$.

\begin{lem}[Smoothness and approximation of the envelope,  Lemma 2.1 in~\citet{chen2020finite}]
	\label{lem:envelop}
	Let $\|\cdot\|_\bp$ denote the $\ell_\bp$-norm defined in $\RB^d$.
	Define the Moreau envelope of $\frac{1}{2}\|\cdot\|^2$ w.r.t. $\frac{1}{2}\|\cdot\|_\bp^2$ as
	\[
	M(\x) = \min_{\su \in \RB^d} \left[ \frac{1}{2}\|\su\|^2+\frac{\lambda}{2}\|\x-\su\|_\bp^2 \right].
	\]
	We then have the following results
	\begin{enumerate}[(i)]
		\item  \label{asmp:smooth-envelop} $M(\x)$ is convex in $\x$ and is $(\bp-1)\lambda$-smooth w.r.t. the norm $\|\cdot\|_\bp$.
		\item \label{asmp:appro-envelop}Suppose $l_\bp \|\cdot\| \le \|\cdot\|_\bp \le  u_\bp \|\cdot\|$, then for all $\x \in \RB^d$,
		\[
		\left( 1 + \frac{\lambda}{u_\bp^2} \right)M(\x) \le \frac{1}{2}\|\x\|^2 \le \left( 1 + \frac{\lambda}{l_\bp^2} \right)M(\x).
		\]
		\item \label{asmp:norm-envelop} There exists one norm $\|\cdot\|_M$ such that $M(\x) = \frac{1}{2}\|\x\|_M^2$ for all $\x \in \RB^d$.
	\end{enumerate}
\end{lem}

\begin{proof}[Proof of Theorem~\ref{thm:consistency}]
	Recall that the update rule is $\x_{t+1} = \x_t - \eta_t  \sH(\x_t, \xi_t) $.
	Hence, it follows that
	\begin{align}
		\label{eq:M-recur}
		M(\x_{t+1}-\x^{\star}) 
		&\le M(\x_t-\x^{\star}) + \langle \nabla M(\x_t-\x^{\star}),  \x_{t+1}-\x_t \rangle + \frac{(\bp-1)\lambda}{2} \|\x_t -\x_{t+1}\|_\bp^2\nonumber \\
		&= M(\x_t-\x^{\star}) - \eta_t \langle \nabla M(\x_t-\x^{\star}),  \sH(\x_t, \xi_t) \rangle + \frac{(\bp-1)\lambda\eta
			_t^2}{2} \|\sH(\x_t, \xi_t) \|_\bp^2.
	\end{align}
	
	\subsection{Establishment of $(L^2, a_t\sqrt{\eta_t})$-consistency}
	
	Let $\GM_t = \sigma(\{ \xi_\tau\}_{0 \le \tau < t})$ be the $\sigma$-filed generated by all random variables $\{\xi_\tau\}_{0\le \tau <t}$ strictly before iteration $t$.
	Clearly, $\x_t$ is $\GM_t$-measurable.
	For one thing,
	\begin{align}
		\label{eq:M-quadratic}
		\EB\|\sH(\x_t, \xi_t) \|_\bp^2
		&\le \EB \left(\|\sH(\x_t, \xi_t) -\sH(\x^{\star}, \xi_t)\|_\bp + \|\sH(\x^{\star}, \xi_t) \|_\bp\right) ^2 \nonumber \\
		&\le 2 \left(\EB\|\sH(\x_t, \xi_t) -\sH(\x^{\star}, \xi_t)\|_\bp^2 +\EB \|\sH(\x^{\star}, \xi_t) \|_\bp^2\right)\nonumber \\
		&\le 2 u_\bp^2 \left(\EB \|\sH(\x_t, \xi_t) -\sH(\x^{\star}, \xi_t)\|^2 + \EB\|\sH(\x^{\star}, \xi_t) \|^2\right) \nonumber \\
		&\le 2 u_\bp^2  \left(\EB\PM\|\sH(\x_t, \xi_{t-1}) -\sH(\x^{\star}, \xi_{t-1})\|^2 + \EB\|\sH(\x^{\star}, \xi_{t}) \|^2\right)\nonumber \\
		&\overset{(a)}{\le} 2u_\bp^2 \left( L_H^2 \EB\| \x_t -\x^{\star}\|^2 + \EB\|\sH(\x^{\star}, \xi_{t}) \|^2 \right)\nonumber \\
		&\overset{(b)}{\le} 2 u_\bp^2 \left(
		2L_H^2 \left(1+\frac{\lambda}{l_\bp^2}\right) \EB M(\x_t-\x^{\star}) + \EB\|\sH(\x^{\star}, \xi_{t}) \|^2 \right),
	\end{align}
	where $(a)$ uses Assumption~\ref{asmp:H} and $(b)$ uses~\ref{asmp:appro-envelop} in Lemma~\ref{lem:envelop}.
	
	For another thing, we decompose the cross term into three part as following
	\begin{align}
		\EB&\langle \nabla M(\x_t-\x^{\star}),  \sH(\x_t, \xi_t) \rangle  \nonumber \\
		&=\EB \left[\EB[\langle \nabla M(\x_t-\x^{\star}),  \sH(\x_t, \xi_t) \rangle |\GM_t] \right] 
		=\EB \langle \nabla M(\x_t-\x^{\star}),  \PM\sH(\x_t, \xi_{t-1}) \rangle \nonumber \\
		\begin{split}
			\label{eq:M-cross}
			&= \EB \underbrace{\langle \nabla M(\x_t-\x^{\star}),   \PM\sH(\x_t, \xi_{t-1}) -  \PM\sH(\x^{\star}, \xi_{t-1}) - c (\x_t-\x^{\star})\rangle }_{I} \\
			&\quad + \EB\underbrace{c \langle \nabla M(\x_t-\x^{\star}),  \x_t-\x^{\star} \rangle }_{II}
			+ \EB \underbrace{ \langle \nabla M(\x_t-\x^{\star}),  \PM\sH(\x^{\star}, \xi_{t-1}) \rangle}_{III}.
		\end{split}
	\end{align}
	From~\ref{asmp:norm-envelop} in Lemma~\ref{lem:envelop}, we have $M(\x) = \frac{1}{2}\|\x\|_M^2$ for all $\x \in \RB^d$.
	Hence, $\nabla M(\x) = \|\x\|_M \sv_\x$ where $\sv_\x \in \partial  \|\x\|_M$ is a subgradient of the function $\|\x\|_M$ at $\x$. 
	Let $\|\cdot\|_M^{\star}$ denote the dual norm of $\|\cdot\|_M$, defined by $\|\x\|_M^{\star} = \sup_{\|\y\|_M \le 1} \langle\x, \y \rangle$.
	Since $\|\cdot\|_M$ is a 1-Lipschitz w.r.t. the norm itself, we have $\|\x\|_M^{\star} \le 1$ for all $\x \in \RB^d$. 
	
	We are going to analyze the three terms in~\eqref{eq:M-cross} respectively in the following.
	\paragraph{For the term $I$} By Assumption~\ref{asmp:lya}, it follows that
	\begin{align*}
		|I| &\le \|\x_t-\x^{\star}\|_M \|\sv_{\x_t-\x^{\star}} \|_M^{\star} \|\PM\sH(\x_t, \xi_{t-1}) -  \PM\sH(\x^{\star}, \xi_{t-1}) -  c(\x_t-\x^{\star})\|_M\\
		&\le \|\x_t-\x^{\star}\|_M  \|\PM\sH(\x_t, \xi_{t-1}) -  \PM\sH(\x^{\star}, \xi_{t-1}) -  c(\x_t-\x^{\star})\|_M
	\end{align*}
	For another thing, by~\ref{asmp:appro-envelop} in Lemma~\ref{lem:envelop}, $\left( 1 + \frac{\lambda}{u_\bp^2} \right)M(\x) \le \frac{1}{2}\|\x\|^2 \le \left( 1 + \frac{\lambda}{l_\bp^2} \right)M(\x) $, which is equivalent to $\frac{l_\bp}{\sqrt{l_\bp^2+\lambda}} \|\x\| \le \|\x\|_M \le \frac{u_\bp}{\sqrt{u_\bp^2+\lambda}} \|\x\|$ for all $\x \in \RB^d$.
	Hence,
	\begin{align*}
		\|\PM&\sH(\x_t, \xi_{t-1}) -  \PM\sH(\x^{\star}, \xi_{t-1}) -  c(\x_t-\x^{\star})\|_M\\ 
		&\le \frac{u_\bp}{\sqrt{u_\bp^2+\lambda}} \|\PM\sH(\x_t, \xi_{t-1}) -  \PM\sH(\x^{\star}, \xi_{t-1}) -  c(\x_t-\x^{\star})\|\\
		&\le \frac{c \gamma  u_\bp}{\sqrt{u_\bp^2+\lambda}} \|\x_t-\x^{\star}\|
		\le c\gamma  \cdot 
		\frac{ u_\bp\sqrt{l_\bp^2+\lambda}}{l_\bp\sqrt{u_\bp^2+\lambda}} \|\x_t-\x^{\star}\|_M.
	\end{align*}
	As a result,
	\begin{equation}
		\label{eq:cross-I}
		|I| \le 2c\gamma  \frac{ u_\bp\sqrt{l_\bp^2+\lambda}}{l_\bp\sqrt{u_\bp^2+\lambda}} M(\x_t -\x^{\star}).
	\end{equation}
	
	\paragraph{For the term $II$} 
	Since $\|\cdot\|_M$ is a convex function of $\x$,  we have by the definition of convexity that $\|\0\|_M - \|\x_t -\x^{\star}\|_M \ge \langle  \sv_{\x_t-\x^{\star}}, -(\x_t-\x^{\star}) \rangle$. Hence,
	\begin{align}
		\label{eq:cross-II}
		II = c  \|\x_t-\x^{\star}\|_M \langle  \sv_{\x_t-\x^{\star}}, \x_t-\x^{\star}\rangle \ge c\|\x_t-\x^{\star}\|_M ^2 = 2c M(\x_t-\x^{\star}).
	\end{align}

	\paragraph{For the term $III$} 
	The the term $III$ exists due to Markovian data.
	%In the following, we denote $\|\cdot\|_*$ by the dual norm of $\|\cdot\|$ defined by $\|\x\|_* = \sup_{\|\y\|\le 1} \langle \x, \y \rangle$.
	%Due to norms are equivalent in any finite-dimensional spaces, we assume $\|\x\|_* \le u_* \|\x\|$ for all $\x \in \RB^d$. 
	Note that $\x_t, \nabla M(\x_t -\x^{\star}) \in \GM_t$ and $\xi_{t-1} \in \GM_t$.
	By Lemma~\ref{lem:geo-con} and Assumption~\ref{asmp:H}, for any $t \ge 0$,
	\begin{align*}
		\|\EB[\sH(\x^{\star}, \xi_{t+1})|\xi_0=\xi] \|
		&= \| \PM^{t+1}\sH(\x^{\star}, \xi)\|
		\le \kappa \rho^t \sup_{\xi \in \Xi} \| \PM \sH(\x^{\star}, \xi) \|\le  \kappa \sigma \rho^{t}.
	\end{align*}
	Therefore, we are motivated to define
	\begin{equation}
		\tag{\ref{eq:at}}
		a_t = \ceil{\log_{\rho} \frac{\eta_t}{\sigma \kappa}}
		\ \text{if} \ \rho > 0; \ a_t = 0 \ \text{otherwise},
	\end{equation}
	for each $t \ge0$ such that for any $\xi \in \Xi$,
	\begin{align}
		\begin{split}
			\label{eq:a_t-H}
			\|\PM^{a_t+1}\sH(\x^{\star}, \xi)\|
			&=
			\|\EB[\sH(\x^{\star}, \xi_{a_t+1})|\xi_0=\xi] \|  =\|\EB[\sH(\x^{\star}, \xi_t)|\xi_{t-a_t-1}=\xi] \| \le \eta_t,
		\end{split}
	\end{align}
	where the last equality holds because we consider a time-homogeneous Markov chain.
	Then,
	\begin{align}
		\EB III 
		&= \EB \langle \nabla M(\x_t-\x^{\star})-\nabla M(\x_{t-a_t}-\x^{\star}),  \sH(\x^{\star}, \xi_{t}) \rangle  \nonumber \\
		& \qquad + \EB \langle \nabla M(\x_{t-a_t}-\x^{\star}), \sH(\x^{\star}, \xi_{t}) \rangle\nonumber \\
		&= \EB \langle \nabla M(\x_t-\x^{\star})-\nabla M(\x_{t-a_t}-\x^{\star}),  \EB[\sH(\x^{\star}, \xi_{t})|\GM_{t}] \rangle \nonumber \\
		& \qquad + \EB \langle \nabla M(\x_{t-a_t}-\x^{\star}), \EB[\sH(\x^{\star}, \xi_{t})|\GM_{t-a_t}]  \rangle \nonumber \\
		\begin{split}
			\label{eq:cross-III}
			&= \EB \langle \nabla M(\x_t-\x^{\star})-\nabla M(\x_{t-a_t}-\x^{\star}),  \PM\sH(\x^{\star}, \xi_{t-1}) \rangle  \\
			& \qquad + \EB \langle \nabla M(\x_{t-a_t}-\x^{\star}), \PM^{a_t+1}\sH(\x^{\star}, \xi_{t-a_t-1})  \rangle.
		\end{split}
	\end{align}
	Let $\bq\ge 1$ be the real number satisfying $\bq^{-1}+\bp^{-1} = 1$ for the given $\bp$.
	By Hölder's inequality,
	\begin{align}
		\label{eq:term3-1}
		|\langle &\nabla M(\x_t-\x^{\star})-\nabla M(\x_{t-a_t}-\x^{\star}),  \PM\sH(\x^{\star}, \xi_{t-1}) \rangle | \nonumber \\
		&\le \| \nabla M(\x_t-\x^{\star})-\nabla M(\x_{t-a_t}-\x^{\star})\|_\bq \|\PM\sH(\x^{\star}, \xi_{t-1}) \|_\bp \nonumber \\
		&\le u_\bp \cdot \| \nabla M(\x_t-\x^{\star})-\nabla M(\x_{t-a_t}-\x^{\star})\|_\bq \|\PM\sH(\x^{\star}, \xi_{t-1}) \|.
	\end{align}
	By~\ref{asmp:smooth-envelop} in Lemma~\ref{lem:envelop}, we have
	\begin{equation}
		\label{eq:term3-1-smooth}
		\| \nabla M(\x_t-\x^{\star})-\nabla M(\x_{t-a_t}-\x^{\star})\|_\bq
		\le (\bp-1)\lambda \cdot \|\x_t-\x_{t-a_t}\|_\bp \le (\bp-1)u_\bp\lambda \cdot \|\x_t-\x_{t-a_t}\|.
	\end{equation}
	
	To proceed the proof, we introduce three useful lemmas in the following.
	The proof of Lemma~\ref{lem:eta-t} can be found in Section~\ref{proof:eta-t}, the proof of  Lemma~\ref{lem:at-x-diff} is deferred to Section~\ref{proof:at-x-diff}, and the proof of Lemma~\ref{lem:sup-h} is in Section~\ref{proof:sup-h}.
	\begin{lem}[Properties of $a_t$'s]
		\label{lem:eta-t}
		Define $\{a_t\}_{t \ge 0}$ according to~\eqref{eq:at}. Under Assumption~\ref{asmp:eta},it follows that (i) $a_t = \OM(\log t)$, (ii) $a_t \eta_{t-a_t} \log t = o(1)$ when $t$ goes to infinity, as a result of which, there exists $K > 0$ such that any $t \ge K$, we have
		\[
		M a_t \eta_{t-a_t} \le \log 2,
		\]
		(iii) $\eta_{t-a_t}/\eta_t = \OM(1)$, and (vi) $a_t \le a_{t+1} \le a_t +1$ for any sufficiently large $t$. 
	\end{lem}
	
	\begin{lem}
		\label{lem:at-x-diff}
		With $\{a_t\}_{t \ge 0}$ defined in~\eqref{eq:at}, we introduce 
		\begin{equation}
			\label{eq:h}
			g_{t-1} = \left\{ \begin{array}{cl}
				\sup\limits_{t-a_t \le \tau \le t-1} g(\xi_\tau) &  \ \text{if} \ a_t \ge 1;  \\
				0  & \ \text{if} \ a_t = 0.
			\end{array} \right.
		\end{equation}
		Then under Assumption~\ref{asmp:H},~\ref{asmp:markov-noise},~\ref{asmp:eta} and~\ref{asmp:growth}, for any $t \ge K$,
		\[
		\|\x_t -\x_{t-a_t} \|  \le 6 Ma_t \eta_{t-a_t} ( \|\x_t\|  +g_{t-1})\le 2( \|\x_t\|  + g_{t-1}) .
		\]
	\end{lem}
	
	\begin{lem}
		\label{lem:sup-h}
		Under Assumption~\ref{asmp:growth}, we have 
		$ \EB g_{t-1} \le (\EB g_{t-1}^\frac{p}{2})^{\frac{2}{p}} = \OM (a_t)$ where $\OM(\cdot)$ hides the linear dependence on $\sup_{t \ge 0} (\EB |g(\xi_t)|^{\frac{p}{2}})^{\frac{2}{p}}$.
	\end{lem}
	
	It then follows that for any $t \ge K$,
	\begin{align} 
		\label{eq:term3-3}
		|\langle &\nabla M(\x_t-\x^{\star})-\nabla M(\x_{t-a_t}-\x^{\star}),  \PM\sH(\x^{\star}, \xi_{t-1}) \rangle | \nonumber \\
		&\overset{(a)}{\le} (\bp-1)u_\bp^2\lambda \cdot  \|\x_t-\x_{t-a_t}\|  \|\PM\sH(\x^{\star}, \xi_{t-1}) \| \nonumber \\
		&\overset{(b)}{\le} 6 M(\bp-1)u_\bp^2\lambda \cdot a_t \eta_{t-a_t} ( \|\x_t-\x^{\star}\| + \|\x^{\star}\|  +g_{t-1}) \|\PM\sH(\x^{\star}, \xi_{t-1}) \| \nonumber \\
		&\overset{(c)}{\le} 6 \sigma M(\bp-1)u_\bp^2\lambda \cdot a_t \eta_{t-a_t} ( \|\x_t-\x^{\star}\| + \|\x^{\star}\|  +g_{t-1})\nonumber \\
		&\overset{(d)}{\le} 6 \sigma M(\bp-1)u_\bp^2\lambda \cdot a_t \eta_{t-a_t} \left( \frac{1}{2}\|\x_t-\x^{\star}\| ^2 + 1 + \|\x^{\star}\|  +g_{t-1}\right)\nonumber \\
		&\overset{(e)}{\le} 6 \sigma M(\bp-1)u_\bp^2\lambda \cdot a_t \eta_{t-a_t} \left( \left(1+\frac{\lambda}{l_\bp^2}\right) M(\x_t-\x^{\star}) + \|\x^{\star}\|  +g_{t-1} + 1\right),
		%	&\le 3 M(\bp-1)u_\bp^2\lambda \cdot a_t \eta_{t-a_t}  \left(  2\left(1+\frac{\lambda}{l_\bp^2}\right) M(\x_t-\x^{\star}) + 2u_*^2\sigma^2+ \|\x^{\star}\|^2 + 2\sigma h_{t-1} \right),
	\end{align}
	where $(a)$ follows from~\eqref{eq:term3-1} and~\eqref{eq:term3-1-smooth}, $(b)$ uses Lemma~\ref{lem:at-x-diff}, $(c)$ uses $\|\PM \sH(\x^{\star}, \xi_{t-1})\| \le \sigma$ from Assumption~\ref{asmp:noise}, $(d)$ uses $x \le \frac{x^2 +1}{2}$ for any $x \in \RB$, and $(e)$ uses~\ref{asmp:appro-envelop} in Lemma~\ref{lem:envelop}.
	
	Notice that $\0$ is the unique minimizer of the smooth function $M(\cdot)$, which implies $\nabla M(\0) = \0$.
	Similarly, we have 
	\begin{align}
		\label{eq:term3-4}
		| \langle &\nabla M(\x_{t-a_t}-\x^{\star}), \PM^{a_t+1}\sH(\x^{\star}, \xi_{t-a_t-1})  \rangle| \nonumber \\
		&\le (\bp-1)u_\bp^2\lambda \cdot \|\x_{t-a_t}-\x^{\star}\| \|\PM^{a_t+1}\sH(\x^{\star}, \xi_{t-a_t-1}) \| \nonumber\\
		&\overset{(a)}{\le} \eta_t (\bp-1)u_\bp^2\lambda \cdot \|\x_{t-a_t}-\x^{\star}\| \nonumber \\
		&\le \eta_t (\bp-1)u_\bp^2\lambda \cdot \left(\|\x_{t-a_t}-\x_t \| + \|\x_t-\x^{\star}\|\right) \nonumber \\
		&\overset{(b)}{\le} \eta_t (\bp-1)u_\bp^2\lambda \cdot \left(2\|\x_t\| +2g_{t-1}+ \|\x_t-\x^{\star}\|\right) \nonumber \\
		&\le \eta_t (\bp-1)u_\bp^2\lambda \cdot \left( 3\|\x_t-\x^{\star}\| + 2(\|\x^{\star}\|+g_{t-1})\right) \nonumber \\
		&\le \eta_t (\bp-1)u_\bp^2\lambda \cdot \left( \frac{3}{2}\|\x_t-\x^{\star}\|^2 + \frac{3}{2} +2(\|\x^{\star}\| + g_{t-1}) \right) \nonumber \\
		&\overset{(c)}{\le} 3\eta_t (\bp-1)u_\bp^2\lambda \cdot \left(\left(1+\frac{\lambda}{l_\bp^2}\right) M(\x_t-\x^{\star}) +(\|\x^{\star}\|+g_{t-1}+1)\right),
	\end{align}
	where $(a)$ follows from~\eqref{eq:a_t-H}, $(b)$ uses Lemma~\ref{lem:at-x-diff} and $(c)$ uses~\ref{asmp:appro-envelop} in Lemma~\ref{lem:envelop}.
	
	Combining~\eqref{eq:cross-III},~\eqref{eq:term3-3} and~\eqref{eq:term3-4}, we have for any $t \ge K$,
	\begin{align*}
		|\EB III |
		\le 3(\bp-1)u_\bp^2\lambda&\left[\left(\eta_t +2 M  \sigma a_t \eta_{t-a_t}\right)  \left(1+\frac{\lambda}{l_\bp^2}\right)\EB M(\x_t-\x^{\star}) \right.\\
		&\quad \left.   + (\eta_t + 2 M \sigma a_t \eta_{t-a_t} )(\EB g_{t-1} + \|\x^{\star}\|+1)
		\right].
	\end{align*}
	
	\paragraph{Putting them together}
	Plugging the bounds for $\EB I, \EB II, \EB III$ into~\eqref{eq:M-cross} and combing the resulting inequality with~\eqref{eq:M-recur} and~\eqref{eq:M-quadratic}, we have for any $t \ge K$,
	\begin{align}
		\begin{split}
			\label{eq:M-final}
			\EB M(\x_{t+1}-\x^{\star}) &\le (1+ A_1 \eta_t^2+A_2 a_t\eta_t\eta_{t-a_t}-A_3 \eta_t )\EB M(\x_{t}-\x^{\star}) \\
			& \qquad + A_4  \eta_t^2 + A_5a_t\eta_t \eta_{t-a_t} + (A_6 \eta_t^2 +A_7  a_t \eta_t \eta_{t-a_t} )\EB g_{t-1},  
		\end{split}
	\end{align}
	where for short we denote 
	\begin{gather*}
		A_1 = (\bp-1) u_\bp^2 \lambda \left(3+2L_H^2\right)  \left(  \frac{\lambda}{l_\bp^2}+1\right),  \
		A_2 = 6M\sigma(\bp-1)u_\bp^2\lambda\left(  \frac{\lambda}{l_\bp^2}+1\right),\\
		A_3 = 2c \left( 1- \gamma  \frac{ u_\bp\sqrt{l_\bp^2+\lambda}}{l_\bp\sqrt{u_\bp^2+\lambda}} \right), \
		A_4 = u_\bp^2(\bp-1) \lambda \left(  \sup_{t \ge 0} \EB \|\sH(\x^{\star}, \xi_t)\|^2
		+ 3(\|\x^{\star}\| +1)
		\right),\\
		A_5 =6M \sigma (\bp-1)u_\bp^2\lambda\left(1+ \|\x^{\star}\|\right), \
		A_6 = 3(\bp-1)u_\bp^2\lambda, \ 
		A_7 = 6M(\bp-1)u_\bp^2 \sigma\lambda.
	\end{gather*}
	Pay attention that by setting $\lambda$ sufficiently small, we can ensure all $A_i$'s are positive.

	Dividing~\eqref{eq:M-final} by $a_t^2 \eta_t$ and simplifying the inequality, we arrive at
	\begin{align*}
		(1+o(\eta_t)) \cdot  \frac{\EB M(\x_{t+1}-\x^{\star})}{a_{t+1}^2 \eta_{t+1}} 
		&\le(1+ A_1 \eta_t^2+A_2 a_t\eta_t\eta_{t-a_t}-A_3 \eta_t ) \frac{\EB M(\x_{t}-\x^{\star})}{a_t^2 \eta_t} + \OM(\eta_t)
	\end{align*}
	where we use $\eta_{t+1} = \eta_t(1+o(\eta_t))$, $1 \le a_t \le a_{t+1}$ and $\eta_{t-a_t}/\eta_t = OM(1)$ in Lemma~\ref{lem:eta-t}, and $\EB g_{t-1} = \OM(a_t)$ in Lemma~\ref{lem:sup-h}.
	As long as $t$ is sufficiently large, we have $\frac{1+ A_1 \eta_t^2+A_2 a_t\eta_t\eta_{t-a_t}-A_3 \eta_t}{1+o(\eta_t)} \le 1- B_1 \eta_t$ and there exist a constant positive $B_2 > 0$ such that
	\[
	\frac{\EB M(\x_{t+1}-\x^{\star}) }{a_{t+1}^2\eta_{t+1}}
	\le \left(1 - B_1 \eta_t \right)\frac{\EB M(\x_{t}-\x^{\star}) }{a_t^2\eta_{t} }+  B_2 \eta_t.
	\]
	Using the last inequality and Lemma A.10 in~\citet{su2018uncertainty}, we have
	\[
	\sup_{t \ge 0} \frac{\EB M(\x_{t}-\x^{\star}) }{a_t^2\eta_{t} } < \infty.
	\]
	By~\ref{asmp:appro-envelop} in Lemma~\ref{lem:envelop}, $\EB M(\x_{t}-\x^{\star})$ approximates $\EB\|\x_t-\x^{\star}\|^2$ up to constant factors.
	It implies $\sup_{t \ge 0} \frac{\EB \|\x_{t}-\x^{\star}\|^2}{\eta_{t} } < \infty$ and thus we establish the $(L^2, a_t\sqrt{\eta_t})$-consistency of $\{\x_t\}_{t \ge 0}$.

	\subsection{Establishment of $(L^p, a_t\sqrt{\eta_t})$-consistency}
	In this subsection, we further establish the $(L^p, a_t\sqrt{\eta_t})$-consistency.
	Though the main idea is similar to the case of $(L^2, a_t\sqrt{\eta_t})$-consistency, the proof procedure is much more circuitous for the following two reasons.
	\begin{enumerate}
		\item First, following the spirit of the generalized Lyapunov approach, we should consider the recursion of the form $\EB M(\x_{t+1} - \x^{\star})^{\frac{p}{2}}$ where  $\x_{t+1}$ is updated according to~\eqref{eq:M-recur}.
		However, $\EB M(\x_{t+1} - \x^{\star})^{\frac{p}{2}}$ doesn't has a close-form expansion as the square counterpart $\EB M(\x_{t+1} - \x^{\star})$.
		We then have to bound the incremental growth of $\EB M(\x_{t+1} - \x^{\star})^{\frac{p}{2}}$ with respect to $\EB M(\x_{t} - \x^{\star})^{\frac{p}{2}}$ via inequalities. To that end, we derive Lemma~\ref{lem:A-x-bound} whose proof is in Section~\ref{proof:A-x-bound}.
		\begin{lem}
			\label{lem:A-x-bound}
			For any scalar $A>0$ and any real number $x\ge -A$, we have
			\begin{equation}
				\label{eq:help-ineq1}
				(A+x)^{1+\alpha} \le 
				\left\{  \begin{array}{ll}
					A^{1+\alpha} + (1+\alpha)A^{\alpha}x + |x|^{1+\alpha}  & \ \text{if} \ \alpha \in (0, 1] \\
					A^{1+\alpha} + (1+\alpha)A^{\alpha}x + \frac{c_{\alpha}(1+\alpha)}{2}A^{\alpha-1}x^2    + c_{\alpha} |x|^{1+\alpha}  & \ \text{if} \ \alpha \in [1, \infty).
				\end{array}
				\right.
			\end{equation}
			where $c_\alpha$ in a universal constant depending $\alpha$ and satisfying $\alpha \le c_\alpha \le 3^\alpha$.
		\end{lem}
		\item Second, according to~\eqref{eq:help-ineq1}, the specific value of $\alpha$ would affect the inequality we use.
		It implies we should proceed the proof in two cases.
	\end{enumerate}
	
	Now, we formally start the proof.
	By~\eqref{eq:M-recur}, we obtain $	M(\x_{t+1}-\x^{\star}) 
	\le M(\x_t-\x^{\star}) - \eta_t  \delta_t $ where
	\begin{equation}
		\label{eq:delta}
		\delta_t := 
		\langle \nabla M(\x_t-\x^{\star}),  \sH(\x_t, \xi_t) \rangle - \frac{(\bp-1)\lambda\eta
			_t}{2} \|\sH(\x_t, \xi_t) \|_\bp^2.
	\end{equation}
	It is clear that $M(\x_t-\x^{\star}) - \eta_t  \delta_t \ge M(\x_{t+1}-\x^{\star})  \ge 0$.
	In the following, we set $\alpha = \frac{\udp}{2}-1$ for short and have $\alpha > 0$ by assumption.

	\paragraph{For the case of $\alpha \in (0, 1]$}
	Taking $(1+\alpha)$-th order moment and using the first scalar inequality in~\eqref{eq:help-ineq1}, we have
	\begin{align}
		\label{eq:help2}
		\EB	M(\x_{t+1}-\x^{\star})^{1+\alpha}
		\le 	\EB	M(\x_{t}-\x^{\star})^{1+\alpha} - (1+\alpha) \eta_t \EB M(\x_{t}-\x^{\star})^{\alpha} \delta_t + \eta_t^{1+\alpha} \EB |\delta_t|^{1+\alpha}.
	\end{align}
	
	To analyze the second and third term in~\eqref{eq:help2}, we establish corresponding upper bounds in Lemma~\ref{lem:p-cross-term} and Lemma~\ref{lem:p-quadratic-term}.
	Their proofs are deferred in Section~\ref{proof:p-cross-term} and Section~\ref{proof:p-quadratic-term} respectively.
	
	\begin{lem}
		\label{lem:p-cross-term}
		Let $d_t = \max_{t-a_t \le \tau \le t}  \EB M(\x_{\tau}-\x^{\star})^{1+\alpha} $.
		There exists a constant $A_8 > 0$ such that
		\[
		\EB M(\x_{t}-\x^{\star})^{\alpha} \delta_t  \ge A_3 \EB M(\x_t-\x^{\star})^{1+\alpha} - A_8 (\eta_t +a_t \eta_{t-a_t} )\left( d_t + a_t \cdot d_t^{\frac{\alpha}{1+\alpha}} \right).
		\]
		Here $A_8$ depends on $A_1, A_2, A_5, A_6, \{\eta_t\}_{t \ge 0}$ and $\sup_{t \ge 0} \EB \|\sH(\x^{\star}, \xi_t)\|^p$.
	\end{lem}

	\begin{lem}
		\label{lem:p-quadratic-term}
		With $\delta_t$ defined in~\eqref{eq:delta}, there exists a constant $A_9 > 0$ such that
		\[
		\EB |\delta_t|^{1+\alpha} \le A_9(\EB M(\x_t-\x^{\star})^{1+\alpha} + \eta_t^{1+\alpha}).
		\]
		Here $A_9$ depends on $\bp, \lambda, u_{\bp}, L_H$ and $\sup_{t \ge 0} \EB \|\sH(\x^{\star}, \xi_t)\|^p$.
	\end{lem}

	Denote $v_t = \EB M(\x_{t}-\x^{\star})^{1+\alpha}$.
	With $d_t$ defined in Lemma~\ref{lem:p-cross-term}, we have $v_t \le d_t$ by definition.
	Plugging the bounds in Lemma~\ref{lem:p-cross-term} and Lemma~\ref{lem:p-quadratic-term} into~\eqref{eq:help2}, we have
	\[
	v_{t+1}
	\le \left( 1- (1+\alpha) A_3 \eta_t  \right)  v_t + (1+\alpha) A_8\eta_t (\eta_t +a_t \eta_{t-a_t} )\left( d_t + a_t \cdot d_t^{\frac{\alpha}{1+\alpha}}\right) +  A_9\eta_{t}^{1+\alpha}(v_t+ \eta_t^{1+\alpha}).
	\]
	We define $\td_t  = {d_t} a_t^{-2(1+\alpha)} \eta_t^{-(1+\alpha)}$ and similarly $\tv_t  = {v_t}a_t^{-2(1+\alpha)} \eta_t^{-(1+\alpha)}$.
	For sufficiently large $t$, we would have $1- (1+\alpha) A_3 \eta_t  \in (0, 1)$.
	Dividing $\eta_t^{1+\alpha} a_t^{2(1+\alpha)} $ on the both sides of the last inequality and using $\eta_{t+1} = \eta_t(1+o(\eta_t))$ and $1 \le a_t \le a_{t+1}$, we arrive at
	\begin{align}
		\tv_{t+1} (1+o(\eta_t))
		& \le \left[1 - (1+\alpha) A_3 \eta_t + (1+\alpha) A_8 \eta_t(\eta_t + a_t \eta_{t-a_t}) + A_9 \eta_t^{1+\alpha}
		\right] \td_t   \nonumber \\
		& \qquad + (1+\alpha) A_8 \eta_t ( 1 + a_t \eta_{t-a_t}/\eta_t ) a_t^{-1} \td_t^{\frac{\alpha}{1+\alpha}} + A_9 \eta_t^{1+\alpha} \nonumber \\
		&\le \left[1 - (1+\alpha) A_3 \eta_t(1+o(\eta_t)) \right] \td_t + \OM(\eta_t) \cdot \td_t^{\frac{\alpha}{1+\alpha}}  + A_9 \eta_t^{1+\alpha}		\label{eq:help3}
	\end{align}
	where the last equality uses $ a_t \eta_{t-a_t} = o(1)$ and $\eta_{t-a_t}/\eta_t  = \OM(1)$ in Lemma~\ref{lem:eta-t}.

	We assert that 
	\[
	\sup_{t \ge 0}\td_{t} < \infty.
	\]
	We prove this statement in the following.
	For sufficiently large $t$, we have that $0 < \frac{1- (1+\alpha) A_3 \eta_t }{1 + o(\eta_t)} \le 1- B_1 \eta_t < 1$ for some constant $B_1 > 0$.
	Then we can find constants $B_2, B_3 > 0$ and simplify~\eqref{eq:help3} as
	\begin{eqnarray}
		\label{eq:help4}
		\tv_{t+1} \le (1-B_1 \eta_t)  \td_t   + B_2  \eta_t \td_t^{\frac{\alpha}{1+\alpha}}+ B_3 \eta_t =: \td_t - \eta_t h( \td_t)
	\end{eqnarray}
	where $h(x) = B_1 x - B_2 x^{\frac{\alpha}{1+\alpha}} - B_3$ is a helper function.
	One can show that $h(x)$ is a function defined on $[0, \infty)$ that starts from a negative value, then decreases, and finally increases to infinity.
	As a result, there is a unique root $x^{\star} > 0$ such that $h(x^{\star}) = 0$.
	With a sufficiently large $t$, one has $a_t \le a_{t+1} \le a_t +1$ from Lemma~\ref{lem:eta-t}.
	If $\td_t \ge x^{\star}$, we then have  $h(\td_t) \ge 0$ and thus $\tv_{t+1} \le \td_t$ from~\eqref{eq:help4}.
	As a result of the fact $t+1 - a_{t+1} \ge t - a_t$, we have
	\[
	\td_{t+1} =  \max_{t+1-a_{t+1} \le \tau \le t+1} \tv_{t} \le  \max_{t-a_{t} \le \tau \le t+1} \tv_{t}
	= \max \left\{
	\max_{t-a_{t} \le \tau \le t} \tv_{t},  \tv_{t+1}
	\right\} = \max \left\{
	\td_t, \tv_{t+1}
	\right\} \le \td_t.
	\]
	In short, once $\td_t \ge x^{\star}$, $\td_{t+1}$ decreases until it is smaller than $x^{\star}$.
	In this way, $\td_t$ is impossible to reach infinity, and thus $\sup_{t \ge 0} \td_t < \infty$.
	
	Given $\sup_{t \ge 0} \td_t < \infty$ and $\frac{p}{2}=1+\alpha$, we have that $\EB M(\x_t-\x^{\star})^{\frac{p}{2}} \le C_p \eta_t^{\frac{p}{2}} a_t^{p}$ uniformly for $t \ge 0$ and a universal constant $C_p > 0$.
	By Lemma~\ref{lem:envelop}, we have $\|\x_t-\x^{\star}\|^2 \precsim M(\x_t-\x^{\star})$.
	As a result, we have $\EB\|\x_t-\x^{\star}\|^p \le C_p \eta_t^{\frac{p}{2}} a_t^{p}$ (by slightly abusing the notation $C_p$).

	\paragraph{For the case of $\alpha \in (1, \infty)$}
		Taking $(1+\alpha)$-th order moment and using the second scalar inequality in~\eqref{eq:help-ineq1}, we have
	\begin{align}
		\label{eq:help5}
		\begin{split}
					\EB	M(\x_{t+1}-\x^{\star})^{1+\alpha}
			&\le 	\EB	M(\x_{t}-\x^{\star})^{1+\alpha} - (1+\alpha) \eta_t \EB M(\x_{t}-\x^{\star})^{\alpha} \delta_t \\
			& \qquad  + \frac{c_{\alpha}(1+\alpha)}{2} M(\x_t-\x^{\star})^{\alpha -1} \eta_t^2 |\delta_t|^2 + c_{\alpha} \eta_t^{1+\alpha} \EB |\delta_t|^{1+\alpha}.
		\end{split}
	\end{align}

Because most of the terms in~\eqref{eq:help5} have been analyzed previously, we only focus on the remaining term $\EB M(\x_t-\x^{\star})^{\alpha -1} |\delta_t|^2$.
We provide an upper bound for it in Lemma~\ref{lem:p-cross-quadratic-term} whose proof is collected in Section~\ref{proof:p-cross-quadratic-term}.

\begin{lem}
	\label{lem:p-cross-quadratic-term}
	There exists a positive constant $A_{10} > 0$ such that 
	\begin{align*}
	\EB M(\x_t-\x^{\star})^{\alpha -1} |\delta_t|^2 
	&\le A_{10} \left[
	\EB M(\x_t-\x^{\star})^{\alpha +1 }  + \left( \EB M(\x_t-\x^{\star})^{1+ \alpha} \right)^{\frac{\alpha}{\alpha+1}}  + \eta_t^2 (\EB M(\x_{t}-\x^{\star})^{1+\alpha})^\frac{\alpha-1}{\alpha+1}\right].
	\end{align*}
Here $A_{10}$ depends on $L_H, M, \|\x^{\star}\|, \lambda, l_{\bp}, \sup_{t \ge 0} \EB \|\sH(\x^{\star}, \xi_t)\|^p$ and $\sup_{t \ge 0} \EB|g(\xi_t)|^{p}$.
\end{lem}
Plugging these bounds in Lemma~\ref{lem:p-cross-term}, Lemma~\ref{lem:p-quadratic-term}, and Lemma~\ref{lem:p-cross-quadratic-term} into~\eqref{eq:help5}, we have
\begin{align*}
v_{t+1}
&\le \left( 1- (1+\alpha) A_3 \eta_t  \right)  v_t + (1+\alpha) A_8\eta_t (\eta_t +a_t \eta_{t-a_t} )\left( d_t + a_t \cdot d_t^{\frac{\alpha}{1+\alpha}}\right)  \\
& \qquad + (1+\alpha)c_{\alpha} A_{10} \eta_t^2 \left[  v_{t} + v_{t}^{\frac{\alpha}{1+\alpha}} + \eta_t^2  v_{t}^{\frac{\alpha-1}{1+\alpha}} \right] + c_\alpha A_9\eta_{t}^{1+\alpha}(v_t+ \eta_t^{1+\alpha}).
\end{align*}
Recall that $\td_t  = {d_t} a_t^{-2(1+\alpha)} \eta_t^{-(1+\alpha)}$ and $\tv_t  = {v_t}a_t^{-2(1+\alpha)} \eta_t^{-(1+\alpha)}$.
For simplicity, we let $\OM(\cdot)$ hide positive constant factors.
Then, dividing $\eta_t^{1+\alpha} a_t^{2(1+\alpha)} $ on the both sides of the last equation and using $\eta_{t+1} = \eta_t(1+o(\eta_t))$ and $1 \le a_t \le a_{t+1}$, we arrive at
\begin{align}
	\tv_{t+1} (1+o(\eta_t))
	& \le \left[1 - (1+\alpha) A_3 \eta_t + \OM(\eta_t) \cdot (\eta_t + a_t \eta_{t-a_t}) + \OM ( \eta_t^{1+\alpha})
	\right] \td_t   \nonumber \\
	& \qquad + \OM(\eta_t) \cdot  ( 1 + a_t \eta_{t-a_t}/\eta_t ) a_t^{-1} \td_t^{\frac{\alpha}{1+\alpha}} + \OM(\eta_t^2) \cdot \td_t^{\frac{\alpha-1}{\alpha+1}} + \OM ( \eta_t^{1+\alpha}) \nonumber \\
	&\overset{(a)}{\le} \left[1 - (1+\alpha) A_3 \eta_t(1+o(\eta_t)) \right] \td_t + \OM(\eta_t) \cdot \td_t^{\frac{\alpha}{1+\alpha}}  + \OM(\eta_t^2) \cdot \td_t^{\frac{\alpha-1}{\alpha+1}} + \OM ( \eta_t^{1+\alpha}) \nonumber \\
	&\overset{(b)}{\le} \left[1 - (1+\alpha) A_3 \eta_t(1+o(\eta_t)) \right] \td_t + \OM(\eta_t) \cdot \td_t^{\frac{\alpha}{1+\alpha}}  + \OM ( \eta_t^{1+\alpha}) 
\end{align}
where $(a)$ uses $ a_t \eta_{t-a_t} = o(1)$ and $\eta_{t-a_t}/\eta_t  = \OM(1)$ in Lemma~\ref{lem:eta-t} and $(b)$ follows because we can assume $\td_{t} \ge 1$ without loss of generality (which can be achieved by redefine $\td_{t} \gets \max \{\td_t, 1 \}$).

For sufficiently large $t$, we can find positive constants $B_1, B_2, B_3 > 0$ such that 
\[
	\tv_{t+1} \le (1-B_1 \eta_t) \td_{t} + B_2 \eta_t \td_{t}^{\frac{\alpha}{\alpha+1}} + B_3 \eta_t,
\]
which is the inequality we have already analyzed in~\eqref{eq:help4}.
By an identical argument therein, we conclude $\sup_{t \ge 0} \td_t < \infty$.
Therefore, we also have $\EB\|\x_t-\x^{\star}\|^p \le C_p \eta_t^{\frac{p}{2}} a_t^{p}$ when $\alpha > 1$.

\end{proof}

\subsection{Proof of Lemma~\ref{lem:eta-t}}
\label{proof:eta-t}
\begin{proof}[Proof of Lemma~\ref{lem:eta-t}]
	\begin{itemize}
		\item Under Assumption~\ref{asmp:eta}, we have $\eta_t \downarrow 0$ and $t \eta_t \uparrow \infty$ as $t \to \infty$.
		Hence, for any fixed $m>0$, we have $t \eta_t \ge m$ for sufficiently large $t$.
		Then,
		\[
		a_t = \ceil{\log_{\rho} \frac{\eta_t}{\sigma \kappa}} 
		= \ceil{\log_{\frac{1}{\rho}} \frac{\sigma \kappa}{\eta_t}} 
		\le  \ceil{\log_{\frac{1}{\rho}} \frac{\sigma \kappa t}{m}}
		\ \implies  \ a_t = \OM(\log t).
		\]
		\item Since $a_t = \OM(\log t)$, for sufficiently large $t$, there exists $\mu > 0$ such that $a_t \le \mu \log t$ and thus
		\[
		a_t \eta_{t-a_t} \log t \le \mu \log^2 t \cdot \eta_{t - \mu \log t} = 
		\frac{\mu \log^2 t}{\log^2 (t-\mu \log t)} \cdot\eta_{t - \mu \log t}   \log^2 (t-\mu 
		\log t) = o(1),
		\]
		where we use $ \eta_t \log^2 t = o(1)$ when $t$ goes to infinity due to Assumption~\ref{asmp:eta}.
		\item It follows that
		\begin{align*}
			\frac{\eta_{t-a_t}}{\eta_t} =
			\prod_{\tau=t-a_t}^{t-1}	\frac{\eta_{\tau}}{\eta_{\tau+1}}
			= \prod_{\tau=t-a_t}^{t-1} (1+o(\eta_t))
			\le \exp\left( o(1) \sum_{\tau=t-a_t}^{t-1}  \eta_{\tau} \right)
			\le \exp(o(1) a_t \eta_{t-a_t} ) = \OM(1).
		\end{align*}
		\item By $\eta_{t+1} = \eta_t (1+o(\eta_t))$, it follow that 
		\[
		\log_{\frac{1}{\rho}} \frac{\sigma \kappa}{\eta_{t+1}} = 	\log_{\frac{1}{\rho}} \frac{\sigma \kappa(1+o(\eta_t))}{\eta_{t}}
		=	\log_{\frac{1}{\rho}} \frac{\sigma \kappa}{\eta_{t}}  + \log_{\frac{1}{\rho}} (1+o(\eta_t))
		=	\log_{\frac{1}{\rho}} \frac{\sigma \kappa}{\eta_{t}}  + o(\eta_t).
		\]
		For sufficiently large $t$, we will have $o(\eta_t) \le 0.5$ and thus
		\[
		a_{t+1} = \left\lceil \log_{\frac{1}{\rho}} \frac{\sigma \kappa}{\eta_{t+1} } \right\rceil 
		\le \left\lceil \log_{\frac{1}{\rho}} \frac{\sigma \kappa}{\eta_t} \right\rceil  + 1 = a_t + 1.
		\]
		It is clearly that we have $a_t \le a_{t+1}$ due to $\eta_t \downarrow 0$. 
	\end{itemize}
	
\end{proof}

\subsection{Proof of Lemma~\ref{lem:at-x-diff}}
\label{proof:at-x-diff}
\begin{proof}[Proof of Lemma~\ref{lem:at-x-diff}]
	The conclusion is obvious if $a_t = 0$. 
	Without loss of generality, we assume $\rho>0$ and $a_t \ge 1$.
	Recall that the update rule is $\x_{t+1} = \x_t - \eta_t  \sH(\x_t, \xi_t) $.
	Hence, under Assumption~\ref{asmp:growth},
	\[
	|\|\x_{t+1} \| - \| \x_t \| | \le \|\x_{t+1}-\x_t\| = \eta_t \| \sH(\x_t, \xi_t)\| \le M \eta_t (\|\x_t\|+g(\xi_t)),
	\]
	which implies that
	\[
	\|\x_{t+1} \|  \le (1+M\eta_t) \|\x_t\| + M\eta_tg(\xi_t).
	\]
	For simplicity, we denote $\eta_{s, t} := \sum_{l=s}^t \eta_l$ is $s \le t$ otherwise $\eta_{s, t} := 0$ for $s > t$.
	Iterating the last inequality yields for any $t-a_t-1\le \tau 
	\le t-1$ with $t \ge K$,
	\begin{align*}
		\|\x_{\tau+1} \| 
		&\le  \prod_{s=t-a_t}^\tau (1+M\eta_s) \|\x_{t-a_t}\| + M\sum_{s={t-a_t}}^\tau \eta_s g(\xi_s)  \prod_{l=s+1}^\tau (1+M\eta_l)\\
		&\le  \exp\left( M \eta_{t-a_t, \tau} \right) \|\x_{t-a_t}\| + M\sum_{s={t-a_t}}^\tau \eta_s g(\xi_s) \exp\left( M \eta_{s+1, \tau} \right) \\
		&\overset{(a)}{\le}  \exp\left( M a_t \eta_{t-a_t} \right) \left[ \|\x_{t-a_t}\| + M\sum_{s={t-a_t}}^\tau \eta_s g(\xi_s)\right]\\
		& \overset{(b)}{\le}2 \left(\|\x_{t-a_t}\| + Ma_t \eta_{t-a_t} g_{t-1} \right)
	\end{align*}
	where $(a)$ uses $\eta_{t-a_t, \tau}  \le a_t \eta_{t-a_t}$ by definition and $(b)$ uses Lemma~\ref{lem:eta-t} and the definition of $g_{t-1}$ in~\eqref{eq:h}.
	
	As a result,
	\begin{align*}
		\|\x_t -\x_{t-a_t} \| 
		&\le \sum_{\tau=t-a_t}^{t-1} \|\x_{\tau+1}-\x_\tau\|
		\le \sum_{\tau=t-a_t}^{t-1} M \eta_\tau (\|\x_\tau\| + g(\xi_\tau))\\
		&\le \sum_{\tau=t-a_t}^{t-1} M \eta_\tau (2 \|\x_{t-a_t}\| + 2Ma_t \eta_{t-a_t}g_{t-1} ) + M \eta_{t-a_t, t-1}g_{t-1} \\
		&\le 2 M \eta_{t-a_t, t-1} ( \|\x_{t-a_t}\|  +g_{t-1})
		\le 2 M a_t \eta_{t-a_t} ( \|\x_{t-a_t}\|  +g_{t-1})
	\end{align*}
	where the last inequality uses Lemma~\ref{lem:eta-t} and $ M a_t \eta_{t-a_t} \le \log 2 \le \frac{1}{2}$.
	
	Therefore, using $ \log 2 \le \frac{1}{3}$, we have
	\[
	\|\x_t -\x_{t-a_t} \| 
	\le 2 M a_t \eta_{t-a_t} ( \|\x_{t-a_t}-\x_t\| + \|\x_t\|  +g_{t-1})
	\le \frac{2}{3}\|\x_{t-a_t}-\x_t\|  + 2 M a_t \eta_{t-a_t} ( \|\x_t\|  +g_{t-1})
	\]
	which implies
	\[
	\|\x_t -\x_{t-a_t} \|  \le 6 Ma_t \eta_{t-a_t} ( \|\x_t\|  +g_{t-1}) 
	\le 2( \|\x_t\|  +g_{t-1}) .
	\]
\end{proof}

\subsection{Proof of Lemma~\ref{lem:sup-h}}
\label{proof:sup-h}
\begin{proof}[Proof of Lemma~\ref{lem:sup-h}]
	Our target is to prove
	\[
	\EB \sup_{t-a_t \le\tau \le t-1} |g(\xi_\tau)|
	\le 
	\left(\EB \sup_{t-a_t \le\tau \le t-1} |g(\xi_\tau)|
	^\frac{p}{2}\right)^{\frac{2}{p}} =  \OM (a_t).
	\]
	The left inequality follows from Jensen's inequality.
	We then focus on the right equality.
	
	The fact $p>2$ implies $\frac{2}{p}< 1$.
	Then $(x+y)^\frac{2}{p} \le x^\frac{2}{p}+y^\frac{2}{p}$ for any $x, y \ge 0$.
	Therefore,
	\begin{align*}
		\left(\EB \sup_{t-a_t \le\tau \le t-1} |g(\xi_\tau)|
		^\frac{p}{2}\right)^{\frac{2}{p}} 
		&\le \left(\EB \sum_{t-a_t \le\tau \le t-1} |g(\xi_\tau)|
		^\frac{p}{2}\right)^{\frac{2}{p}}  \\
		&\le \sum_{t-a_t \le\tau \le t-1} \left(\EB|g(\xi_\tau)|
		^\frac{p}{2}\right)^{\frac{2}{p}}
		\le  a_t \cdot \sup_{t \ge 0} \left(\EB|g(\xi_t)|
		^\frac{p}{2}\right)^{\frac{2}{p}} \precsim a_t.
	\end{align*}
	%By the definition in~\eqref{eq:at}, we have $a_t = \OM(\log t)$.
	%Plugging it into the last inequality, we complete the proof.
\end{proof}

\subsection{Proof of Lemma~\ref{lem:A-x-bound}}
\label{proof:A-x-bound}
\begin{proof}[Proof of Lemma~\ref{lem:A-x-bound}]
	By homogeneity, we only need to prove for the case of $A = 1$.
	\begin{itemize}
		\item When $\alpha \in (0,1]$, we let $f(x) = 1+  ({1+\alpha})x + |x|^{1+\alpha}   -  (1+x)^{1+\alpha}$ and its derivative is $f'(x) = (1+\alpha) \left(1+ |x|^{\alpha}\mathrm{sign}(x)- (1+x)^{\alpha}\right)$.
		When $1
		\ge \alpha>0$, we have $(1+x)^{\alpha} \le x^{\alpha} + 1$ for $x \ge 0$ and $1 \le (1-x)^{\alpha}+x^{\alpha}$ for $x \in [0, 1]$.
		It implies that $f'(x)\ge0$ for $x\ge0$ and $f'(x)<0$ for $-1\le x<0$.
		Hence, $f(x) \ge f(0)=0$ for any $x \ge -1$.
		\item When $\alpha \in [1, \infty)$, we let $f(x) = 1+  ({1+\alpha})x  + \frac{c_{\alpha}(1+\alpha)}{2}x^2  +c_{\alpha} |x|^{1+\alpha}   -  (1+x)^{1+\alpha}$ and its derivative is $f'(x) = (1+\alpha) \left[1 + c_{\alpha} (x+ |x|^{\alpha}\mathrm{sign}(x))- (1+x)^{\alpha}\right]$.
		Similarly, we are going to show $f'(x)\ge0$ for $x\ge0$ and $f'(x)<0$ for $-1\le x<0$.
		These two conditions is equivalent to
		\begin{equation*}
			c_{\alpha} \ge \left\{
			\begin{array}{ll}
				\frac{(1+x)^{\alpha}-1}{x+x^\alpha} & \ \text{if} \ 0 \le x < \infty;\\
				\frac{1-(1-x)^{\alpha}}{x+x^\alpha} & \ \text{if}  \ 0 \le x \le 1.
			\end{array}
			\right.		 		
		\end{equation*}
		The last inequality is satisfied when we set
		\[
		c_{\alpha} := \sup_{x \ge 0} \frac{(1+x)^{\alpha}-1}{x+x^\alpha}.
		\]
		We explain the reason in the following.
		Since $(1-x)^{r} \ge 1-rx$ for any $x \in [0, 1]$ and $r \ge 1$, we have $\sup_{x \in [0, 1]} \frac{1-(1-x)^{\alpha}}{x+x^\alpha} \le c_{\alpha} \le \sup_{x \in [0, 1]} \frac{x \alpha }{x+x^\alpha} = c_{\alpha} \le \sup_{x \in [0, 1]} \frac{ \alpha }{1+x^{\alpha-1}} = \alpha$.
		Let $h(x) = \frac{(1+x)^{\alpha}-1}{x+x^\alpha}$, then $c_{\alpha} = \sup_{x \in [0, \infty)} h(x)$.
		One can easily show that, on the interval  $(0, \infty)$, $h(x)$ is a continuous function with $\lim_{x \to 0^+} h(x) = \alpha$ and $\min_{x \to \infty} h(x) = 1$.
		As a result, we know that $\sup_{x \in [0, \infty)} h(x)$ is finite and no smaller than $h(0):=\alpha$.
		
		We complete the proof by showing $c_\alpha \le^\alpha$ in the following.
		If $x \ge 1$, we have
		\[
		\left(\frac{(1+x)^{\alpha}-1}{x+x^\alpha}\right)^{\frac{1}{\alpha}}
		\le 		 		\left(\frac{(1+x)^{\alpha}}{x^\alpha}\right)^{\frac{1}{\alpha}} \le \frac{1+x}{x} \le 2.
		\]
		If $0 \le x \le 1$, using $(1+x)^{\alpha}-1 \le \alpha x (1+x)^{\alpha-1}$, we have that for any $\alpha \ge 1$,
		\[
		\left(\frac{(1+x)^{\alpha}-1}{x+x^\alpha}\right)^{\frac{1}{\alpha}}
		\le \left(\frac{\alpha(1+x)^{\alpha-1}}{1+x^{\alpha-1}}\right)^{\frac{1}{\alpha}} \le (\alpha 2^{\alpha-1})^{\frac{1}{\alpha}} \le 3.
		\]
	\end{itemize}
\end{proof}

\subsection{Proof of Lemma~\ref{lem:p-cross-term}}
\label{proof:p-cross-term}
\begin{proof}[Proof of Lemma~\ref{lem:p-cross-term}]
	The main idea is to decompose $\EB M(\x_{t}-\x^{\star})^{\alpha} \delta_t$ into three terms and then bound each term respectively.
	It follows that
	\begin{align}
		\label{eq:p-cross-term}
		\begin{split}
			\EB M(\x_{t}-\x^{\star})^{\alpha} \delta_t 
			&=  		\EB M(\x_{t}-\x^{\star})^{\alpha}  \langle \nabla M(\x_t-\x^{\star}),   \PM \sH(\x_t, \xi_{t-1}) -  \PM\sH(\x^{\star}, \xi_{t-1})  \rangle  \\
			&\quad + \EB M(\x_{t}-\x^{\star})^{\alpha}  \langle \nabla M(\x_t-\x^{\star}),  \PM\sH(\x^{\star}, \xi_{t-1})  \rangle  \\
			&\quad - \frac{(\bp-1)\lambda\eta
				_t}{2} \cdot \EB M(\x_{t}-\x^{\star})^{\alpha}  \|\sH(\x_t, \xi_t) \|_\bp^2.
		\end{split}
	\end{align}
	\paragraph{For the first term}
	From~\eqref{eq:cross-I} and~\eqref{eq:cross-II}, it follows that
	\begin{equation}
		\label{eq:p-cross-term1}
		\langle \nabla M(\x_t-\x^{\star}),   \PM\sH(\x_t, \xi_{t-1}) -  \PM\sH(\x^{\star}, \xi_{t-1})  \rangle \ge A_3 M(\x_t-\x^{\star}).
	\end{equation}
	\paragraph{For the second term}
	Similar to~\eqref{eq:cross-III}, we have
	\begin{align*}
		|\EB	&M(\x_{t}-\x^{\star})^{\alpha} \langle \nabla M(\x_t-\x^{\star})),  \PM\sH(\x^{\star}, \xi_{t-1}) \rangle |\\
		&\le	|\EB M(\x_{t}-\x^{\star})^{\alpha} \langle \nabla M(\x_t-\x^{\star}))-\nabla M(\x_{t-a_t}-\x^{\star})),  \PM\sH(\x^{\star}, \xi_{t-1}) \rangle| \\
		& \quad +	|\EB	M(\x_{t-a_t}-\x^{\star})^{\alpha}
		\langle \nabla M(\x_{t-a_t}-\x^{\star})),  \PM^{a_t+1}\sH(\x^{\star}, \xi_{t-a_t-1}) \rangle|\\
		& \quad +		|\EB\left(M(\x_{t}-\x^{\star})^{\alpha}-M(\x_{t-a_t}-\x^{\star})^{\alpha}\right)
		\langle \nabla M(\x_{t-a_t}-\x^{\star})),  \PM\sH(\x^{\star}, \xi_{t-1}) \rangle|\\
		& := T_1 + T_2 + T_3.
	\end{align*}
	We are going to analyze the three terms separately.
	By~\eqref{eq:term3-3}, we have
	\begin{align*}
		|\langle &\nabla M(\x_t-\x^{\star})-\nabla M(\x_{t-a_t}-\x^{\star}),  \PM\sH(\x^{\star}, \xi_{t-1}) \rangle |  \\
		& \le 6 \sigma M(\bp-1)u_\bp^2\lambda \cdot a_t \eta_{t-a_t} \left( \left(1+\frac{\lambda}{l_\bp^2}\right) M(\x_t-\x^{\star}) + \|\x^{\star}\|  +g_{t-1} + 1\right),
	\end{align*}
	which implies the first term $T_1$ satisfies 
	\begin{align*}
		T_1 &\precsim a_t \eta_{t-a_t} (\EB M(\x_t-\x^{\star})^{1+\alpha} + \EB M(\x_t-\x^{\star})^{\alpha}(1 + g_{t-1}) )\\
		&\overset{(a)}{\precsim} a_t \eta_{t-a_t} (\EB M(\x_t-\x^{\star})^{1+\alpha} +(1+ (\EB g_{t-1}^{\frac{p}{2}})^{\frac{2}{p}}) (\EB M(\x_t-\x^{\star})^{1+\alpha})^{\frac{\alpha}{1+\alpha}} )\\
		&\overset{(b)}{\precsim} a_t \eta_{t-a_t} (\EB M(\x_t-\x^{\star})^{1+\alpha} + a_t \cdot (\EB M(\x_t-\x^{\star})^{1+\alpha})^{\frac{\alpha}{1+\alpha}} ) ,
	\end{align*}
	where $(a)$ uses Holder's inequality and $2(1+\alpha) = p$ for simplicity and $(b)$ uses $(\EB h_{t-1}^{\frac{p}{2}})^{\frac{2}{p}} \precsim \log t$ due to Lemma~\ref{lem:sup-h}.
	By $(a)$ in~\eqref{eq:term3-4}, we have
	\begin{align*}
		| \langle &\nabla M(\x_{t-a_t}-\x^{\star}), \PM^{a_t+1}\sH(\x^{\star}, \xi_{t-a_t-1})  \rangle|  \\
		&\le \eta_t (\bp-1)u_\bp^2\lambda \cdot \|\x_{t-a_t}-\x^{\star}\| \\
		&\le \eta_t (\bp-1)u_\bp^2\lambda \cdot \frac{\|\x_{t-a_t}-\x^{\star}\|^2 +1}{2}\\
		&\le \eta_t (\bp-1)u_\bp^2\lambda \cdot \left(\left(1+\frac{\lambda}{l_\bp^2}\right) M(\x_{t-a_t}-\x^{\star}) +1\right),
	\end{align*}
	which implies the second term $T_2$ satisfies
	\begin{align*}
		T_2 &\precsim \eta_t (\EB M(\x_{t-a_t}-\x^{\star})^{1+\alpha} + \EB M(\x_{t-a_t}-\x^{\star})^{\alpha} )\\
		&\precsim \eta_t (\EB M(\x_{t-a_t}-\x^{\star})^{1+\alpha} +  (\EB M(\x_{t-a_t}-\x^{\star})^{1+\alpha})^{\frac{\alpha}{1+\alpha}} ).
	\end{align*}
	
	Finally, as for the third term $T_3$, by a similar argument of the last inequality, we have
	\[
	| \langle \nabla M(\x_{t-a_t}-\x^{\star}), \PM\sH(\x^{\star}, \xi_{t-1})  \rangle|  
	\le \sigma(\bp-1)u_\bp^2\lambda \cdot \|\x_{t-a_t}-\x^{\star}\|.
	\]
	On the other hand, noticing that $|\|\x\|_M^{2\alpha} - \|\y\|_M^{2\alpha}|
	\le 2\alpha \|\x-\y\|_M \cdot \max \{ \|\x\|_M,\|\y\|_M\}^{2\alpha-1}$, we have
	\begin{align*}
		|M(\x_{t}-\x^{\star})^{\alpha}-M(\x_{t-a_t}-\x^{\star})^{\alpha}|
		&\le \frac{\alpha}{2^{\alpha-1}} \|\x_t-\x_{t-a_t}\|_M\cdot \max \{ \|\x_{t}-\x^{\star}\|_M,\|\x_{t-a_t}-\x^{\star}\|_M  \}^{2\alpha-1}.
		% 	&\le \frac{\alpha u_{\bp}}{\sqrt{u_{\bp}^2+\lambda}}\|\x_t-\x_{t-a_t}\|\cdot \max \{ M(\x_{t}-\x^{\star})^{\alpha-\frac{1}{2}},M(\x_{t-a_t}-\x^{\star})^{\alpha-\frac{1}{2}}  \}.
	\end{align*}
	As a result, we have
	\begin{align*}
		T_3 &\precsim \EB \|\x_{t-a_t}-\x^{\star}\| \|\x_t-\x_{t-a_t}\|_M\cdot \max \{ \|\x_{t}-\x^{\star}\|_M,\|\x_{t-a_t}-\x^{\star}\|_M\}^{2\alpha-1}\\
		&\precsim \EB \|\x_{t-a_t}-\x^{\star}\|_M \|\x_t-\x_{t-a_t}\|\cdot \max \{ \|\x_{t}-\x^{\star}\|_M,\|\x_{t-a_t}-\x^{\star}\|_M \}^{2\alpha-1}\\
		&\precsim a_t \eta_{t-a_t} \EB (\|\x_t\|+g_{t-1}) \|\x_{t-a_t}-\x^{\star}\|_M\cdot \max \{ \|\x_{t}-\x^{\star}\|_M,\|\x_{t-a_t}-\x^{\star}\|_M \}^{2\alpha-1}\\
		&\precsim a_t \eta_{t-a_t} \EB (\|\x_t\|_M+g_{t-1}) \cdot \max \{ \|\x_{t}-\x^{\star}\|_M,\|\x_{t-a_t}-\x^{\star}\|_M \}^{2\alpha}\\
		&\precsim a_t \eta_{t-a_t} \EB (\max \{ \|\x_{t}-\x^{\star}\|_M,\|\x_{t-a_t}-\x^{\star}\|_M \}+g_{t-1}) \cdot \max \{ \|\x_{t}-\x^{\star}\|_M,\|\x_{t-a_t}-\x^{\star}\|_M \}^{2\alpha}\\
		&\precsim a_t \eta_{t-a_t} \EB (\max \{ \|\x_{t}-\x^{\star}\|_M,\|\x_{t-a_t}-\x^{\star}\|_M \}^2+g_{t-1}+1) \cdot \max \{ \|\x_{t}-\x^{\star}\|_M,\|\x_{t-a_t}-\x^{\star}\|_M \}^{2\alpha}\\
		& \overset{(a)}{\precsim}a_t \eta_{t-a_t} \EB (b_t^2+g_{t-1}+1) \cdot b_t^{2\alpha}
		\precsim a_t \eta_{t-a_t}  \left[ \EB b_t^{2(1+\alpha)}+ \EB(g_{t-1}+1)  b_t^{2\alpha} \right] \\
		&\overset{(b)}{\precsim} a_t \eta_{t-a_t} \left[ \EB b_t^{2(1+\alpha)}+ (1+ (\EB g_{t-1}^{\frac{p}{2}})^{\frac{2}{p}}) (\EB b_t^{2(1+\alpha)})^{\frac{\alpha}{1+\alpha}} \right] \\
		&\overset{(c)}{\precsim} a_t \eta_{t-a_t} \left( \EB b_t^{2(1+\alpha)}+ a_t \cdot (\EB b_t^{2(1+\alpha)})^{\frac{\alpha}{1+\alpha}}\right)\\
		&\overset{(d)}{\precsim} a_t \eta_{t-a_t} \left( d_t + a_t \cdot d_t^{\frac{\alpha}{1+\alpha}}\right),
	\end{align*}
	where $(a)$ follows the notation $b_t = \max \{ \|\x_{t}-\x^{\star}\|_M,\|\x_{t-a_t}-\x^{\star}\|_M \}$, $(b)$ uses Holder's inequality and $2(1+\alpha) = p$, $(c)$ uses $(\EB h_{t-1}^{\frac{p}{2}})^{\frac{2}{p}} \precsim a_t$ due to Lemma~\ref{lem:sup-h}, and $(d)$ uses the notation $d_t := \max_{t-a_t \le \tau \le t}  \EB M(\x_{\tau}-\x^{\star})^{1+\alpha} $ and $d_t \ge\EB b_t^{2(1+\alpha)}$ by definition.
	
	Combing the bounds for $T_1, T_2$ and $T_3$, we have
	\begin{equation}
		\label{eq:p-cross-term2}
		|\EB M(\x_{t}-\x^{\star})^{\alpha} \langle \nabla M(\x_t-\x^{\star})),  \PM\sH(\x^{\star}, \xi_{t-1}) \rangle |
		\precsim a_t \eta_{t-a_t} \left( d_t + a_t \cdot d_t^{\frac{\alpha}{1+\alpha}} \right).
	\end{equation}
	
	\paragraph{For the last term}
	Finally, we analyze the last term of~\eqref{eq:p-cross-term}.
	It follows from Hölder's inequality that
	\begin{align*}
		\EB M(\x_{t}-\x^{\star})^{\alpha}  \|\sH(\x_t, \xi_t) \|_\bp^2
		&\le (\EB M(\x_{t}-\x^{\star})^{1+\alpha})^\frac{\alpha}{1+\alpha}
		(\EB  \|\sH(\x_t, \xi_t) \|_\bp^{2(1+\alpha)})^\frac{1}{1+\alpha}\\
		&\precsim (\EB M(\x_{t}-\x^{\star})^{1+\alpha})^\frac{\alpha}{1+\alpha}
		(\EB  \|\sH(\x_t, \xi_t) \|^{2(1+\alpha)})^\frac{1}{1+\alpha}\\
		&
		\precsim (\EB M(\x_{t}-\x^{\star})^{1+\alpha})^\frac{\alpha}{1+\alpha}	(\EB \PM \|\sH(\x_t, \xi_{t-1}) \|^{\udp})^\frac{1}{1+\alpha}.
	\end{align*}
	By Assumption~\ref{asmp:H} and~\ref{asmp:noise}, we have
	\begin{align}
		\label{eq:help1}
		\EB \PM \|\sH(\x_t, \xi_{t-1}) \|^{\udp} 
		&\precsim \EB \PM \|\sH(\x_t, \xi_{t-1}) -\sH(\x^{\star}, \xi_{t-1}) \|^{\udp} +  \EB \PM \|\sH(\x^{\star}, \xi_{t-1}) \|^{\udp}  \nonumber \\
		&\precsim \EB \PM \|\sH(\x_t, \xi_{t-1}) -\sH(\x^{\star}, \xi_{t-1}) \|^{\udp} +  \sup_{t \ge 0}\EB\|\sH(\x^{\star}, \xi_{t}) \|^{\udp}  \nonumber \\
		&\precsim \EB \|\x_t-\x^{\star}\|^\udp + 1
		\precsim \EB M(\x_{t}-\x^{\star})^{1+\alpha} + 1.
	\end{align}
	Using $(x+1)^{\frac{1}{1+\alpha}} \le x^{\frac{1}{1+\alpha}} +1$ for $x \ge0$, we have
	\begin{equation}
		\label{eq:p-cross-term3}
		\EB M(\x_{t}-\x^{\star})^{\alpha}  \|\sH(\x_t, \xi_t) \|_\bp^2
		\precsim \EB M(\x_{t}-\x^{\star})^{1+\alpha}	+(\EB M(\x_{t}-\x^{\star})^{1+\alpha})^\frac{\alpha}{1+\alpha}.
	\end{equation}
	
	Plugging~\eqref{eq:p-cross-term1},~\eqref{eq:p-cross-term2} and~\eqref{eq:p-cross-term3} into~\eqref{eq:p-cross-term}, we complete the proof.
\end{proof}

\subsection{Proof of Lemma~\ref{lem:p-quadratic-term}}
\label{proof:p-quadratic-term}
\begin{proof}[Proof of Lemma~\ref{lem:p-quadratic-term}]
	By the definition of $\delta_t$, it follows that
	\begin{align*}
		\EB|\delta_t|^{1+\alpha}
		\precsim \EB | \langle \nabla M(\x_t-\x^{\star}),  \sH(\x_t, \xi_t) \rangle|^{1+\alpha} + \eta_t^{1+\alpha} \EB\|\sH(\x_t, \xi_t) \|_\bp^{2(1+\alpha)}
	\end{align*}
	For one thing, by Hölder's inequality, we have 
	\begin{align*}
		\EB | \langle \nabla M(\x_t-\x^{\star}),  \sH(\x_t, \xi_t) \rangle|^{1+\alpha}
		&\le \EB \|\nabla M(\x_t-\x^{\star})\|_\bq^{1+\alpha} \cdot \| \sH(\x_t, \xi_t) \|_\bp^{1+\alpha}\\
		&\precsim  \EB\|\nabla M(\x_t-\x^{\star})\|_\bq^{2(1+\alpha)} + \EB  \| \sH(\x_t, \xi_t) \|_\bp^{2(1+\alpha)}.
	\end{align*}
	Since $M(\x)$ is smooth w.r.t. the norm $\|\cdot\|_\bp$ (due to~\ref{asmp:smooth-envelop} in Lemma~\ref{lem:envelop}) and $\nabla M(\0)=\0$, we have
	\[
	\EB\|\nabla M(\x_t-\x^{\star})\|_\bq^{2(1+\alpha)}
	=  \EB\|\nabla M(\x_t-\x^{\star})\|_\bq^\udp
	\precsim  \EB\|\x_t-\x^{\star}\|_\bp^\udp
	\precsim  \EB\|\x_t-\x^{\star}\|^\udp
	\precsim  \EB M(\x_t-\x^{\star})^{1+\alpha},
	\]
	where the last inequality uses the fact $\|\cdot\|$ is equivalent to $\|\cdot\|_M$ up to constant factors and $M(\x) = \frac{1}{2}\|\x\|_M^2$.
	For another thing,
	\begin{align*}
		\EB\|\sH(\x_t, \xi_t) \|_\bp^{2(1+\alpha)}
		&\precsim 	\EB\|\sH(\x_t, \xi_t) \|^{2(1+\alpha)} = \EB\PM\|\sH(\x_t, \xi_{t-1}) \|^{\udp} \\
		&\precsim \EB M(\x_t-\x^{\star})^{1+\alpha} + 1,
	\end{align*}
	where the last inequality follows from~\eqref{eq:help1}.
	
	Putting two pieces together, we have
	\[
	\EB|\delta_t|^{1+\alpha}
	\precsim \EB M(\x_t-\x^{\star})^{1+\alpha} + \eta_t^{1+\alpha}.
	\]
\end{proof}

\subsection{Proof of Lemma~\ref{lem:p-cross-quadratic-term}}
\label{proof:p-cross-quadratic-term}
\begin{proof}[Proof of Lemma~\ref{lem:p-cross-quadratic-term}]
	By definition of $\delta_t$ in~\eqref{eq:delta}, it follows that
	\[
	|\delta_t|^2 \le 2 |\langle \nabla M(\x_t-\x^{\star}),  \sH(\x_t, \xi_t) \rangle |^2 + 
	\frac{(\bp-1)^2\lambda^2\eta_t^2}{2} \|\sH(\x_t, \xi_t) \|_\bp^4,
	\]
	by which, $\EB M(\x_t-\x^{\star})^{\alpha -1} |\delta_t|^2$ can be further divided into two terms
	\begin{align*}
		\EB M(\x_t-\x^{\star})^{\alpha -1} |\delta_t|^2 
		&\le 2 \EB M(\x_t-\x^{\star})^{\alpha -1}|\langle \nabla M(\x_t-\x^{\star}),  \sH(\x_t, \xi_t) \rangle |^2  \\
		& \qquad + \frac{(\bp-1)^2\lambda^2\eta
			_t^2}{2}  \EB M(\x_t-\x^{\star})^{\alpha -1} \|\sH(\x_t, \xi_t) \|_\bp^4.
	\end{align*}

	\paragraph{For the first term}
	We first note that by a similar argument of $(a)$ in~\eqref{eq:term3-4}, we have
	\[
	|\langle \nabla M(\x_t-\x^{\star}),  \sH(\x_t, \xi_{t}) \rangle |
	\le (\bp-1) u_{\bp}^2 \lambda  \| \x_t-\x^{\star}\|  \cdot \| \sH(\x_t, \xi_{t}) \|.
	\]
	Second, we have
	\begin{align*}
		\EB [\| \sH(\x_t, \xi_{t})  \|^2 |\FM_{t-1} ]
		&= \PM\| \sH(\x_t, \xi_{t-1})  \|^2 \\
		&\le 2 \left[  \PM\| \sH(\x_t, \xi_{t-1})-\sH(\x^{\star}, \xi_{t-1} ) \|^2 + \PM \|\sH(\x^{\star}, \xi_{t-1})\|^2
		\right]\\
		&\overset{(a)}{\le} 2 L_H^2 \|\x_t -\x^{\star}\|^2 + 2 \PM \|\sH(\x^{\star}, \xi_{t-1})\|^2 \\
		&\overset{(b)}{\le} 2 L_H^2 \|\x_t -\x^{\star}\|^2 + 4M^2(\|\x^{\star}\|^2 + \PM g^2(\xi_{t-1}))
	\end{align*}
	where $(a)$ uses Assumption~\ref{asmp:H} and $(b)$ uses Assumption~\ref{asmp:growth}.
	As a result
	\begin{align*}
		\EB &M(\x_t-\x^{\star})^{\alpha -1}|\langle \nabla M(\x_t-\x^{\star}),  \sH(\x_t, \xi_t) \rangle |^2  \\
		&\precsim  \EB M(\x_t-\x^{\star})^{\alpha -1}  \left[\| \x_t-\x^{\star}\|^2  \cdot \| \sH(\x_t, \xi_{t}) \|^2\right] \\
		&=  \EB M(\x_t-\x^{\star})^{\alpha -1}\| \x_t-\x^{\star}\|^2  \cdot	\EB [\| \sH(\x_t, \xi_{t})  \|^2 |\FM_{t-1} ] \\
		&\precsim \EB M(\x_t-\x^{\star})^{\alpha -1}\| \x_t-\x^{\star}\|^2  \cdot	 \left[
		\|\x_t -\x^{\star}\|^2 +  \|\x^{\star}\|^2 +  \PM g^2(\xi_{t-1})
		\right] \\
		&\overset{(a)}{\precsim} \EB M(\x_t-\x^{\star})^{\alpha +1 }  + \EB M(\x_t-\x^{\star})^{\alpha}  + \EB M(\x_t-\x^{\star})^{\alpha } g^2(\xi_t) \\
		&\overset{(b)}{\le} \EB M(\x_t-\x^{\star})^{\alpha +1 }  + \EB M(\x_t-\x^{\star})^{\alpha}  +\left( \EB M(\x_t-\x^{\star})^{1+ \alpha} \right)^{\frac{\alpha}{\alpha+1}},
	\end{align*}
	where $(a)$ uses~\ref{asmp:appro-envelop} in Lemma~\ref{lem:envelop} and $(b)$ uses the following inequality (proved by Hölder's inequality) and $p=2(1+\alpha)$,
	\begin{align*}
		\EB M(\x_t-\x^{\star})^{\alpha } g^2(\xi_t)
		&\le  \left( \EB M(\x_t-\x^{\star})^{ \alpha \frac{p}{p-2}} \right)^{1-\frac{2}{p}}   (\EB |g(\xi_t)|^{p})^{\frac{2}{p}}
		\precsim \left( \EB M(\x_t-\x^{\star})^{1+ \alpha} \right)^{\frac{\alpha}{\alpha+1}} .
	\end{align*}
	Therefore,
	\begin{align*}
		\EB M(\x_t-\x^{\star})^{\alpha -1} & |\langle \nabla M(\x_t-\x^{\star}),  \sH(\x_t, \xi_t) \rangle |^2 \\
		&\precsim  \EB M(\x_t-\x^{\star})^{\alpha +1 }  + \EB M(\x_t-\x^{\star})^{\alpha}  +\left( \EB M(\x_t-\x^{\star})^{1+ \alpha} \right)^{\frac{\alpha}{\alpha+1}} \\
			&\le  \EB M(\x_t-\x^{\star})^{\alpha +1 } +\left( \EB M(\x_t-\x^{\star})^{1+ \alpha} \right)^{\frac{\alpha}{\alpha+1}} .
	\end{align*}

	\paragraph{For the second term}
	It follows from Hölder's inequality that
	\begin{align*}
		\EB M(\x_{t}-\x^{\star})^{\alpha-1}  \|\sH(\x_t, \xi_t) \|_\bp^4
		&\le (\EB M(\x_{t}-\x^{\star})^{1+\alpha})^\frac{\alpha-1}{1+\alpha}
		(\EB  \|\sH(\x_t, \xi_t) \|_\bp^{2(1+\alpha)})^\frac{2}{1+\alpha}\\
		&\precsim (\EB M(\x_{t}-\x^{\star})^{1+\alpha})^\frac{\alpha-1}{1+\alpha}
		(\EB  \|\sH(\x_t, \xi_t) \|^{2(1+\alpha)})^\frac{2}{1+\alpha}\\
		&
		\precsim (\EB M(\x_{t}-\x^{\star})^{1+\alpha})^\frac{\alpha-1}{1+\alpha}	(\EB \PM \|\sH(\x_t, \xi_{t-1}) \|^{\udp})^\frac{2}{1+\alpha}.
	\end{align*}
	By~\eqref{eq:help1}, we have $\EB \PM \|\sH(\x_t, \xi_{t-1}) \|^{\udp}  	\precsim \EB M(\x_{t}-\x^{\star})^{1+\alpha} + 1$.
	Using $(x+1)^{\frac{1}{1+\alpha}} \le x^{\frac{1}{1+\alpha}} +1$ for $x \ge0$, we again have
	\begin{equation}
		\tag{\ref{eq:p-cross-term3}}
		\EB M(\x_{t}-\x^{\star})^{\alpha}  \|\sH(\x_t, \xi_t) \|_\bp^2
		\precsim \EB M(\x_{t}-\x^{\star})^{1+\alpha}	+(\EB M(\x_{t}-\x^{\star})^{1+\alpha})^\frac{\alpha-1}{\alpha+1}.
	\end{equation}
	
	Combing these two parts, we complete the proof.
\end{proof}

\section{Proof for the semiparametric efficient lower bound}

\subsection{Proof of Theorem \ref{thm:lower}}

\begin{proof}[Proof of Theorem \ref{thm:lower}]
	In literature, the semiparametric efficiency for empirical estimators has been well understood when the interest of (unknown) parameter is in an expectation form, i.e., $\EB_{\xi \sim \pi} \ell(\xi)$ for a function $\ell$.
	However, our interest parameter is $\x^{\star}$, which is the root of the equation $\sg(\x) := \EB_{\xi \sim \pi }\sH(\x, \xi) = \0$.
	To make use of the existing result, we provide the following lemma to serve as a bridge.
	\begin{lem}\label{lem:zest_to_mest}
		For any RAL estimator $\sT_n$ for $\x^{\star}$ on $\pi$ with limit $\LL$, we have that $\g(\sT_n)$ is an RAL estimator for $-\EB_{\xi \sim \pi}\sH(\x^{\star},\xi)$ with limit $\sG\cdot\LL$.
	\end{lem}
	
	For any RAL estimator $\sT_n$ for $\x^{\star}$ on $\pi$ with limit $\LL$, Lemma~\ref{lem:zest_to_mest} shows the transformed estimator $\g(\sT_n)$ is an RAL estimator for $-\EB_{\xi \sim \pi}\sH(\x^{\star},\xi)$ with limit $\sG\cdot\LL$.
	Because $-\EB_{\xi \sim \pi}\sH(\x^{\star},\xi)$ is a parameter in the expectation form, the Markovian convolution theorem presented in \citet{greenwood1998maximum} shows that $\sG\cdot\LL$ can be represented as $\M+\N$, where $\M$ is independent of $\N$ and $\N$ is Gaussian distributed with zero mean and the covariance $\EB_{\xi \sim \pi}\left[(\IM - \gP)^{-1}\sH(\x^{\star},\xi)\right]\left[(\IM - \gP)^{-1}\sH(\x^{\star},\xi)\right]^\top$.
By Lemma~\ref{lem:poisson}, we know the matrix is exactly $\sS$.
Therefore, under $P$, $\Var(\N) \succeq \sS$ and thus
	\[
	\lim\limits_{n\to\infty}n\EB(\sT_n - \x^{\star})(\sT_n - \x^{\star})^\top  
	= \Var({\LL})
	=  \sG^{-1}\Var(\M+\N) \sG^{-\top}	\succeq  \sG^{-1} \Var(\N)\sG^{-\top}
	=  \sG^{-1} \sS \sG^{-\top}.
	\]
\end{proof}

\subsection{Proof of Theorem~\ref{thm:ral}}
\begin{proof}[Proof of Theorem~\ref{thm:ral}]
	In Section~\ref{sec:fclt}, we have analyzed $\ph_T$.
	We will make many results obtained therein.
	We decompose $\ph_T$ into several terms in~\eqref{eq:bpsi}
	\[
	\widetilde{\ph}_T(r)  - \frac{1}{\sqrt{T}} \sum_{j=0}^{\floor{Tr}} \sG^{-1}  \su_t = \Bpsi_0(r) + \Bpsi_1(r) + \Bpsi_2(r) +  \Bpsi_3(r).
	\]
	We also show that $\vertiii{\widetilde{\ph}_T-\ph_T} = o_{\PB}(1)$ and $\vertiii{\Bpsi_k} = o_{\PB}(1)$ for $0 \le k \le 3$.
	In the proof of Lemma~\ref{lem:error-analysis}, we also decompose $\su_t := \su_{t, 1} + \su_{t, 2}$ into two terms in~\eqref{eq:U-12} such that we have
	\[
	\vertiii{\frac{1}{\sqrt{T}}\sum_{t=1}^{\ceil{Tr}} \su_{t, 1}} = o_{\PB}(1) 
	\ \text{and} \ \su_{t, 2} =  \left[  \sU(\x^{\star}, \xi_t) - \PM \sU(\x^{\star}, \xi_{t-1}) \right] .
	\]
	Putting these results together and using Slutsky's theorem, we finish the proof.
\end{proof}

\subsection{Proof of Lemma \ref{lem:zest_to_mest}}
\begin{proof}[Proof of Lemma \ref{lem:zest_to_mest}]
	By the definition of RAL estimators, we need to check asymptotic linearity and regularity.
	We denote by $\PM$ and $\PM_{n\sh}$ forward operator of the transition kernels $P$ and $P_{n\sh}$ respectively.
	
	\paragraph{Asymptotic linearity}
	From the regularity of $\sT_n$, we have $\sqrt{n}(\sT_n -\x^{\star}) \overset{d}{\to} \LL$ under $P$.
	It implies that $\sT_n \overset{p}{\to} \x^{\star}$ and $\EB_{P^n}\|\sT_n - \x^{\star}\|^2 \precsim \frac{1}{n}$.
	By Assumption \ref{asmp:nonlinear}, it holds that
	\[
	\|\sqrt{n}\left(\g(\sT_n) - \g(\x^{\star})\right) - \sqrt{n}\sG(\sT_n - \x^{\star})\| \le L_G\sqrt{n}\|\sT_n - \x^{\star}\|^2 + o_{P^n}(1) = o_{P^n}(1).
	\]
	By the asymptotic linearity of $\sT_n$, we have $	\sqrt{n} (\sT_n - \x^{\star}) = \frac{1}{\sqrt{n}} \sum_{i=1}^n \vph(\xi_{i-1},\xi) + o_{P^n}(1)$ and thus
	\[
	\sqrt{n}(\g(\sT_n) - \g(\x^{\star}))= \sqrt{n}\g(\sT_n)= \frac{1}{\sqrt{n}}\ssum{i}{1}{n}\sG\vph(\xi_{i-1}, \xi_i) + o_{P^n}(1).
	\]
	\paragraph{Regularity}
	We first control the sum $\EB_{\xi \sim \pi}\sH(\x_{n\sh}^{\star},\xi) + \EB_{\xi \sim \pi_{n\sh}}\sH(\x^{\star},\xi)$. 
	By using the fact $\EB_{\sim \sim \pi}\sH(\x^{\star},\xi) = \EB_{\xi \sim \pi_{n\sh}}\sH(\x_{n\sh}^{\star},\xi) = \0$, we have
	\begin{align*}
		&\EB_{\xi \sim \pi}\sH(\x_{n\sh}^{\star},\xi) + \EB_{\pi_{n\sh}} \sH(\x^{\star}, \xi)  \\
		=& 
		\EB_{\xi \sim \pi}[\sH(\x_{n\sh}^{\star},\xi) - \sH(\x^{\star}, \xi)] - \EB_{\xi \sim \pi_{n\sh}}[\sH(\x_{n\sh}^{\star},\xi) - \sH(\x^{\star}, \xi)]\\
		\overset{(a)}{=}& \EB_{\xi \sim  \pi}\gP[\sH(\x_{n\sh}^{\star},\xi) - \sH(\x^{\star}, \xi)] -
		\EB_{\xi \sim \pi_{n\sh}}\gP_{n\sh}[\sH(\x_{n\sh}^{\star},\xi) - \sH(\x^{\star}, \xi)]\\
		\overset{(b)}{=}& \EB_{\xi \sim  \pi}\gP[\sH(\x_{n\sh}^{\star},\xi) - \sH(\x^{\star}, \xi)] -
		\EB_{\xi\sim\pi_{n\sh}} \gP [\sH(\x_{n\sh}^{\star},\xi) - \sH(\x^{\star}, \xi)] \\
		& \qquad + \frac{1}{\sqrt{n}} \EB_{\xi'\sim\pi_{n\sh}} \EB_{\xi \sim P(\xi, \cdot)} \sh(\xi, \xi') [\sH(\x_{n\sh}^{\star},\xi') - \sH(\x^{\star}, \xi')]\\
		=& \int_{\Xi} \gP[\sH(\x_{n\sh}^{\star},\xi) - \sH(\x^{\star}, \xi)](\pi(d\xi) - \pi_{n\sh}(d\xi)) \\
			& \qquad +\frac{1}{\sqrt{n}} \EB_{\xi'\sim\pi_{n\sh}} \EB_{\xi \sim P(\xi, \cdot)} \sh(\xi, \xi') [\sH(\x_{n\sh}^{\star},\xi') - \sH(\x^{\star}, \xi')]\\
		:=& \gZ_1 + \gZ_2.
	\end{align*}
	where $(a)$ uses the fact that $\pi$ and $\pi_{n\sh}$ are stationary distributions of $P$ and $P_{n\sh}$ and $(b)$ uses the choice $\gP_{n\sh}(\xi, d\xi') = \gP(\xi, d\xi')\left(1+ \frac{1}{\sqrt{n}}\sh(\xi,\xi')\right)$.
	
	We then bound the two term $\gZ_1$ and $\gZ_2$ respectively.
	By the boundedness of $\sh$ and Assumption \ref{asmp:H}, we have
	\[
	\|\gZ_2\| \precsim \frac{1}{\sqrt{n}}\EB_{\xi \sim \pi_{n\sh}}\gP\|\sH(\x_{n\sh}^{\star},\xi) - \sH(\x^{\star}, \xi)\| \precsim \frac{1}{\sqrt{n}}\|\x_{n\sh}^{\star} - \x^{\star}\|.
	\]
	On the other hand, from Assumption \ref{asmp:markov-noise}, both of the transition kernels $P$ and $P_{n\sh}$ are \emph{strongly stable} which is defined in \citet{kartashov1986inequalities}. By Theorem 3 in \citet{kartashov1986inequalities}, it follows that $\dTV(\pi, \pi_{n\sh})  \precsim \sup\limits_{\xi\in\Xi} \dTV(\PM(\xi, \cdot), \PM_{n\sh}(\xi, \cdot))$.
	Therefore,
	\begin{align*}
		\|\gZ_1\| &\le \int_{\Xi} \|\gP[\sH(\x_{n\sh}^{\star},\xi) - \sH(\x^{\star}, \xi)]\|\cdot |\pi(d\xi) - \pi_{n\sh}(d\xi)|\\
		&\le \sup\limits_{\xi\in\Xi}\gP\|\sH(\x_{n\sh}^{\star},\xi) - \sH(\x^{\star}, \xi)\|\cdot\dTV(\pi, \pi_{n\sh}) \\
		&\overset{(a)}{\precsim} \|\x_{n\sh}^{\star} - \x^{\star}\|\cdot  \sup\limits_{\xi\in\Xi} \dTV(\PM(\xi, \cdot), \PM_{n\sh}(\xi, \cdot))\\
		&\overset{(b)}{\le} \|\x^{\star}_{n\sh} - x^{\star}\|\ \cdot \frac{1}{\sqrt{n}}\sup\limits_{\xi,\xi' \in \Xi}\|\sh(\xi,\xi')\| 
		\precsim \frac{1}{\sqrt{n}}\|\x^{\star}_{n\sh} - x^{\star}\|
	\end{align*}
	where $(a)$ follows from Assumption \ref{asmp:H} and $(b)$ follows from the definition of $\gP_{n\sh}(\xi, d\xi')$. 
	Combining these two bounds, we get that 
	\[
\g(\x^{\star}_{n\sh}) + \EB_{\xi \sim \pi_{n\sh}}\sH(\x^{\star},\xi)=	\EB_{\xi \sim \pi}\sH(\x_{n\sh}^{\star},\xi) + \EB_{\xi \sim \pi_{n\sh}}\sH(\x^{\star}, \xi) \precsim \frac{\|\x^{\star}_{n\sh} - \x^{\star}\|}{\sqrt{n}}.
	\]
	Noting that $\EB_{\xi \sim \pi_{n\sh}}\sH(\x^{\star},\xi)  = \EB_{\xi \sim \pi_{n\sh}}\sH(\x^{\star},\xi) - \EB_{\xi \sim \pi}\sH(\x^{\star},\xi) $, we can show $\EB_{\xi \sim \pi_{n\sh}}\sH(\x^{\star},\xi) = \gO(1/\sqrt{n})$ by using the same technique in bounding $\|\gZ_1\|$.
Using the last inequality, we have
	\begin{align*}
		\sg(\x^{\star}) - \sg(\x^{\star}_{n\sh}) &= - \EB_{\xi \sim \pi}\sH(\x^{\star}_{n\sh},\xi) - \EB_{\xi \sim \pi_{n\sh}}\sH(\x^{\star},\xi) + \EB_{\xi \sim \pi_{n\sh}}\sH(\x^{\star},\xi) \\
		&= \EB_{\xi \sim \pi_{n\sh}}\sH(\x^{\star},\xi) + \gO\left(\frac{1}{\sqrt{n}}\|\x^{\star}_{n\sh} - \x^{\star}\|\right).
	\end{align*}
	By Assumption \ref{asmp:lya}, it is easy to show that $(1-\gamma)c\|\x^{\star}_{n\sh} - \x^{\star}\| \le \|\g(\x^{\star}_{n\sh}) - \g(\x^{\star})\|$.
	Hence,
	\[
	\|\x^{\star}_{n\sh} - \x^{\star}\| \le \|\EB_{\pi_{n\sh}}\sH(\x^{\star},\xi)\| + \gO\left(\frac{1}{\sqrt{n}}\|\x^{\star}_{n\sh} - \x^{\star}\|\right) = \gO\left(\frac{1}{\sqrt{n}}\right) + \gO\left(\frac{1}{\sqrt{n}}\|\x^{\star}_{n\sh} - \x^{\star}\|\right)
	\]
	Rearranging the last inequality yields $\|\x^{\star}_{n\sh} - \x^{\star}\| \precsim \frac{1}{\sqrt{n}}$. 
	
	Finally, by the regularity of $\sT_n$, we have $\sqrt{n}(\sT_n -\x_{n\sh}^{\star}) \overset{d}{\to} \LL$ under the perturbed distribution $P_{n\sh}$ and thus $\sT_n \overset{p}{\to} \x^{\star}$.
	Therefore,
	\begin{align*}
		&\sqrt{n}(\sg(\sT_n) + \EB_{\xi \sim \pi_{n\sh}}\sH(\x^{\star},\xi))  \\
		=& \sqrt{n}(\sg(\sT_n) - \sg(\x^{\star}_{n\sh})) + \sqrt{n}\left(\g(\x^{\star}_{n\sh}) + \EB_{\xi \sim \pi_{n\sh}}\sH(\x^{\star},\xi)\right) \\
		=& \sqrt{n}[(\sg(\sT_n) - \sg(\x^{\star})) - (\sg(\x^{\star}_{n\sh}) - \sg(\x^{\star}))] + \gO(\|\x^{\star}_{n\sh} - \x^{\star}\|)\\
		=& \sqrt{n}[\sG(\sT_n - \x^{\star}) - \sG(\x^{\star}_{n\sh} - \x^{\star})] + \gO\left(\sqrt{n}\|\sT_n - \x^{\star}_{n\sh}\|^2 + \sqrt{n}\|\x^{\star}_{n\sh} - \x^{\star}\|^2\right) + \gO(1/\sqrt{n})\\
		=& \sG\sqrt{n}(\sT_n- \x^{\star}_{n\sh}) + \gO_{P^n}(1/\sqrt{n}) = 
		\sG\sqrt{n}(\sT_n - \x^{\star}_{n\sh}) + o_{P^n}(1)\\
		\overset{d}{\to}& \sG\cdot\LL.
	\end{align*}
The last equation means  $\sg(\sT_n)$ is a regular estimator for $ \EB_{\xi \sim \pi}\sH(\x^{\star},\xi) $ with limit $\sG \LL$.
\end{proof}

\section{Convergence rate of functional central limit theorem}
\label{appen:rate}
\subsection{A Ky-Fan-metric-type functional}
Before presenting the proof, we introduce additional preliminaries and notation. 
%We denote $(\sC_{[0,1]}, \vertiii{\cdot})$ as the metric space consisting of all $d$-dimensional continuous functions on $[0, 1]$ (i.e., $\vx:[0,1]\to \RB^d$) with the uniform norm $\vertiii{\vx} = \sup\limits_{t\in[0,1]}\|\vx_t\|$. 
%As shown by~\citet{skorokhod1956limit}, $(\C_{[0,1]}, \|\cdot\|_\infty)$ is a Polish space that is separable, completely, and metrizable.
%Let $\gC_{[0,1]}$ be the Borel algebra in $(\C_{[0,1]}, \|\cdot\|_\infty)$ that is formed from open sets through the operations of countable union, countable intersection, and relative complement.
%Therefore, $(\C_{[0,1]}, \gC_{[0,1]}, \PB)$ becomes a probability space.
%
%For two probability measures $Q_1$ and $Q_2$ on $(\C_{[0,1]},\gC_{[0,1]})$, we denote by $d_P$ the L\'evy-Prokhorov metric~\citep{prokhorov1956convergence,gibbs2002choosing}, i.e.,
%\begin{equation}
%	\label{eq:dp}
%	d_P(Q_1,Q_2) := \inf\{\eps:Q_1(B)\le Q_2(B^\eps) + \eps; ~\forall B\in \gC_{[0,1]}\}.
%\end{equation}
%where we use $B^\eps := \{\vx: \inf\limits_{\vy\in B}\|\vx-\vy\|_\infty \le \eps\}$. 
%Since $(\C_{[0,1]}, \|\cdot\|_\infty)$ is separable, convergence of measures in the Lévy–Prokhorov metric is equivalent to weak convergence of measures.
We relate the L\'evy-Prokhorov metric  $\dS(\cdot)$ in~\eqref{eq:dp} with a Ky-Fan-metric-type functional $\widetilde{d}(\cdot)$ that would be frequently used latter on.
For any continuous stochastic process $\ph \in \BDD$, we denote 
\begin{equation}
	\label{eq:kfm}
	\widetilde{d}(\ph) := \inf\limits_{\eps \ge 0} \eps\vee \PB( \vertiii{\ph} > \eps).
\end{equation}

\begin{prop}\label{prop:dstb_on_pkhv}
	\label{prop:diff}
	For any $\ph_1,\ph_2 \in \BDD$, it then follows that
	\[
	\dP(\ph_1+\ph_2, \ph_1)  \le \widetilde{d}(\ph_2).
	\]
\end{prop}

\begin{proof}[Proof of Proposition~\ref{prop:dstb_on_pkhv}]
	For each $\ph_2$, we assume the maximum in $\widetilde{d}(\ph_2)$ is achieved by $\eps_2$ such that $\widetilde{d}(\ph_2) = \eps_2 \vee \PB( \vertiii{\ph_2} > \eps_2)$. 
	It is obvious that $\eps_2 \le \widetilde{d}(\ph_2)$. 
	Recall that $B^\eps := \{\ph_1: \inf\limits_{\ph_2\in B} \dS(\ph_1, \ph_2) \le \eps\}$. 
	Then, for any $B\in \BDM$, once $\ph_1 + \ph_2 \in B$ and $\vertiii{\ph_2} \le \eps$, we have $\ph_1 \in B^{\eps}$. 
	Therefore,
	\begin{align*}
		\PB(\ph_1+ \ph_2 \in B)&= \PB(\ph_1 + \ph_2 \in B, \vertiii{\ph_2} \le \eps_2) + \PB(\ph_1 + \ph_2 \in B, \vertiii{\ph_2} > \eps_2)\\
		&\le \PB(\ph_1\in B^{\eps_2}) + \PB(\vertiii{\ph_2} > \eps_2)\\
		&\le \PB(\ph_1 \in B^{\widetilde{d}(\ph_2)}) + \widetilde{d}(\ph_2).
	\end{align*}
	By taking $B$ as all measurable set in $\BDM$, we conclude that $\dP( \ph_1+\ph_2, \ph_1 ) \le \widetilde{d}(\ph_2)$ by the definition of $\dP$ in~\eqref{eq:dp}.
\end{proof}

\begin{prop}\label{prop:one_on_pkhv}
	\label{prop:one}
	Let $g: \BDD \to {\mathsf{D}_{[0, 1],\RB^k}} (k \ge 1)$ be $L$-Lipschitz continuous in $\vertiii{\cdot}$ in the sense that $\vertiii{f(\ph_1)-f(\ph_2)} \le L \cdot \vertiii{\ph_1-\ph_2}$ for any $\ph_1, \ph_2 \in \BDD$.
	For any $\ph_1, \ph_2 \in \BDD$, it follows that
	\[
	\dP(g(\ph_1),g(\ph_2)) \le (L \vee 1)  \cdot   \dP(\ph_1,\ph_2)  .
	\]
\end{prop}

\begin{proof}[Proof of Proposition~\ref{prop:one_on_pkhv}]
	Let $\widetilde{B}$ be any measurable Borel set in $\RB^k$ and we define $B = \{ \ph \in \BDO:   g(\ph) \in \widetilde{B}  \}$.
	Let $\eps =  \dP(\ph_1,\ph_2)$. 
	By definition, we have $\PB(\ph_1 \in B) \le \PB(\ph_2 \in B^\eps) + \eps$.
	Notice that $\PB(\ph_1 \in B) = \PB( g(\ph_1) \in \widetilde{B})$ and $\PB(\ph_2 \in B^\eps) \le \PB( g(\ph_2) \in \widetilde{B}^{L\eps})$.
	
	The second inequality uses the result that if $\ph_2 \in B^\eps$, then there exists $\ph_3 \in B$ such that $g(\ph_3) \in B$ and $\vertiii{\ph_2-\ph_3}\le \eps$.
	Therefore, $\vertiii{g(\ph_2)-g(\ph_3)}  \le L \cdot \vertiii{\ph_2-\ph_3} \le L\cdot\eps$ and thus $g(\ph_2) \in \widetilde{B}^{L\eps}$.
	Hence, by arbitrariness of $\widetilde{B}$, $\dP(g(\ph_1), g(\ph_2)) \le   (L \vee 1)  \cdot \dP(\ph_1,\ph_2)$.
\end{proof}

As a direct corollary of Proposition~\ref{prop:one}, we have
\begin{cor}
	\label{cor:linear}
	For any vector $\ThetaSym \in \RB^d$ satisfying $\|\ThetaSym\|_* = 1$,
	\[
	\dP(\ThetaSym^\top\ph_1, \ThetaSym^\top\ph_2) \le   \dP(\ph_1,\ph_2)  .
	\]
\end{cor}

\begin{prop}\label{prop:pkhv_to_mmt}
	If $\ph  \in \BDD$ satisfies $\EB\vertiii{\ph}^p < \infty$ with $p>0$, then
	\[
	\widetilde{d}(\ph) \le \left(\EB\vertiii{\ph}^p\right)^{\frac{1}{p+1}}.
	\]
\end{prop}
\begin{proof}[Proof of Proposition~\ref{prop:pkhv_to_mmt}]
	With $\eps = \left(\EB\vertiii{\ph}^p\right)^{\frac{1}{p+1}}$, Markov's inequality yields that $\PB(\vertiii{\ph} > \eps) \le \frac{\EB\vertiii{\ph}^p}{\eps^p} = \eps$.
	Hence, $\widetilde{d}(\ph) \le \eps\vee \PB(\vertiii{\ph}> \eps) = \eps = \left(\EB\vertiii{\ph}^p\right)^{\frac{1}{p+1}}$.
	% . Then, we can get $\eps = \frac{\EB\|\vy\|_\infty^p}{\eps^p}$. Then by the Markov's inequality, $\PB(\|\vy\|_\infty > \eps) \le \frac{\EB\|\vy\|_\infty^p}{\eps^p} = \eps$. So 
\end{proof}

% The above two propositions play key roles in our subsequent derivations. They help us to divide a complicated problem into several simpler tasks and connect them with the results that we are more familiar with.

Proposition~\ref{prop:diff} shows that the L\'evy-Prokhorov metric between $\ph_1+\ph_2$ and $\ph_1$ is exactly bounded by $\widetilde{d}(\ph_2)$.
Proposition~\ref{prop:pkhv_to_mmt} then implies $\widetilde{d}(\ph_2)$ is further bounded by  $\left(\EB\vertiii{\ph_2}^p\right)^{\frac{1}{p+1}}$ if the $p$-th order moment exists.
In this way, we reduce the L\'evy-Prokhorov metric between two given random processes to the high-order moments of their difference.
The latter is more tractable and thus easier to analyze.

\begin{thm}[Corollary 1 in \citet{kubilius1985rate})]
	\label{thm:rate_fclt_mkv}
	Let $(X^n,F^n)$ be a sequence of locally square integrable martingales in $\RB$, and $(X,F)$ be a continuous Gaussian martingale. Then for any $T>0$, and $0<\delta < 3/2$,
	\begin{equation}
		\begin{gathered}
			\dP\left(X^n,  X\right)=\gO\left(\left\{\left(\EB \sup _{t \leqslant T}\left|\left\langle X^n\right\rangle_t-\langle X\rangle_t\right|\right)^{\frac{1}{3}}+\left(\EB \int_0^T \int_\RB|x|^{2+2\delta} \Pi^n(d s, d x)\right)^{\frac{1}{3+2 \delta}}\right\}\right. \\
			\left.\quad \times\left|\ln \left(\EB \sup _{t \leqslant T}\left|\left\langle X^n\right\rangle_t-\langle X\rangle_t\right|+\EB \int_0^T \int_{\RB}|x|^{2+2 \delta} \Pi^n(d s, d x)\right)\right|^{1 / 2}\right) .
		\end{gathered}
	\end{equation}
	where $\langle X\rangle$ is the quadratic characteristic of $X$ and $\Pi^n$ is the dual predictable projection of the process $X^n$.
\end{thm}

\subsection{Proof of Theorem~\ref{thm:rate}}
\label{proof:error-decom2}
\begin{proof}[Proof of Theorem~\ref{thm:rate}]
	
We rewrite $p=2(1+\delta)$ for simplicity. 
Then $p>2$ is equivalent to $\delta > 0$.
\paragraph{Step one: Finer partial-sum process decomposition}
We have analyzed the partial-sum decomposition in Section~\ref{proof:recursion}.
We will further decompose two terms to proceed proof.
Recall that $\widetilde{\ph}_T(r) = \frac{1}{\sqrt{T}}\sum_{t=0}^{\floor{Tr}} (\tx_t -\x^{\star})$ and $\tx_t = \x_t -\eta_t\PM \sU(\x_{t}, \xi_{t-1})$.
We directly quote the result~\eqref{eq:bpsi} here
\begin{align}
	\widetilde{\ph}_T(r)  - \frac{1}{\sqrt{T}} \sum_{t=0}^{\floor{Tr}} \sG^{-1}  \su_t
	&= \frac{1}{\sqrt{T}\eta_0} \sA_0^{\floor{Tr}} \sB_0\De_0  
	+ \frac{1}{\sqrt{T}} \sum_{t=0}^{\floor{Tr}} \sA_t^{\floor{Tr}}(\sr_t + \snu_t)
	\nonumber	\\
	&\qquad + \frac{1}{\sqrt{T}} \sum_{t=0}^{\floor{Tr}} \left(\sA_t^T -\sG^{-1}\right)\su_t
	+ \frac{1}{\sqrt{T}} \sum_{t=0}^{\floor{Tr}} \left(\sA_t^{\floor{Tr}} -\sA_t^T\right)\su_t\nonumber \\
	&:= \Bpsi_0(r) + \Bpsi_1(r) + \Bpsi_2(r) +  \Bpsi_3(r). \tag{\ref{eq:bpsi}}
\end{align}
First,  we further decompose $\Bpsi_1(r) := \Bpsi_{1,1}(r) +  \Bpsi_{1,2}(r)$ into two terms and arrive at
\[
\Bpsi_1(r) =\frac{1}{\sqrt{T}} \sum_{t=0}^{\floor{Tr}} \sA_t^{\floor{Tr}}(\sr_t + \snu_t) := \frac{1}{\sqrt{T}} \sum_{t=0}^{\floor{Tr}} \sA_t^{\floor{Tr}}\sr_t 
+ \frac{1}{\sqrt{T}} \sum_{t=0}^{\floor{Tr}} \sA_t^{\floor{Tr}}\snu_t
=: \Bpsi_{1,1}(r) +  \Bpsi_{1,2}(r).
\]
Second, we decompose the noise $\vu_t = \vu_{t,1}  + \vu_{t,2}$ where
\begin{align}
	\tag{\ref{eq:U-12}}
	\begin{split}
		\su_{t, 1} &=  \left[  \sU(\x_t, \xi_t) - \PM \sU(\x_t, \xi_{t-1}) \right] - \left[  \sU(\x^{\star}, \xi_t) - \PM \sU(\x^{\star}, \xi_{t-1}) \right],\\
		\su_{t, 2}&=  \left[  \sU(\x^{\star}, \xi_t) - \PM \sU(\x^{\star}, \xi_{t-1}) \right].
	\end{split}
\end{align}
This decomposition has been used to analyze the asymptotic behavior of $\frac{1}{\sqrt{T}}\ssum{t}{0}{T}\sG^{-1}\vu_t$ in Lemma~\ref{lem:error-analysis}.
From the proof of~\ref{lem:error-u} in Lemma~\ref{lem:error-analysis}, we know that both $\{ \su_{t,1} \}_{t \ge 0}$ and $\{ \su_{t,2} \}_{t \ge 0}$ are martingale difference sequences with bounded $(2+2\delta)$-th order moment.
For simplicity, we denote 
\[
\Bpsi_{4,1}(r) = \frac{1}{\sqrt{T}}\ssum{t}{0}{\floor{Tr}}\sG^{-1}\vu_{t,1}, \quad
\Bpsi_{4,2}(r) = \frac{1}{\sqrt{T}}\ssum{t}{0}{\floor{Tr}}\sG^{-1}\vu_{t,2}, \quad \text{and} \quad
\Bpsi(r) = \sG^{-1} \sS^{1/2} \sW(r).
\]
Therefore, it follows that
\[
\ph_T =  (\ph_T- \widetilde{\ph}_T) +  \Bpsi_0 + \Bpsi_{1,1} +  \Bpsi_{1,2}  + \Bpsi_{2} + \Bpsi_{3} + \Bpsi_{4,1} + \Bpsi_{4,2}.
\]
By repeatedly using Proposition~\ref{prop:dstb_on_pkhv} and Corollary~\ref{cor:linear}, it follows that for any $\ThetaSym \in \RB^d$ satisfying $\|\ThetaSym\|_*=1$,
\begin{align}
	\label{eq:finer-decomposition}
	\begin{split}
	\dP(\ThetaSym^\top\ph_T, \ThetaSym^\top\Bpsi)
	& \le \dP\left( \ThetaSym^\top{\ph}_T, \ThetaSym^\top\widetilde{\ph}_T\right)   + \widetilde{d}(\Bpsi_0) + \widetilde{d}(\Bpsi_{1,1})  + \widetilde{d}(\Bpsi_{1,2}) \\
	& \quad+ \widetilde{d}(\Bpsi_{2}) + \widetilde{d}(\Bpsi_{3}) +  \widetilde{d}(\Bpsi_{4,1})  + 	\dP(\ThetaSym^\top \Bpsi_{4,2}, \ThetaSym^\top\Bpsi).
	\end{split}
\end{align}

\paragraph{Step two: Moment analysis}
By Proposition~\ref{prop:pkhv_to_mmt}, each $\widetilde{d}(\Bpsi)$ is bounded by the moment $\left(\EB\vertiii{\Bpsi}^v\right)^{\frac{1}{v+1}}$ for any $1 \le v \le p$.
Therefore, analyzing most of the terms in the right-hand side of~\eqref{eq:finer-decomposition} is reduced to analyze their higher-order moment with the moment order $v$ unspecified as a variable.
Lemma~\ref{lem:moment} provides these higher order moment bounds with $\lambda, m, l, k$ the corresponding variables.
Given the interested parameters include only $\tmix$ and $T$, we will hide other parameter dependence in $\precsim, \OM$ and $\TOM$.
%From Lemma~\ref{lem:poisson}, we know that $C_U = \OM(\tmix)$ and $L_U = \OM(1+\tmix)$ depends on $\tmix$ implicitly, which is the reason why they appear in the following lemma.
The proof of Lemma~\ref{lem:moment} is collected in Section~\ref{proof:moment}.

\begin{lem}
	\label{lem:moment}
	Rewrite $p=2(1+\delta)$.
Under the assumptions of Theorem~\ref{thm:rate}, it follows that
\begin{align}
	\dP\left( \ThetaSym^\top{\ph}_T, \ThetaSym^\top\widetilde{\ph}_T\right)  &= 
	{\gO}\left(
\tmix^{\frac{1+m}{2+m}}\cdot T^{\frac{1+m}{2(2+m)}} \cdot \left( \frac{1}{T}\ssum{t}{0}{T}\eta_t^{1+m}\right)^{\frac{1}{2+m}}
	\right) \quad \forall m \in [0, 2\delta+1],\label{eq:d_p_1-1}\\
\widetilde{d}(\Bpsi_{0} ) &=\OM  \left( T^{-\frac{1}{2}} \right)	,	\label{eq:bpsi0} \\
	\widetilde{d}(\Bpsi_{1,1})&= \TOM \left(
		\left(c_r + \tmix\right)^{\frac{1+\lambda}{2+\lambda}}  \cdot 	T^{\frac{1+\lambda}{2(2+\lambda)}} \cdot \left(\frac{1}{T}\ssum{t}{0}{T}  \eta_t^{1+\lambda}\right)^{\frac{1}{2+\lambda}}
		\right) \quad \forall \lambda \in [0, \delta],  	\label{eq:bpsi11}\\
	\widetilde{d}(\Bpsi_{1,2})&=\widetilde{\gO}\left(
	\left(1+\tmix\right)^{\frac{1+m}{2+m}}\cdot T^{\frac{1+m}{2(2+m)}} \cdot \left( \frac{1}{T}\ssum{t}{0}{T}\eta_t^{1+m}\right)^{\frac{1}{2+m}}
	\right) \quad \forall m \in [0, 2\delta+1],	\label{eq:bpsi12} \\
		\widetilde{d}(\Bpsi_2) &= \gO\left(T^{-\frac{1-\alpha}{3}}\right)  ,	\label{eq:bpsi2} \\
		 \widetilde{d}(\Bpsi_3)&= \gO\left( (1+l) \cdot T^{-\frac{l(1-\alpha)}{3+2l}}\right) \quad \forall l \in [0, \delta],	\label{eq:bpsi3}\\
		 \widetilde{d}(\Bpsi_{4,1})&=	 \TOM\left( \sqrt{k} C_k  \cdot  \left( \frac{1}{T} \sum_{t=0}^T \eta_t^{k/2} \right)^{\frac{1}{1+k}}   \right)  \quad \forall k \in [1, 2(1+ \delta)],	\label{eq:bpsi41}\\
		\dP(\ThetaSym^\top \Bpsi_{4,2}, \ThetaSym^\top\Bpsi)&= \OM\left( T^{-\frac{\delta}{3+2\delta} }+ T^{- (\frac{1}{4}-o(1)) }  +T^{-\frac{1}{3}} + \tmix^{\frac{1}{6}} T^{-\frac{1}{6}} \right) \ \text{for an infinitesimal} \  o(1),\label{eq:bpsi42}
\end{align}
where $c_r :=\max\left\{L_G, \frac{L_H +\|\sG\|}{\delta_G}\right\}$ and $C_k$ is the constant in the $(L^p, (1+ \log t) \sqrt{\eta_t})$ consistency.
Here, $\TOM(\cdot)$ hides uninterested parameters and the log factor $\log T$.
\end{lem}

\paragraph{Step three: Variable selection}
Notice that for any $\beta \ge 0$, we have
\begin{equation}
	\label{eq:help-sum}
	\frac{1}{T} \sum_{t=0}^T \eta_t^\beta = 
	\frac{1}{T}\sum_{t=0}^T t^{-\alpha\beta} =
	\left\{ 
	\begin{array}{cc}
		\OM\left(\frac{1}{1-\alpha\beta} T^{-\alpha\beta} \right) & \text{if} \ \alpha \beta < 1 \\
		\OM \left( \frac{\log T}{T}  \right) & \text{if} \ \alpha\beta = 1\\
		\OM(\frac{1}{T} ) & \text{if} \  \alpha\beta > 1
	\end{array}
	\right.
	= \widetilde{\OM} \left( T^{- (\alpha \beta ) \wedge 1 } \right)
\end{equation}
where $\TOM(\cdot)$ hides the log factor $\log T$ and constant dependence on $\alpha, \beta$ and $a \wedge b = \min \{a, b\}$.

With the help of~\eqref{eq:help-sum}, we simplify the bounds in Lemma~\ref{lem:moment} by choosing (nearly) optimal variables $\lambda, m, l$ and $k$.
Recall that we rewrite $p=2(1+\delta)$ for simplicity.

\begin{itemize}
	\item It is easy to verify that
	\begin{equation}
			\label{eq:J1}
		J_1(\alpha) :=	\max_{k \in [1, 2(1+\delta)]}   \frac{\alpha k \wedge 2}{2(k+1)}  =  \left\{  
		\begin{array}{cc}
			\frac{\alpha(1+\delta)}{3+2\delta} & \text{if} \   \alpha \in \left(0, \frac{1}{1+\delta}\right] \ \text{achieved by} \  k=2(1+\delta), \\
			\frac{\alpha}{2+\alpha} & \text{if} \   \alpha \in \left[ \frac{1}{1+\delta}, 1\right) \ \text{achieved by} \ k = \frac{2}{\alpha} .
		\end{array}
		\right.
	\end{equation}
By setting $k = \min \left\{ 2(1+\delta), \frac{2}{\alpha} \right\}$, we get that
\[
\widetilde{d}\left( \Bpsi_{4,1} \right)  
=  \TOM\left(  \frac{C_{\frac{2}{\alpha} \wedge p } }{\sqrt{\alpha}} \cdot T^{-J_1(\alpha)}  \right) 
=   \TOM\left( T^{-J_1(\alpha)}  \right)
\]
where the last equality uses $\alpha \in (0.5, 1)$ and $C_k$ is increasing in $k$.
\item Note that
\[
T^{\frac{1+\lambda}{2(2+\lambda)}} \cdot \left( \frac{1}{T}\ssum{t}{0}{T}\eta_t^{1+\lambda}\right)^{\frac{1}{2+\lambda}} = \widetilde{\gO}\left(
T^{-   \frac{1+\lambda}{2+\lambda}\left[ 
	(\alpha-0.5) \wedge \frac{1-\lambda}{2(1+\lambda)}\right] }\right)
= \widetilde{\gO} \left( T^{-h_0(\lambda)} \right)
\]
where we denote
\begin{equation*}
	\label{eq:h0}
	h_0(\lambda) =  \frac{1+\lambda}{2+\lambda}\left[  (\alpha-0.5) \wedge \frac{1-\lambda}{2(1+\lambda)}\right].
\end{equation*}
One can show that
\begin{equation}
	\label{eq:J2}
	J_2(\alpha) :=	\max_{\lambda \in [0, \delta]} h_0(\lambda)
	= \left\{  
	\begin{array}{cc}
		(\alpha -0.5)\frac{1+\delta}{2+\delta}& \text{if} \   \alpha \in \left(0.5, \frac{1}{1+\delta}\right]  \ \text{achieved by} \  \lambda=\delta, \\
		\frac{\alpha-0.5}{\alpha+1} & \text{if} \   \alpha \in \left[ \frac{1}{1+\delta}, 1\right)   \ \text{achieved by} \  \lambda =  \frac{1}{\alpha}-1. \\
	\end{array}
	\right.
\end{equation}
By setting $\lambda = \min \left\{ \delta, \frac{1}{\alpha} -1 \right\}$, we get that
\[
\max \left\{	\widetilde{d}\left( \Bpsi_{1,1} \right), 	\widetilde{d}\left( \Bpsi_{1,2} \right)\right\}  
=\TOM\left(  (1 + \tmix)^{\frac{1+\delta}{2+\delta} }  \cdot T^{-J_2(\alpha)}  \right).
\]
\item Note that
\[
\max_{l \in [0, \delta]} \left[ \frac{1}{3} \wedge \frac{l}{3+2l} \right] 
	= \left\{  
\begin{array}{cc}
 \frac{\delta}{3+2\delta} & \text{if} \  \delta \in [0, 3] \ \text{achieved by} \  l = \delta, \\
	\frac{1}{3} & \text{if} \  \delta \in [3, \infty) \ \text{achieved by} \  l = 3. \\
\end{array}
\right.
\]
By setting $l = \min\{\delta, 3 \}$, we have that
\[
\max \left\{	\widetilde{d}\left( \Bpsi_{2} \right), 	\widetilde{d}\left( \Bpsi_{3} \right)\right\}  =  \TOM\left(  T^{ -(1-\alpha)  \left[\frac{\delta}{3+2\delta}  \wedge \frac{1}{3}\right] } \right).
\]
\item 
Finally, we note that $T^{ -(1-\alpha)  \left[\frac{\delta}{3+2\delta}  \wedge \frac{1}{3}\right] } \ge  \max \left\{
T^{-\frac{\delta}{3+2\delta} }, T^{- (\frac{1}{4}-o(1)) }, T^{-\frac{1}{3}}
\right\}$ due to $\alpha \in (0, 1)$.
\end{itemize}
Combining these bounds and using $p=2(1+\delta)$, we arrive at
\begin{align}
	\label{eq:rate-most}
	\dP(\ThetaSym^\top \ph_T, \ThetaSym^\top \Bpsi )
	= \TOM \left(T^{-J_1(\alpha)} +
	(1+\tmix)^{\frac{p}{2+p} }  \cdot T^{-J_2(\alpha)}  
	+ T^{ -(1-\alpha)  \left[\frac{\delta}{3+2\delta}  \wedge \frac{1}{3}\right] } +\tmix^{\frac{1}{6}} T^{-\frac{1}{6}} \right).
\end{align}

\paragraph{A special case: I.i.d. data}
From the above analysis, one can find that $\Bpsi_{1,2}$ contributes a lot to the bound~\eqref{eq:rate-most}.
When it comes to the i.i.d. case, $\sU(\x, \xi) = \sH(\x, \xi)$ and $\sg(\x) = \PM \sH(\x, \xi)$ for all $\x \in \RB^d$ and $\xi \in \Xi$.
In this case, there is a refined decomposition where $\Bpsi_{1,2}$ doesn't show up.
In contrast, $\Bpsi_{1,2}$ always appears in~\eqref{eq:finer-decomposition} no matter what the case is.

The key idea in the refined decomposition is to use $\ph_T$ rather than $\widetilde{\ph}_T$.
With a slight of notation abuse, we redefine $\De_t = \x_t -\x^{\star}$, then similar to~\eqref{eq:help0}, we have $\De_{t+1} = (\sI -\eta_t \sG) \De_t + \eta_t [\sr_t + \su_t]$ where $\sr_t =\sg(\x_t) - \sG( \x_t -\x^{\star})$.
The key observation is that once iterating $\ph_T$ rather than $\widetilde{\ph}_T$, the sum of the residual term and coboudary term in~\eqref{eq:decompose0} equals to zero because $\PM\sU(\x_t, \xi) = \sg(\x_t)$ for all $\xi \in \Xi$.
Hence, by a similar recursion analysis in Section~\ref{proof:recursion}, we have
\[
\ph_T = \Bpsi_0 + \Bpsi_{1,1} + \Bpsi_2 +  \Bpsi_3 + \Bpsi_{4,1} + \Bpsi_{4,2}.
\]
By repeatedly using Proposition~\ref{prop:dstb_on_pkhv} and Corollary~\ref{cor:linear}, it follows that for any $\ThetaSym \in \RB^d$ satisfying $\|\ThetaSym\|_*=1$,
\begin{align*}
		\dP(\ThetaSym^\top\ph_T, \ThetaSym^\top\Bpsi)
		& \le \widetilde{d}(\Bpsi_0) + \widetilde{d}(\Bpsi_{1,1}) + \widetilde{d}(\Bpsi_{2}) + \widetilde{d}(\Bpsi_{3}) +  \widetilde{d}(\Bpsi_{4,1})  + 	\dP(\ThetaSym^\top \Bpsi_{4,2}, \ThetaSym^\top\Bpsi).
\end{align*}
It turns out that $\dP(\ThetaSym^\top\ph_T, \ThetaSym^\top\Bpsi)$ doesn't depend on $\widetilde{d}(\Bpsi_{2})$ any more.
We comment that~\eqref{eq:bpsi11} is still a valid upper bound for $\widetilde{d}(\Bpsi_{1,1})$ even we change the definition of $\De_t$ from $\widetilde{\x}_t-\x^{\star}$ to $\x_t -\x^{\star}$.

Taking this special case into consideration, we have
\begin{align*}
	\max \left\{	\widetilde{d}\left( \Bpsi_{1,1} \right), 	\widetilde{d}\left( \Bpsi_{1,2} \right)\right\}  
	&=  \TOM\left(  (c_r + \tmix + (1+\tmix) \mathds{1}_{\tmix } )^{\frac{1+\delta}{2+\delta} }  \cdot T^{-J_2(\alpha)}  \right)\\
	&=\TOM\left(  (c_r + \tmix)^{\frac{1+\delta}{2+\delta} }  \cdot T^{-J_2(\alpha)}  \right).
\end{align*}
where $\mathds{1}_{\tmix}$ is an indicator function for the event $\{ \tmix > 0 \}$ satisfying $\mathds{1}_{\tmix} \le \tmix$.
As a result, a finer bound is 
\begin{equation}
\tag{\ref{eq:rate-bound}}
	\dP(\ThetaSym^\top \ph_T, \ThetaSym^\top \Bpsi )
= \TOM \left(T^{-J_1(\alpha)} +
(c_r+\tmix)^{\frac{p}{2+p} }  \cdot T^{-J_2(\alpha)}  
+ T^{ -(1-\alpha)  \left[\frac{\delta}{3+2\delta}  \wedge \frac{1}{3}\right] }+\tmix^{\frac{1}{6}} T^{-\frac{1}{6}} \right).
\end{equation}
\end{proof}

\subsection{Proof of Corollary~\ref{cor:optimal-rate}}

\begin{proof}[Proof of Corollary~\ref{cor:optimal-rate}]
We proceed with the proof by discussing two scenarios.
	\paragraph{Linear SA with i.i.d. data}
	We first consider a simple case that is linear SA with i.i.d. data.
	In this case, $\tmix=0$ and $c_r = 0$ so that the second term in~\eqref{eq:rate-bound} disappear and the bound~\eqref{eq:rate-bound} becomes
	\[
	 \TOM \left(T^{-J_1(\alpha)}
	+ T^{ -(1-\alpha)  \left[\frac{\delta}{3+2\delta}  \wedge \frac{1}{3}\right] }+\tmix^{\frac{1}{6}} T^{-\frac{1}{6}} \right)
	= \TOM \left(
	T^{-h_1(\alpha)} 
	\right)
	\]
	where $J_1(\cdot)$ is defined in~\eqref{eq:J1} and
	\begin{equation}
			\label{eq:h-help-4}
		h_1(\alpha) = \min \left\{
		J_1(\alpha), (1-\alpha)  \left[\frac{\delta}{3+2\delta}  \wedge \frac{1}{3}\right]
		\right\}.
	\end{equation}

	In the following, we maximize~\eqref{eq:h-help-4} by considering different values of $\delta$.
	To ensure the optimal $\alpha^*$ is achievable, we consider $\alpha \in [0.5+\eps, 1)$ for a very small $\eps > 0$.  
	Note that $J_1(\alpha)$ strictly increases in $\alpha$ and has a unique intersection point with the straight line $\frac{\delta (1 - \alpha)}{3+2\delta}$ on the interval $[0, 1]$.
	\begin{enumerate}
		\item If $\delta \in \left(0, \frac{1-2\eps}{1+2\eps}\right]$, we then have $0.5+\eps \le \frac{1}{1+\delta}$.
		\eqref{eq:h-help-4} becomes  $\min \left\{  \frac{\delta(1-\alpha)}{3+2\delta} , \frac{\alpha(1+\delta)}{3+2\delta}
		\right\} $.
		One can show that, $ \frac{\alpha(1+\delta)}{3+2\delta}$ intersect with $\frac{\delta (1 - \alpha)}{3+2\delta}$ at $\alpha_1 := \frac{\delta}{2\delta + 1}$ which doesn't lie in the interval we consider.
		Hence, $\max\limits_{\alpha \in [0.5+\eps, 1)}  h_1(\alpha)  = \max\limits_{\alpha \in [0.5+\eps, 1)}  \frac{\delta(1-\alpha)}{3+2\delta} = \frac{\delta(1-2\eps)}{6 + 4\delta}$.
		\item  If $\delta \in \left[\frac{1-2\eps}{1+2\eps}, 3\right]$, we then have $\frac{1}{1+\delta} \le 0.5+\eps$.
		\eqref{eq:h-help-4} becomes $\min \left\{  \frac{\delta(1-\alpha)}{3+2\delta} , \frac{\alpha}{2+\alpha}
		\right\} $.
		Denote the intersection point between $\frac{\delta (1-\alpha)}{3+2\delta}$ and $\frac{\alpha}{2+\alpha}$ by $\alpha_2$.
		Direct calculation yields $\alpha_2 = \frac{\sqrt{9\left(1+\delta\right)^2 + 8\delta^2} - 3(1+\delta)}{2\delta}$ and $\alpha_2 < 0.5$ for all $\delta \le 3$.
		It implies the two segments doesn't intersect at the given interval.
		Hence, $\max\limits_{\alpha \in [0.5+\eps, 1)} h_1(\alpha) =  \max\limits_{\alpha \in [0.5+\eps, 1)}\frac{\delta(1-\alpha)}{3+2\delta} = \frac{\delta(1-2\eps)}{6 + 4\delta}$.
		\item If $\delta \in \left[3, \infty\right)$,\eqref{eq:h-help-4} becomes $ \min \left\{  \frac{1-\alpha}{3}, \frac{\alpha}{2+\alpha}
		\right\} $.
		Denote the intersection point between $\frac{1-\alpha}{3}$ and $\frac{\alpha}{2+\alpha}$ by $\alpha_3$.
		Direct calculation yields $\alpha_3 =\sqrt{6}-2 < 0.5$.
		It implies the two curves doesn't intersect at the given interval.
		So,$\max\limits_{\alpha \in [0.5+\eps, 1)} h_1(\alpha) = \max\limits_{\alpha \in [0.5+\eps, 1)} \frac{1-\alpha}{3} = \frac{1-2\eps}{6}$.
	\end{enumerate}
	Putting pieces together, we have
	\[
	\min_{\alpha \in [0.5+\eps, 1) } \dP P\left(\ThetaSym^\top\ph_T,\ThetaSym^\top \Bpsi \right)  
	=  \TOM\left(T^{-f_1(\delta)}  \right)
	\]
	where
	\begin{equation}
		\label{eq:f1}
		f_1(\delta) = 
		\left[ \frac{\delta}{6+4\delta} \wedge \frac{1}{6}\right](1-2\eps).
	\end{equation}
	
		\paragraph{Other cases}
		One can show that $J_1(\alpha) \ge J_2(\alpha)$ for any $\alpha \in (0.5, 1)$.
		Once $\tmix > 0$ or $c_r > 0$, 
		the bound~\eqref{eq:rate-bound} becomes
		\[
	 \TOM \left( (c_r+\tmix)^{\frac{p}{2+p} }  \cdot T^{-J_2(\alpha)}  
	+ T^{ -(1-\alpha)  \left[\frac{\delta}{3+2\delta}  \wedge \frac{1}{3}\right] }+\tmix^{\frac{1}{6}} T^{-\frac{1}{6}} \right).
		\]
		where $J_2(\cdot)$ is defined in~\eqref{eq:J2} and
		\begin{equation}
			\label{eq:h-help-3}
			h_2(\alpha) = \min \left\{
			J_2(\alpha), (1-\alpha)  \left[\frac{\delta}{3+2\delta}  \wedge \frac{1}{3}\right]
			\right\}.
		\end{equation}
	One can find that $J_2(\alpha)$ and $\frac{\delta (1-\alpha)}{3+2\delta}$ intersect at a unique point.
	Denote a polynomial function $\ell$ by $\ell(\delta) := 4\delta^3+7\delta^2-2\delta -3$.
	One can find that (i) $\ell(\delta)$ strictly increases in $\delta \in (0.5, \infty)$ and (ii) there exists a unique $\delta_0 \in (0.5, 1)$ such that $\ell(\delta_0) = 0$.

		In the following, we maximize~\eqref{eq:h-help-3} by considering different values of $\delta$.
	\begin{enumerate}
		\item If $\delta \in (0, \delta_0]$,  denote the solution of $\frac{\delta (1-\alpha)}{3+2\delta}  = (\alpha -0.5)\frac{1+\delta}{2+\delta}$ by $\alpha_1$.
		Direct calculation yields $\alpha_1 = \frac{4\delta^2+9\delta + 3}{6\delta^2 + 14 \delta + 6}$.
		One can show that $0.5 < \alpha_1 \le \frac{1}{1+\delta}$.
		The right-hand side inequality is equivalent to $\ell(\delta) := 4\delta^3+7\delta^2-2\delta -3 \le 0$, which is true because $\delta \le \delta_0$.
		Hence, $\max\limits_{\alpha \in (0.5, 1)} h_2(\alpha) =  \frac{\delta(2\delta^2 + 5\delta + 3)}{2(3+2\delta)(3\delta^2 + 7\delta + 3)} = \frac{\delta(\delta+1)}{2(3\delta^2 + 7\delta + 3)}$.
		
		\item If $\delta \in [\delta_0, 3]$, denote the solution of $\frac{\delta (1-\alpha)}{3+2\delta} =\frac{\alpha- 0.5}{\alpha + 1}$ by $\alpha_2$.
		Direct calculation yields $\alpha_2 =\frac{\sqrt{(3+2\delta)^2+2\delta(3+4\delta)} - (3+2\delta)}{2\delta} > 0.5$.
		Once can show that $\alpha_2 \ge \frac{1}{\delta + 1}$.
		This is because the inequality is equivalent to  $\ell(\delta) := 4\delta^3+7\delta^2-2\delta -3 \ge 0$ which is true because $\delta \ge \delta_0$.
		Hence, $\max\limits_{\alpha \in (0.5, 1)} h_2(\alpha) =  \frac{3+4\delta - \sqrt{(3+2\delta)^2 + 2\delta(3+4\delta)}}{2(3+2\delta)}$.
		
		\item If $\delta \in [3, \infty)$, denote the solution of $\frac{ 1-\alpha}{3} =\frac{\alpha- 0.5}{\alpha + 1}$ by $\alpha_3$.
		Direct calculation yields $\alpha_3 = \frac{\sqrt{19}-3}{2}$ and $1 > \alpha_3 > 0.5 > \frac{1}{1+\delta}$.
		Hence, $\max\limits_{\alpha \in (0.5, 1)} h_2(\alpha) =  \frac{5-\sqrt{19}}{6}$
	\end{enumerate}
	Putting pieces together, we have
	\[
\min\limits_{\alpha \in (0.5, 1)}  \dP\left(\ThetaSym^\top\ph_T,\ThetaSym^\top \Bpsi \right)  
	=  \gO\left(\left[(c_r + \tmix)^{\frac{p}{2+p}} + 1\right]  \cdot T^{-f_2(\delta)}  \right),
	\]
	where
	\begin{equation}
		f_2(\delta) = 
		\left\{\begin{array}{ll}
			\frac{\delta(2\delta^2 + 5\delta + 3)}{2(3+2\delta)(3\delta^2 + 7\delta + 3)}  &  \ \text{if} \  \delta \in (0, \delta_0], \\
			\frac{3+4\delta - \sqrt{(3+2\delta)^2 + 2\delta(3+4\delta)}}{2(3+2\delta)} &\ \text{if} \  \delta \in [\delta_0, 3],   \\
			\frac{5-\sqrt{19}}{6} & \ \text{if} \ \delta \in [3, \infty). \\
		\end{array}
		\right.
	\end{equation}
\end{proof}

\subsection{Proof of Lemma~\ref{lem:moment}}
\label{proof:moment}
\begin{proof}[Proof of Lemma~\ref{lem:moment}]
	We will analyze each term in~\eqref{eq:finer-decomposition} respectively.
	 For simplicity, we define
	 \[
	 C_{U, \x_t} =  \kappa \tmix \cdot (2L_H \|\x_t-\x^{\star}\|+\sigma).
	 \]
	\paragraph{For $\ph_T- \widetilde{\ph}_T$} 
	Recall $p=2(1+\delta)$ and let $m \in [0, 2\delta+1]$ such that $1 \le 1+m \le p$.
	It follows that
	\begin{align*}
		\dP\left( \ThetaSym^\top{\ph}_T, \ThetaSym^\top\widetilde{\ph}_T\right) 
		&\overset{(a)}{\le}\dP\left({\ph}_T, \widetilde{\ph}_T \right)  
		\overset{(b)}{\le} \widetilde{d} \left( \frac{1}{\sqrt{T}}\sum_{t=0}^{\floor{Tr}} \eta_t \PM\sU(\x_t, \xi_{t-1}) \right) \nonumber \\
		&\overset{(c)}{\le} \left(
		\EB \sup_{r \in [0, 1]} \left\| \frac{1}{\sqrt{T}}\sum_{t=0}^{\floor{Tr}} \eta_t \PM\sU(\x_t, \xi_{t-1}) \right\|^{m+1}
		\right)^{\frac{1}{m+2}} \nonumber \\
		&\overset{(d)}{\le} \left(  T^{\frac{m+1}{2}}  \EB \left(
		\frac{1}{T}\sum_{t=0}^{T} \eta_t C_{U, \x_t}\right)^{1+m}
		\right)^{\frac{1}{m+2}} \\
		&\overset{(e)}{\precsim}
		\left(  T^{\frac{m+1}{2}}  \tmix^{m+1} \cdot \frac{1}{T}\sum_{t=0}^T \eta_t^{m+1} (\EB\|\x_t-\x^{\star}\|^{m+1} + \sigma^{m+1} )  \right)^{\frac{1}{m+2}}
		\\
		&\overset{(f)}{\precsim} 
		 \OM  \left(  T^{\frac{m+1}{m+2}} \cdot \tmix^\frac{m+1}{m+2}  \cdot \left(  \frac{1}{T} \sum_{t=0}^T \eta_t^{m+1} \right)^{\frac{1}{m+2}}   \right), 
	\end{align*}
	where $(a)$ uses Proposition~\ref{prop:one_on_pkhv}, $(b)$ follows from $\widetilde{\ph}_T(r) = {\ph}_T(r)-\frac{1}{\sqrt{T}}\sum_{t=0}^{\floor{Tr}} \eta_t \PM\sU(\x_t, \xi_{t-1})$ and Proposition~\ref{prop:dstb_on_pkhv}, $(c)$ follows from Proposition~\ref{prop:pkhv_to_mmt}, $(d)$ uses the fact that $\|\PM\sU(\x_t, \xi_{t-1})\| \le C_{U, \x_t}$ from Lemma~\ref{lem:poisson}, $(e)$ uses Jensen's inequality, and $(f)$ uses Assumption~\ref{asmp:x} .

	\paragraph{For $\Bpsi_0$} 
	From Lemma~\ref{lem:A}, we know that $\sA_j^n$ is uniformly bounded. 
	Hence, as $T\to \infty$,
	\begin{equation*}
		\vertiii{\Bpsi_0} = 
		\sup_{r \in [0, 1]}
		\|\Bpsi_0(r)\| = \frac{1}{\sqrt{T}\eta_0}\sup\limits_{r\in[0,1]}\|\sA_0^{\floor{Tr}}\sB_0\De_0\| = \gO\left(\frac{1}{\sqrt{T}}\right) .
	\end{equation*}
	Because $\Bpsi_0(\cdot)$ is a deterministic process (given $\gF_0$), it's easy to show that $\widetilde{d}(\Bpsi_0) = \gO(T^{-1/2})$ (by letting $p \to \infty$ in Proposition~\ref{prop:pkhv_to_mmt}).

	\paragraph{For $\Bpsi_{1,1}$} 
	Notice that $\Bpsi_{1,1}(r) =  \frac{1}{\sqrt{T}} \sum_{t=0}^{\floor{Tr}} \sA_t^{\floor{Tr}}\sr_t$.
	From the proof of Lemma~\ref{lem:error-analysis}, we know there exists $c_r := \max\left\{L_G, \frac{L_H +\|\sG\|}{\delta_G}\right\}$ such that
	\begin{align*}
			\|\sr_t\|&\le c_r\|\vx_t - \vx^{\star}\|^2 + \eta_t C_{U, \x_t} \\
			&\le 
		(c_r + \kappa \tmix)\|\x_t - \x^{\star}\|^2 + \eta_t  \kappa \tmix(\sigma + L_H^2 )\\
		&:= \widetilde{c}_r \|\x_t - \x^{\star}\|^2 + \eta_tC_U.
	\end{align*}
	Lemma~\ref{lem:A} implies that $\sA_j^n$ is uniformly bounded by a universal constant $C_0$ in the sense that $\|\sA_j^n\| \le C_0$ for all $j \le n$.
	Let $\lambda$ denote any positive number satisfying $0 \le \lambda \le \delta$.
	By the $(L^p, (1+ \log t)\sqrt{\eta_t})$-consistency assumption with $p=2+2\delta$, we upper bound the $(1+\lambda)$-th moment of $\|\Bpsi_1\|_{\infty}$ by Jensen's inequality as following
	\begin{align*}
		\EB \vertiii{\Bpsi_{1,1}}^{1+\lambda}
		&=\EB\sup\limits_{0\le r\le 1}\|\Bpsi_{1,1}(r)\|^{1+\lambda} = \EB\sup\limits_{0\le r\le 1}\left\|\frac{1}{\sqrt{T}}\ssum{t}{0}{\floor{Tr}}\sA_t^{\floor{Tr}}\sr_t\right\|^{1+\lambda}\\
		&\le \EB\left(\frac{1}{\sqrt{T}}\ssum{t}{0}{T}C_0\|\sr_t\|\right)^{1+\lambda}
		\le T^{\frac{1+\lambda}{2}}C_0^{1+\lambda} \EB \left(\frac{1}{T}\ssum{t}{0}{T}\|\sr_t\|\right)^{1+\lambda}\\
		&\le T^{\frac{1+\lambda}{2}}C_0^{1+\lambda} 2^{\lambda} \left[ 	\widetilde{c}_r^{1+\lambda}\EB\left(\frac{1}{T}\ssum{t}{0}{T}\|\vx_t - \vx^{\star}\|^2\right)^{1+\lambda}
		+C_U^{1+\lambda} \left( \frac{1}{T}  \ssum{t}{0}{T} \eta_t \right)^{1+\lambda}
		\right]\\
		&\le  T^{\frac{1+\lambda}{2}}C_0^{1+\lambda}
		2^{\lambda} \left[ 	\widetilde{c}_r^{1+\lambda}\frac{1}{T}\ssum{t}{0}{T} \EB\|\vx_t - \vx^{\star}\|^{2(1+\lambda)}
		+C_U^{1+\lambda}  \frac{1}{T}  \ssum{t}{0}{T} \eta_t^{1+\lambda}
		\right]\\
			&\le  T^{\frac{1+\lambda}{2}}C_0^{1+\lambda}
	2^{\lambda} \left[ 	\widetilde{c}_r^{1+\lambda}\frac{1}{T}\ssum{t}{0}{T}  \eta_t^{1+\lambda} C_p \log^p T
	+C_U^{1+\lambda}  \frac{1}{T}  \ssum{t}{0}{T} \eta_t^{1+\lambda}
	\right].
	\end{align*}
	As a result of Proposition~\ref{prop:pkhv_to_mmt} with $p=1+\lambda$, we get
	\begin{align*}
			\widetilde{d}(\Bpsi_{1,1}) 
		\le (\EB \vertiii{\Bpsi_{1,1}}^{1+\lambda})^{\frac{1}{2+\lambda}}
		&= \TOM \left(
		\left(\widetilde{c}_r +  C_U\right)^{\frac{1+\lambda}{2+\lambda}} \cdot 	T^{\frac{1+\lambda}{2(2+\lambda)}} \cdot  \left(\frac{1}{T}\ssum{t}{0}{T}  \eta_t^{1+\lambda}\right)^{\frac{1}{2+\lambda}}
		\right)\\
		&= \TOM \left(
		\left( c_r + \tmix \right)^{\frac{1+\lambda}{2+\lambda}} \cdot 	T^{\frac{1+\lambda}{2(2+\lambda)}} \cdot  \left(\frac{1}{T}\ssum{t}{0}{T}  \eta_t^{1+\lambda}\right)^{\frac{1}{2+\lambda}}
		\right).
	\end{align*}

	\paragraph{For $\Bpsi_{1,2}$} 
	Recall that $\Bpsi_{1,2}(r) =  \frac{1}{\sqrt{T}} \sum_{t=0}^{\floor{Tr}} \sA_t^{\floor{Tr}}\snu_t$.
	Note that $\frac{\eta_t-\eta_{t+1}}{\eta_t}=1-\left(1-\frac{1}{t+1}\right)^\alpha\le1-\exp(-\frac{\alpha}{t})\le\frac{\alpha}{t} \le \alpha \eta_t$.
	By the definition of $\snu_t$ in~\eqref{eq:nu} and the inequality~\eqref{eq:help-nu-0}, we have
	\begin{align}
		\label{eq:snu_bound}
			\|\snu_t\|  
			&\le  L_U \|\x_{t+1} - \x_t\| + \left| \frac{\eta_{t+1}-\eta_t}{\eta_t} \right| \cdot C_{U, \x_{t+1}}  \nonumber \\
			&\le L_U  \|\x_{t+1} - \x_t\|  + \alpha \kappa \tmix \eta_t \cdot (2L_H \|\x_{t+1}-\x^{\star}\|+\sigma) \nonumber \\
			&\le (L_U + \alpha \kappa \tmix) \left(
			\|\x_{t+1} - \x_t\|  + \eta_t \|\x_{t+1}-\x^{\star}\|
			\right) + \eta_t \cdot  \alpha \kappa  \sigma\tmix
	\end{align}
	where $L_U = \OM(L_H(1 + \kappa \tmix))$ is given in Lemma~\ref{lem:poisson}.
	Let $0 \le m \le 2\delta+1$ be any real number.
	
	We assert that there exists a positive constant $C_{1,2} > 0$ so that
	\begin{equation}
		\label{eq:12help}
			\EB \left(
		\|\x_{t+1} - \x_t\|  + \eta_t \|\x_{t+1}-\x^{\star}\|
		\right)^{1+m} \precsim C_{1,2}^{1+m} \eta_t^{1+m}.
	\end{equation}
	We prove this statement in the following.
First, from Assumption~\ref{asmp:futher-noise}, $\x_t-\x^{\star}$ has uniformly bounded $p$-th order moments and thus $\sup_{t \ge 0} (\EB \|\x_t-\x^{\star}\|^p)^\frac{1}{p} < \infty$.
Second, it follows that $\EB \|\x_{t+1} - \x_t\|^{1+m} = \eta_t^{1+m} 	\EB \|\sH(\x_t, \xi_t)\|^{1 + m} $ and
	\begin{align*}
	\EB \|\sH(\x_t, \xi_t)\|^{1 + m} 
	&\le 2^{m} \left[
	\EB \|\sH(\x_t, \xi_t)-\sH(\x^{\star}, \xi_t)\|^{1 + m}  + \EB \|\sH(\x^{\star}, \xi_t)\|^{1 + m} 
	\right] \\
	& \overset{(a)}{\le} 2^{m} \left[ L_H^{1+m}
	\EB \|\x_t -\x^{\star} \|^{1 + m}  + \EB \|\sH(\x^{\star}, \xi_t)\|^{1 + m} 
	\right] \\
	&\overset{(b)}{\le}2^{m} \left[ L_H^{1+m}
	\left(\sup_{t \ge 0}\EB \|\x_t -\x^{\star} \|^{p} \right)^\frac{1+m}{p}  + \sup_{t \ge 0} \left(\EB \|\sH(\x^{\star}, \xi_t)\|^{p} \right)^{\frac{1+m}{p}}
	\right].
\end{align*}
where $(a)$ uses Assumption~\ref{asmp:H}, $(b)$ uses Jensen's inequality, and $(c)$ uses Assumption~\ref{asmp:noise}.
Combing the last two points, we know that~\eqref{eq:12help} with $C_{1,2}$ depending on universal constants as well as $\sup_{t \ge 0} \left(\EB \|\sH(\x^{\star}, \xi_t)\|^{p} \right)^{\frac{1}{p}}, \sup_{t \ge 0} \left( \EB\|\x_t -\x^{\star} \|^{p} \right)^\frac{1}{p}$, and $L_H$.

Therefore,
	\begin{align*}
		\EB  \|\snu_t\|^{1+m}  
		&\le
		2^{1+m}(L_U + \alpha \kappa \tmix)^{1+m} C_{1,2}^{1+m} \eta_t^{1+m} + \left( 2  \alpha \kappa  \sigma\tmix \cdot \eta_t \right)^{1+m}\\
		&\le (2C_{1,2} (L_U+\alpha \kappa \tmix) + 2\alpha \kappa \sigma \tmix )^{1+m}\eta_t^{1+m} \\
		&\le (\tmix + 1)^{1+m} C_{1,3}^{1+m} \eta_t^{1+m}
	\end{align*}
	where the first inequality follows from applying Jensen's inequality to~\eqref{eq:snu_bound} and plugging~\eqref{eq:12help} into it and the last inequality enlarges $C_{1,2}$ to $C_{1,3}$ to simplify notation.
	Using the last inequality, we have
	\begin{align*}
		\EB \vertiii{\Bpsi_{1,2}}^{1+m}
		&=\EB\sup\limits_{0\le r\le 1}\|\Bpsi_{1,2}(r)\|^{1+m} 
		= \EB\sup\limits_{0\le r\le 1}\left\|\frac{1}{\sqrt{T}}\ssum{t}{0}{\floor{Tr}}\sA_t^{\floor{Tr}}\snu_t\right\|^{1+m}\\
		&\le \EB\left(\frac{1}{\sqrt{T}}\ssum{t}{0}{T}C_0\|\snu_t\|\right)^{1+m}\\
		&\le T^{\frac{1+m}{2}}C_0^{1+m} \EB\left(\frac{1}{T}\ssum{t}{0}{T}\|\snu_t\|\right)^{1+m}
		\\
		&\le T^{\frac{1+m}{2}}C_0^{1+m} \frac{1}{T}\ssum{t}{0}{T}\EB\|\snu_t\|^{1+m}
		\\
		&\precsim T^{\frac{1+m}{2}} (1+\tmix)^{1+m} \cdot \frac{1}{T}\ssum{t}{0}{T}\eta_t^{1+m}.
	\end{align*}
	As a result of Proposition~\ref{prop:pkhv_to_mmt} with $p=1+m$, we get
	\begin{equation*}
		\widetilde{d}(\Bpsi_{1,2}) 
		\le (\EB\|\Bpsi_{1,2}\|_{\infty}^{1+m})^{\frac{1}{2+m}}
		=\widetilde{\gO}\left(
		\left(1+\tmix\right)^{\frac{1+m}{2+m}} \cdot T^{\frac{1+m}{2(2+m)}} \cdot \left( \frac{1}{T}\ssum{t}{0}{T}\eta_t^{1+m}\right)^{\frac{1}{2+m}}
		\right).
	\end{equation*}

\paragraph{For $\Bpsi_2$}
Notice that $\ssum{t}{0}{k}(\sA_t^T - \sG^{-1})\vu_t $ is a martingale with the natural filtration $\gF_k$. By Doob's inequality,
\begin{align*}
	\EB\sup\limits_{r\in[0,1]}\|\Bpsi_2(r)\|_2^2 &\le \frac{4}{T}\ssum{t}{0}{T}\EB\|(\sA_t^T - \sG^{-1})\vu_t\|_2^2 \\
	&\le 4\sup\limits_{t\ge 0}\EB\|\vu_t\|_2^2\cdot \frac{1}{T}\ssum{t}{0}{T}\|\sA_t^T - \sG^{-1}\|_2^2.
\end{align*}
We then need to analyze the order of $\|\sA_t^T - \sG^{-1}\|_2$. 
To that end, we introduce another quantity 
\begin{equation}
	\label{eq:D}
	\sD_t^n := \ssum{j}{t}{n}\eta_{j+1}\prod\limits_{i=t}^{j}(\sI- \eta_i\sG).
\end{equation}

\begin{lem}\label{lem:vanish_A_rate}
	There exists two constants $c, c_0 > 0$ such that for all $n \ge t \ge0$,
	\[
	\|\sD_t^n - \sG^{-1}\|_2 \le \eta_{t} + c_0\exp\left\{-c\ssum{i}{t}{n+1}\eta_i\right\}\|\sG^{-1}\|_2
	\quad \text{and} \quad
		\left\| \sA_{t-1}^n - \sD_t^n\right\|_2 =  \gO(t^{\alpha -1})
	\]
	where we hide dependence $\alpha$ and other universal constant factors.
\end{lem}
The proof of Lemma~\ref{lem:vanish_A_rate} is provided in Section~\ref{proof:vanish_A_rate}.
% owing to the proof of Lemma 3.4.1 in \citet{chen2002stochastic}, we can bound the gap between $\sA_{t-1}^n$ and $\sD_t^n$. In fact, note that we suppose $\eta_i$ has the form $i^{-\alpha}$
By Lemma~\ref{lem:vanish_A_rate} and triangular inequality, we have
\[
\|\sA_t^n - \sG^{-1}\|_2 = \gO\left(t^{\alpha - 1} + \exp\left\{-c\ssum{i}{t}{n+1}\eta_i\right\}\right)
\]
Therefore,
\begin{align*}
	\frac{1}{T}\ssum{t}{0}{T}\|\sA_t^T - \sG^{-1}\|_2^2 &= \frac{\OM(1)}{T}\ssum{t}{0}{T}\left(t^{2\alpha - 2} + \exp\left\{-2c\ssum{i}{t}{T+1}\eta_i\right\}\right)\\
	&=\OM\left( T^{2\alpha - 2} + \frac{1}{T\eta_T} \cdot \eta_T\ssum{t}{1}{T}\exp\left\{-2c\ssum{i}{t}{T}\eta_i\right\}\right) \\
	&= \gO\left(T^{2\alpha - 2} +\frac{1}{T\eta_T}\right) = \gO (T^{\alpha-1}),
\end{align*}
where the last equation holds by the fact $\eta_T\ssum{t}{1}{T}\exp\left\{-2c\ssum{i}{t+1}{T}\eta_i\right\} \to 1$ as $T\to \infty$ and thus is uniformly bounded.
One can prove it by using Stolz–Cesàro theorem.
Thus, by setting $p=2$ in Proposition~\ref{prop:pkhv_to_mmt}, we know that
\begin{equation*}
	\widetilde{d}(\Bpsi_2) 
	\le (\EB \vertiii{\Bpsi_{2}}^2)^{1/3}
	\precsim (\EB \sup_{r \in [0, 1]} \|\Bpsi_2(r)\|_2^2)^{1/3}
	= \gO\left(T^{\frac{\alpha-1}{3}}\right).
\end{equation*}

\paragraph{For $\Bpsi_3$}
In our previous asymptotic result, we establish Lemma~\ref{lem:error0} to analyze the term $\Bpsi_3$.
In order to provide an quantitative result, we need to capture the exact convergence rate in Lemma~\ref{lem:error0}, which is equivalent to analyze the moments of decomposed errors therein.
Thanks to our technique developed therein, it is possible to do that.
In the following, we will use the same notation in the proof of Lemma~\ref{lem:error0} for the sake of consistency and quick understanding.

\begin{lem}\label{lem:error1}
	Assume the same assumptions in Lemma~\ref{lem:error} and let $\{\vy_t\}_{t \ge0}$ be defined in~\eqref{eq:y}.
	If we set $\eta_t = t^{-\alpha}$,  then for any $ 0 \le l \le \delta$ where $p=2+2\delta$, we have
	\begin{equation}
	\tag{\ref{eq:p-rate}}
	\widetilde{d}\left(\bar{\vy}_T\right) = \gO\left((1+l) \cdot {T^{-\frac{l(1-\alpha)}{3+2l}}}\right)
	\quad \text{where} \quad
	\bar{\vy}_T(r) = 
	\frac{\vy_{\floor{(T+1)r}}}{\sqrt{T}\eta_{\floor{(T+1)r}}}
	\quad \text{for} \quad r \in [0, 1].
	\end{equation}
\end{lem}

The proof of Lemma~\ref{lem:error1} can be found in Section~\ref{proof:error1}.
With Lemma~\ref{lem:error1}, we are ready to bound $\widetilde{d}(\Bpsi_3)$.
By~\eqref{eq:bpsi_30}, we have
\[
\vertiii{\Bpsi_3}= \sup_{r \in [0, 1]} \|\Bpsi_3(r)\| \precsim \sup_{n \in [T]} \left\|  \frac{1}{\sqrt{T}}
\frac{1}{\eta_{n+1}}\sum_{t=0}^n \left(\prod_{i=t+1}^n \sB_i\right)
\eta_t \su_t \right\| := \sup_{r \in [0, 1]} \|\bar{\vy}_T(r)\|
=\vertiii{\bar{\vy}_T}
\]
where we define $\bar{\vy}_T(r) = 
\frac{\vy_{\floor{(T+1)r}}}{\sqrt{T}\eta_{\floor{(T+1)r}}}$ and $\vy_{n+1} = \sum_{t=0}^n \left(\prod_{i=t+1}^n \sB_i\right)
\eta_t \su_t$ in the last inequality.
By the definition of $\widetilde{d}(\cdot)$ and Lemma~\ref{lem:error1}, 
\begin{equation*}
	\widetilde{d}(\Bpsi_3) = \inf\limits_\eps \eps\vee \PB(\vertiii{\Bpsi_3} > \eps)
	\precsim \inf\limits_\eps \eps\vee \PB(\vertiii{\bar{\vy}_T} > \eps)
	=\widetilde{d}(\bar{\vy}_T) = \TOM\left((1+l) \cdot T^{-\frac{l(1-\alpha)}{3+2l}}\right).
\end{equation*}

\paragraph{For $\Bpsi_{4,1}$}
Let $k$ by any real number satisfying $1 \le k \le 2 + 2\delta$.
By Burkholder-Davis-Gundy inequality, it follows that
\begin{align*}
	\EB\sup\limits_{0\le t\le T} \left\|\frac{1}{\sqrt{T}}\ssum{j}{0}{t}\vu_{j,1}\right\|^k
	&\le \frac{(c_3 k)^{k/2}}{T^{k/2}}\EB\left(\ssum{t}{1}{T}\EB\left[\vu_{t,1}^2|\gF_{t-1}\right]\right)^{k/2}\\
	&\overset{(a)}{\precsim} \frac{(c_3k)^{k/2}}{T^{k/2}}\EB\left(\ssum{t}{1}{T}\|\vx_t - \vx^{\star}\|^2\right)^{k/2}\\
	&\overset{(b)}{\precsim} \frac{(c_3k)^{k/2}}{T}\EB\ssum{t}{1}{T}\|\vx_t^{\star} - \vx^{\star}\|^k \\
	&\overset{(c)}{\precsim} \frac{(c_3k)^{k/2}C_k^k}{T}\ssum{t}{1}{T}\eta_t^{k/2} \log^{k} T
\end{align*}
where $(a)$ holds because $\EB\left[\vu_{t,1}^2|\gF_{t-1}\right] \precsim \EB\|\vx_t - \vx^{\star}\|^2$ as a result of Assumption~\ref{asmp:H}, $(b)$ follows from Jensen's inequality, $(c)$ holds owing to the $(L^p,(1+\log t)\sqrt{\eta_t})$-consistency that implies $\EB\|\vx_t^{\star} - \vx^{\star}\|^k  \le C_k^k \eta_t^{k/2} \log^{k} T$.
The last inequality together with Proposition~\ref{prop:pkhv_to_mmt} implies that
\begin{align*}
	\widetilde{d}(\Bpsi_{4,1}) 
	\le \left(\EB\sup\limits_{0\le t\le T}\left\|\frac{1}{\sqrt{T}}\ssum{t}{0}{\floor{Tr}}\sG^{-1}\vu_{t,1}\right\|^k\right)^{\frac{1}{k+1}} = \TOM\left( \sqrt{k} C_k  \cdot  \left( \frac{1}{T} \sum_{t=0}^T \eta_t^{k/2} \right)^{\frac{1}{1+k}}   \right).
\end{align*}

\paragraph{For $\Bpsi_{4,2}$}
Recall that $\Bpsi_{4,2}(r) := \frac{1}{\sqrt{T}}\ssum{t}{0}{\floor{Tr}}\ThetaSym^\top\sG^{-1}\vu_{t,2}$ with $\vu_{t,2} = \sU(\x^{\star}, \xi_t) - \PM \sU(\x^{\star}, \xi_{t-1})$ and $\Bpsi(r) := \ThetaSym^\top\sG^{-1}\sS^{1/2}\sW(r)$.
We will apply Theorem~\ref{thm:rate_fclt_mkv} to bound the L\'evy-Prokhorov distance between them.
Since Theorem~\ref{thm:rate_fclt_mkv} holds only for $0 < \delta < 3/2$, we denote $\delta^\prime = \delta\wedge (\frac{3}{2}-o(1))$ for very sufficiently small $o(1)$.\footnote{We can always set the term $o(1)$ as small as expected, which is the reason we denote it by an infinitesimal $o(1)$.}

First, the quadratic variation process of $\Bpsi_{4,2}$ is given by 
\begin{equation}
	\label{eq:u2-quadratic}
	\left\langle \Bpsi_{4,2}(\cdot) \right\rangle_r
	= \frac{1}{T} \ssum{t}{0}{\floor{Tr}} \EB [(\ThetaSym^\top\sG^{-1}\vu_{t,2})^2|\FM_{t-1}]
	= \frac{1}{T} \ssum{t}{0}{\floor{Tr}}  \ThetaSym^\top\sG^{-1} \EB[\vu_{t,2}\vu_{t,2}^\top|\FM_{t-1}]  \sG^{-\top} \ThetaSym.
\end{equation}
Second, note that the partial-sum process $\Bpsi_{4,2}$ is c\`adl\`ag (that is right continuous with left limits) with all discontinuous points given by $\{t/T\}_{t \in [T]}$.
Hence, its corresponding dual predictable projection is the point measure in $[0,1]\times \RB$ (similar to the definition of the Poisson point process) and thus we can compute the following integral and obtain
\begin{equation}
	\label{eq:dual-pred}
	\EB\int_0^1\int_{\RB}|x|^{2+2\delta'}\Pi^n(ds,dx) = \EB\ssum{t}{0}{T}\frac{1}{T^{1+\delta'}}\left|\ThetaSym^\top \sG^{-1}\vu_{t,2}\right|^{2 +2\delta'} \le C_{4,2}^{2+2\delta'} T^{-\delta'},
\end{equation}
where $C_{4,2} = \| \sG^{-1} \| \cdot \sup_{t \ge 0} (\EB \|\su_{t,2}\|^{p} )^\frac{1}{p} < \infty$ due to Assumption~\ref{asmp:noise}.

By Theorem~\ref{thm:rate_fclt_mkv}, it follows that
\begin{align}
	\dP(\ThetaSym^\top\Bpsi_{4,2}, \ThetaSym^\top\Bpsi)
	&= 
	\widetilde{\gO}\left(  T^{-\frac{\delta'}{3+2\delta'}} +
	\left[\EB\sup\limits_{r \in [0, 1]}\left|	\left\langle \Bpsi_{4,2}(\cdot) \right\rangle_r - 	\left\langle \Bpsi(\cdot) \right\rangle_r \right|\right]^{\frac{1}{3}} 
	\right).  \label{eq:u-2-bound}
\end{align}
The second term in~\eqref{eq:u-2-bound} is the expected supreme absolute difference between the quadratic variation processes of $\Bpsi_{4,2}$ and $\Bpsi$ over the fraction $r \in [0, 1]$.
We analyze that term in Lemma~\ref{lem:quad_cha_bd} whose proof is deferred in Section~\ref{proof:quad_cha_bd}.
\begin{lem}\label{lem:quad_cha_bd}
	Rewriting $p = 2+2\delta$ with $p$ given in Assumption~\ref{asmp:noise}.
	For simplicity, we denote by
	\[
	q(\xi_{t-1}) := \EB\left[(\ThetaSym^\top\sG^{-1}\su_{t,2})^2| \gF_{t-1}\right]
	\quad \text{with} \quad
	\su_{t,2} = \sU(\x^{\star}, \xi_t)-\PM \sU(\x^{\star}, \xi_{t-1}).
	\]
	Under Assumption~\ref{asmp:futher-noise}, $\EB q(\xi_t) = \ThetaSym^\top\sG^{-1}\sS\sG^{-T}\ThetaSym$ for all $t \ge 0$.
	Then
	\[
	\EB\sup\limits_{t\le T}\left|\ssum{i}{0}{t}\{q(\xi_i)- \EB_{\xi_i} q(\xi_i) \}\right| = \OM \left( 	\sqrt{T \tmix } \right)
	\]
	where $\OM(\cdot)$ hides factors depending on $\|\sG^{-1}\|, C_U, \kappa$ and $ \sup_{\xi \in \Xi} \PM\|\sH(\x^{\star}, \xi)\|^2$.
\end{lem}

Using the notation in Lemma~\ref{lem:quad_cha_bd}, we denote $q(\xi_{t-1}) := \EB\left[(\ThetaSym^\top\sG^{-1}\su_{t,2})^2| \gF_{t-1}\right]$. Then the quadratic variation of $\Bpsi_{4,2}$ can be expressed in terms of $q(\xi_{t-1})$'s as what follows
\[
\left\langle \Bpsi_{4,2}(\cdot) \right\rangle_r  = \left\langle \frac{1}{\sqrt{T}}\ssum{t}{0}{\floor{T\cdot}}\ThetaSym^\top\sG^{-1}\vu_{t,2} \right\rangle_r 
= \frac{1}{T} \sum_{t=1}^{\floor{Tr}} q(\xi_{t-1}).
\]
By Lemma~\ref{lem:quad_cha_bd}, we have  $\EB q(\xi_{t-1}) = \ThetaSym^\top\sG^{-1}\sS\sG^{-T}\ThetaSym$ for all $t \ge 1$.
Therefore, 
\begin{align*}
\EB\sup\limits_{r \in [0, 1]}\left|	\left\langle \Bpsi_{4,2}(\cdot) \right\rangle_r - 	\left\langle \Bpsi(\cdot) \right\rangle_r \right|
&\le  \EB \sup_{n \in [T]}\frac{1}{T}  \left| \sum_{t=1}^{n} \left\{ q(\xi_{t-1}) - \EB q(\xi_{t-1})\right\}  \right|  \\
& \qquad + 
 \sup_{r \in [0, 1]}  \left| \left(\frac{\floor{Tr}}{T} - r\right)  \ThetaSym^\top\sG^{-1}\sS\sG^{-T}\ThetaSym \right| \\
&=  \OM\left( \sqrt{\frac{\tmix}{T}} \right) 
\end{align*}
\end{proof}

\subsection{Proof of Lemma~\ref{lem:vanish_A_rate}}
\label{proof:vanish_A_rate}

\begin{proof}[Proof of Lemma~\ref{lem:vanish_A_rate}]
	For the first part, it follows that
	\begin{align*}
		\sG\sD_t^n + \pprod{i}{t}{n+1}(\sI - \eta_i\sG) &= \ssum{j}{t}{n}\eta_{j+1}\pprod{i}{t}{j}(\sI - \eta_i\sG) + \pprod{i}{t}{n+1}(\sI - \eta_j\sG)\\
		&= \ssum{j}{t}{n-1}\eta_{j+1}\pprod{i}{t}{j}(\sI - \eta_i\sG) + (\sI - \eta_{n+1}\sG + \eta_{n+1}\sG)\pprod{i}{t}{n}(\sI - \eta_j\sG)\\
		&= \ssum{j}{t}{n-1}\eta_{j+1}\pprod{i}{t}{j}(\sI - \eta_i\sG) + \pprod{i}{t}{n}(\sI - \eta_j\sG)\\
		&=\sG\sD_t^{n-1} +  \pprod{i}{t}{n}(\sI - \eta_j\sG)\\
		&=\eta_{t+1}\sG(\sI - \eta_{t+1}\sG) + (\sI - \eta_t\sG)(\sI - \eta_{t+1}\sG)\\
		&= \sI - \eta_t\sG.
	\end{align*}
	Rearranging the last equation gives
	\[
	\sD_t^n - \sG^{-1} = -\eta_t\sI - \sG^{-1}\pprod{i}{t}{n+1}(\sI - \eta_i\sG).
	\]
	It follows from~\ref{lem:bounded-X} in Lemma~\ref{lem:A} that there exist two constant $c_0,~c >0$ so that $\left\|\pprod{i}{t}{n+1}(\sI - \eta_i\sG)\right\|_2 \le c_0\exp\left\{-c\ssum{i}{t}{n+1}\eta_i\right\}$ for all $n\ge t >0$. 
	We then complete the proof by triangular inequality.

For the second part, we bound the difference between $\sA_{t-1}^n$ and $\sD_t^n$ as following
\begin{align*}
	\left\| \sA_{t-1}^n - \sD_t^n\right\|_2 &= \left\|\eta_{t-1}\sI + \ssum{j}{t}{n}(\eta_{t-1} - \eta_{j+1})\pprod{i}{t}{j}(\sI - \eta_i\sG)\right\|_2\\
	&\le \eta_{t-1} + \ssum{j}{t}{n}\ssum{i}{t}{j+1} (\eta_{i-1} - \eta_i)\left\|\pprod{i}{t}{j}(\sI - \eta_i\sG)\right\|_2\\
	&\overset{(a)}{\le}\eta_{t-1} + \frac{2\alpha}{t} \ssum{j}{t}{n}\ssum{i}{t}{j} \eta_{i}\left\|\pprod{i}{t}{j}(\sI - \eta_i\sG)\right\|_2\\
	&\overset{(b)}{\le}\eta_{t-1} + \frac{2c_0\alpha}{t^{1-\alpha}} \ssum{j}{t}{n} \eta_{j+1}\ssum{i}{t}{j} \eta_{j}\exp\left\{-c\ssum{i}{t}{j}\eta_i\right\}\\
	&\overset{(c)}{=}\gO\left(\eta_{t-1} + t^{\alpha - 1} \right) = \gO(t^{\alpha -1})
\end{align*}
where $(a)$ uses $\eta_{i-1} - \eta_i \le \frac{\alpha}{i-1}\cdot \eta_{i-1} \le  2 \alpha\eta_{i-1} \frac{1}{t}$ for $\eta_{i} = i^{-\alpha}$ and $i \ge t$, $(b)$ uses $\left\|\pprod{i}{t}{j}(\sI - \eta_i\sG)\right\|_2 \le c_0\exp\left\{-c\ssum{i}{t}{j}\eta_i\right\}$ and $\eta_{j+1} \ge \eta_t$ for $j+1 \ge t$, and $(c)$ uses $\ssum{j}{t}{n} \eta_{j+1}\ssum{i}{t}{j} \eta_{j}\exp\left\{-c\ssum{i}{t}{j}\eta_i\right\} \precsim \int_0^\infty m \exp(-cm)d m < \infty$.

Finally, we comment that here we use polynomial step sizes that $t^{-\alpha}$ with $\frac{1}{2} < \alpha < 1$ for simplicity.
It is possible to extend to general step sizes using a similar but more complicate argument.
\end{proof}

\subsection{Proof of Lemma~\ref{lem:error1}}
\label{proof:error1}

\begin{proof}[Proof of Lemma~\ref{lem:error1}]
	The proof can be viewed as a quantitative version of that of Lemma~\ref{lem:error0}.
	We suggest readers should be familiar with the notation and proof idea therein before diving into the details of this proof.
	At the beginning, we choose any $p_0 \in [2, p]$.
	
	We first assume $\sG$ is further diagonalizable.
	Recall the definition of $\gA^c$ in~\eqref{eq:setA}.
	Similar to~\eqref{eq:bound-y}, one can show that $\EB\|\vy_{h_k}\|^{p_0} \le {p_0}^{p_0} c_4^{p_0}  \cdot \eta_{h, k}^{\frac{{p_0}}{2}}$.
	By Markov's inequality, it follows that
	\begin{align*}
		\PB(\gA^c) &\le \ssum{k}{0}{n}\PB\left(\frac{c^\prime_0}{\sqrt{T}}\left\|\frac{\vy_{h_k}}{\eta_{h_k}}\right\|\ge \eps \right)\le \frac{(c^\prime_0)^{p_0}}{T^{{p_0}/2}\eps^{p_0}}\ssum{k}{0}{n}\EB\left\|\frac{\vy_{h_k}}{\eta_{h_k}}\right\|^{p_0}\\
		&\le \frac{1}{T^{{p_0}/2}\eps^{p_0}}\ssum{k}{0}{n}\frac{{p_0}^{p_0}C_{3, 1}^{p_0}}{\eta_{h_k}^{{p_0}/2}}\le \frac{{p_0}^{p_0}C_{3,1}^{p_0}n}{(T\eta_T)^{{p_0}/2}\eps^{p_0}}.
	\end{align*}
	where $C_{3,1} := c_0' \cdot c_4 $ for short.
	On the other hand, by Lemma~\ref{lem:P-bound}, we know that for any $k \in [n]$ or $k=0$,
	\begin{equation}
	\label{eq:GPk}
		\gP_k \le \frac{{p_0}^{p_0}C_3^{p_0}}{n^{{p_0}/2}\eps^{p_0}} \le  \frac{{p_0}^{p_0}C_{3,2}^{p_0}}{n^{{p_0}/2}\eps^{p_0}}
	\end{equation}
	where $C_{3,2} := \max\{ C_{3,1}, C_3 \}$ and $C_3$ is defined in Lemma~\ref{lem:P-bound}.
	We comment that though the bound in Lemma~\ref{lem:P-bound} depends on $p$ rather than $p_0$, one can repeat the proof therein to derive the inequality~\eqref{eq:GPk}.
	A shortcut argument can be used is to assume the noise defined therein has $p_0$-th order moments rather than $p$-th ones.
	Then~\eqref{eq:GPk} directly follows by replacing $p$ with $p_0$ in  Lemma~\ref{lem:P-bound}.
	
	Putting these bounds together, we have that for any $\eps >0$,
	\begin{align*}
		\widetilde{d}\left(\bar{\vy}_T\right) &\le \PB\left(\sup\limits_{0\le t\le T}\frac{\|\vy_{t}\|}{\sqrt{T}\eta_t} > 2\eps\right)\vee 2\eps\\
		&\le 2\eps \vee \left\{\PB\left(\sup\limits_{0\le t\le T}\frac{\|\vy_{t}\|}{\sqrt{T}\eta_t} > 2\eps;~\gA\right) + \PB(\gA^c)\right\}\\
		&\le 2\eps \vee \left\{\ssum{k}{0}{n-1}\gP_k + \PB(\gA^c)\right\}\\
		&\precsim  \eps \vee  \left[ \frac{n {p_0}^{p_0} C_{3,2}^{p_0}}{\eps^{p_0}}  \cdot \left(\frac{1}{n^{{p_0}/2}} + \frac{1}{(T\eta_T)^{{p_0}/2}}\right)
		\right]
	\end{align*}
	Since the last inequality holds for any $n$ and $\eps$, we will carefully set $n$ and $\eps$ to make the bound as small as possible.
	First, we set $n = T^{1-\alpha}$ so that $ \frac{1}{n^{{p_0}/2}} = \frac{1}{(T\eta_T)^{{p_0}/2}}$ as a result of $\eta_T = T^{-\alpha}$.
	Therefore,
	\[
	\widetilde{d}\left(\bar{\vy}_T\right) \precsim \eps\vee \frac{{p_0}^{p_0}C_{3,2}^{p_0}}{T^{(1-\alpha)({p_0}/2-1)}\eps^{p_0}}.
	\]
	Then, we let $\eps = {p_0} C_{3,2} \cdot T^{-\frac{({p_0}/2-1)(1-\alpha)}{1+{p_0}}}$ which ensures that $\eps=\frac{C_{3,2}^{{p_0}+1}{p_0}^{{p_0}+1}}{T^{(1-\alpha)({p_0}/2-1)}\eps^{p_0}}$.
	As a result,
	\[
	\widetilde{d}\left(\bar{\vy}_T\right) \precsim  {p_0} C_{3,2} \cdot T^{-\frac{({p_0}/2-1)(1-\alpha)}{1+{p_0}}} \precsim (1+l) \cdot T^{-\frac{l(1-\alpha)}{3+2l}}
	\]
	where the last inequality is because we rewrite $p_0 = 2(1+l)$ with $0 \le l \le \delta$ and $p=2+2\delta$.
	
	We then consider the case where $\sG$ is not diagonalizable.
	The idea is similar to what we did in Section~\ref{proof:error}.
	Let its Jordan decomposition be $\sG = \sV\sJ\sV^{-1} = \sV\diag\{\sJ_1,\cdots,\sJ_r\}\sV^{-1}$, where $\sV$ is the non-singular matrix and $\{ \sJ_i\}_{1\le i \le r}$ collects all Jordan blocks.
	Recall that $\{\y_t\}_{t \ge 0}$ is defined in~\eqref{eq:y}.
	Let $\widetilde{\y}_t = \sV^{-1}\y_t$, $\widetilde{\seps}_t = \sV^{-1}\seps_t$ be transformed vectors. 
	Then the recursion formula~\eqref{eq:y} becomes
	\[
	\widetilde{\y}_{t+1} = (\sI - \eta_t \sJ) \widetilde{\y}_t + \eta_t\widetilde{\seps}_t.
	\]
	Let $\left(\widetilde{\y}_t\right)_k$ denote the $k$-th coordinate of the vector $\widetilde{
		\y}_t$ and so does $\left(\widetilde{\seps}_t\right)_k$.
	The associated process is denoted by
			\[
	(\bar{\widetilde{\vy}}_T)_k(r) = 
	\frac{(\widetilde{\vy}_{\floor{(T+1)r}})_k }{\sqrt{T}\eta_{\floor{(T+1)r}}}
	~ \text{for} ~ r \in [0, 1].\]
	Then it follows that 
	\begin{align*}
		\vertiii{\bar{\y}_T} = 
		\sup_{0 \le t \le T} \frac{\|\y_{t+1}\|}{\sqrt{T}\eta_{t+1}} 
		\precsim 		\sup_{0 \le t \le T} \frac{\|\widetilde{\y}_{t+1}\|}{\sqrt{T}\eta_{t+1}} 
		\le \sum_{k=1}^d \sup_{0 \le t \le T} \frac{|(\widetilde{\y}_{t+1})_k|}{\sqrt{T}\eta_{t+1}} = \sum_{k=1}^d \vertiii{(\bar{\widetilde{\vy}}_T)_k}.
	\end{align*}
which implies
\[
\widetilde{d}(\bar{\y}_T) = \eps \vee \PB(	\vertiii{\bar{\y}_T}  \ge \eps) \precsim \eps \vee \sum_{k=1}^d \PB \left(\vertiii{(\bar{\widetilde{\vy}}_T)_k} \ge \frac{\eps}{d}  \right) \le d  \cdot \sum_{k=1}^d \widetilde{d}((\bar{\widetilde{\y}}_T)_k). 
\]
In the following, we will focus on each coordinate supreme $\vertiii{(\bar{\widetilde{\vy}}_T)_k}$.
	Without loss of generality, we assume $\sG$ is a matrix of Jordan canonical form, that is, $\sJ$ consists of only one Jordan block~\eqref{eq:J}.
	
	Note that the last coordinate process evolves as $(\widetilde{\y}_{t+1})_d = (1-\eta_t \lambda)(\widetilde{\y}_t)_d + \eta_t (\widetilde{\seps}_{t})_d$.
	By what has been established early in this subsection, we have $\widetilde{d}((\bar{\widetilde{\vy}}_T)_d) \precsim (1+l) \cdot T^{-\frac{l(1-\alpha)}{3+2l}}$.
	We are going to finish the proof by induction.
		Suppose that we already have $\widetilde{d}((\bar{\widetilde{\vy}}_T)_i) \precsim (1+l) \cdot T^{-\frac{l(1-\alpha)}{3+2l}}$ for the coordinates $i = k, k+1, \cdots, d$, we will show $\widetilde{d}((\bar{\widetilde{\vy}}_T)_{k-1})$ is also bounded by that quantity.
		Using the structure of $\sJ$ in~\eqref{eq:J}, we have
		\begin{align}
			\tag{\ref{eq:tl_y_updt}}
			(\widetilde{\y}_{t+1})_{k-1} = (1-\lambda\eta_t)(\widetilde{\y}_t)_{k-1} - \eta_t(\widetilde{\y}_t)_k + \eta_t(\widetilde{\seps}_t)_{k-1}.
		\end{align}
		To facilitate analysis, we construct a surrogate sequence $\{(\widehat{\y}_t)_{k-1}\}$ defined by $\widehat{\y}_0 = \0$ and
		\begin{align}
			\tag{\ref{eq:ht_y_updt}}
			(\widehat{\y}_{t+1})_{k-1} = (1 - \lambda\eta_t)(\widehat{\y}_t)_{k-1} + \eta_t(\widetilde{\seps}_t)_{k-1}.
		\end{align}
		Again, we have
		\[
		\widetilde{d}((\bar{\widehat{\y}}_{T})_{k-1} ) \precsim (1+l) \cdot T^{-\frac{l(1-\alpha)}{3+2l}}  
		~\text{with}~
			(\bar{\widehat{\vy}}_T)_k(r) = 
		\frac{(\widehat{\vy}_{\floor{(T+1)r}})_k }{\sqrt{T}\eta_{\floor{(T+1)r}}}
		~ \text{for} ~ r \in [0, 1].
		\]
		Let $\widetilde{\De}_t := \frac{(\widetilde{\y}_{t})_{k-1} - (\widehat{\y}_{t})_{k-1}}{\eta_t}$ be their normalized difference.
		From \eqref{eq:tl_y_updt} $-$ \eqref{eq:ht_y_updt}, it follows that
		\begin{align*}
			\widetilde{\De}_{t+1} =  \frac{(1-\lambda\eta_t)\eta_t}{\eta_{t+1}}\widetilde{\De}_t - \frac{\eta_t^2}{\eta_{t+1}} \cdot \frac{(\widetilde{\y}_t)_{k}}{\eta_t}
		\end{align*}
	There exists an $t_0$ such that $\left|\frac{(1-\lambda\eta_t)\eta_t}{\eta_{t+1}}\right| \le 1 -  0.5 \lambda \eta_t$ for any $t \ge t_0$.
	In this case, for any $t \ge t_0$, 
	\[
|\widetilde{\De}_{t+1}| \le (1-0.5\lambda \eta_t) \cdot |\widetilde{\De}_{t}| + 2\eta_t  \left| \frac{(\widetilde{\y}_t)_{k}}{\eta_t} \right|,
	\]
	by which one can show the following inequality by induction
	\[
	\sup_{t_0 \le t \le T} |\widetilde{\De}_{t+1}|  \le  \frac{4}{\lambda} \cdot \max\left\{
	|\widetilde{\De}_{t_0}|,  	\sup_{t_0 \le t \le T}  \left| \frac{(\widetilde{\y}_t)_{k}}{\eta_t} \right|
	\right\}.
	\]
	One can also show that there exists a constant $C_{3,3} > 0$ depending on $t_0, \lambda$ and $\{\eta_t\}_{0 \le t \le t_0}$ such that 
	\[
		\sup_{0 \le t \le t_0} |\widetilde{\De}_{t+1}|  \le  C_{3,3} \cdot	\sup_{0 \le t \le t_0}  \left| \frac{(\widetilde{\y}_t)_{k}}{\eta_t} \right|.
	\]
	As a result, we know that
	\[
	\frac{1}{\sqrt{T}} \sup_{0 \le t\le T} |\widetilde{\De}_{t+1}|  \precsim \frac{1}{\sqrt{T}}  \sup_{0 \le t\le T}  \left| \frac{(\widetilde{\y}_t)_{k}}{\eta_t} \right|.
	\]
	which implies
	\[
	\widetilde{d}(\bar{\widetilde{\De}}_T) \precsim \widetilde{d}((\bar{\widehat{\y}}_T)_k ) \precsim (1+l) \cdot T^{-\frac{l(1-\alpha)}{3+2l}}
	~\text{with}~
	(\bar{\widetilde{\De}}_T)(r) = 
	\frac{\widetilde{\De}_{\floor{(T+1)r}}}{\sqrt{T}}
	~ \text{for} ~ r \in [0, 1].
	\]
	Finally, we complete the induction by noting
	\[
		\widetilde{d}((\bar{\widetilde{\y}}_{T})_{k-1} )  \le 2(	\widetilde{d}((\bar{\widehat{\y}}_{T})_{k-1} ) + 	\widetilde{d}(\bar{\widehat{\De}}_{T})) \precsim (1+l) \cdot T^{-\frac{l(1-\alpha)}{3+2l}}.
	\]

	\end{proof}

\subsection{Proof of Lemma~\ref{lem:quad_cha_bd}}
\label{proof:quad_cha_bd}
\begin{proof}[Proof of Lemma~\ref{lem:quad_cha_bd}]
	Let $M = \sup_{\xi \in \Xi}\sqrt{ \PM\|\sH(\x^{\star}, \xi)\|^2}$.
	From Assumption~\ref{asmp:futher-noise}, we have $M < \infty$.
	By Lemma~\ref{lem:poisson}, it follows that $\sU(\x^{\star}, \xi) = \sH(\x^{\star}, \xi) + \PM\sU(\x^{\star}, \xi)$ and $\sup_{\xi \in \Xi} \|\PM\sU(\x^{\star}, \xi)\| \le C_U$. 
	Therefore, we have
	\[
	\sup_{\xi \in \Xi} \PM\|\sU(\x^{\star}, \xi)\|^2 \le \sup_{\xi \in \Xi} 2\left[ \PM\|\sH(\x^{\star}, \xi) \|^2 +  \|\PM\sU(\x^{\star}, \xi)\|^2 \right]
	\le 2(M^2 + C_U^2).
	\]
	The last equation implies 
	\begin{align*}
		\EB[\|\su_{t,2}\|^2|\FM_{t-1}] 
		&= \EB [ \|\sU(\x^{\star}, \xi_t)-\PM \sU(\x^{\star}, \xi_{t-1})\|^2|\FM_{t-1} ]\\
		& \le \EB [ \|\sU(\x^{\star}, \xi_t)\|^2| \FM_{t-1}] = \PM \|\sU(\x^{\star}, \xi_{t-1})\|^2 \le 2(M^2 + C_U^2)
	\end{align*}
	is uniformly bounded.
	As a result,
	\begin{equation}
		\label{eq:q-bound}
		q(\xi_{t-1}) := \EB\left[(\ThetaSym^\top\sG^{-1}\su_{t,2})^2| \gF_{t-1}\right] \le2 \|\ThetaSym\|_*^2 \|\sG^{-1}\|^2(M^2 + C_U^2)
	\end{equation}
	is uniformly bounded and thus has any $l$-th order moment where $l > 0$.
	For simplicity, we set $X_t := q(\xi_t)$.
	From~\eqref{eq:q-bound}, we know that the sequence $\{X_t-\EB X_t \}_{t\ge 0}$ has uniform bounded $1+l$-th order moments for any $l \ge 0$. 
	We denote its centralized $L_{1+l}$-norm by 
	\begin{align*}
		M_{1+l} 
		&:= \sup_{t \ge 0} (\EB|X_t-\EB X_t|^{1+l})^{\frac{1}{1+l}}= \sup_{t \ge 0} (\EB|q(\xi_t) - \EB q(\xi_t)|^{1+l})^{\frac{1}{1+l}}.
	\end{align*}
	On the other hand, since we assume $\xi_0 \sim \pi$, then $\xi_t \sim \pi$ and thus
	\begin{align*}
		\EB q(\xi_t)
		= \EB_{\xi \sim \pi, \xi' \sim P(\xi, \cdot)}[(\ThetaSym^\top\sG^{-1}(\sU(\x^{\star}, \xi')-\PM \sU(\x^{\star}, \xi))^2]
		=\ThetaSym^\top\sG^{-1} \sS \sG^{-\top} \ThetaSym .
	\end{align*}
	For simplicity, we denote $q^{\star} = \ThetaSym^\top\sG^{-1} \sS \sG^{-\top} \ThetaSym$.
	Our target quanitity is $\EB\sup\limits_{t\le T}\left|\ssum{i}{0}{t}\{q(\xi_i)- \EB q(\xi_i) \}\right| = \EB \sup\limits_{t\le T}\left|\sum_{i=0}^t (X_i - \EB X_i)\right|$ where the expectation $\EB(\cdot)$ is taken with respect to all randomness.
	To that end, we will make use of moment inequalities for fast mixing random variables in Lemma~\ref{lem:fuk_nagaev}.
	Before starting the analysis, we first introduce additional notations and preliminaries.
	We denote a given one-dimensional random variable $X \in \RB$ by $Q_X(\cdot)$ as the quantile function of $|X|$.
	It is the inverse of the function $x\to \PB(|X|>x)$, defined by $Q_X(u) = \inf\{x: \PB(|X|>x) \le u \}$.
	We present a useful tail bound for $Q(u):= \sup_{t \ge 0} Q_{X_t -\EB X_t}(u)$ which mainly follows from the Markov inequality.
	\begin{equation}
		\label{eq:Q-bound}
		Q(u) \le \left( \frac{1}{u}{\sup_{t \ge 0}\EB|q(\xi_t) - \EB  q(\xi_t) |^{1+l}}\right)^{\frac{1}{1+l}} =
		M_{1+l}u^{-\frac{1}{1+l}}
		\quad \text{for any} \ l \ge 0.
	\end{equation}
	For a sequence of real numbers $\{\alpha_t\}_{t \ge 0}$, we define by the function $\alpha^{-1}(u)$ the counting function on the indexes $t$'s on which $\alpha_t$ is larger then a given input $u$, that is, $\alpha^{-1}(u):= \ssum{t}{0}{\infty}\mathbbm{1}_{u<\alpha_t}$.

	\begin{defn}[$\alpha$-mixing coefficients]
		\label{def:mix}
		Given two $\sigma$-field $\AM$ and $\BM$, the strong mixing coefficient between them is defined by
		\[
		\alpha(\AM, \BM) := 2 \sup \left\{ \mathrm{Cov}(1_A, 1_B): A \in \AM, B \in \BM \right\}
		\]
		where $1_A$ is the indicator function of the event $A$ and similar is $1_B$.
	\end{defn}
	
	\begin{defn}[Strong mixing coefficients~\citep{rosenblatt1956central}]
		\label{def:strong}
		Let $\{X_t\}_{t > 0}$ be a sequence of real-valued random variables.
		Set $\FM^{\mathrm{l}}_k = \sigma(\{X_t\}_{t \le k})$ and $\FM^{\mathrm{u}}_l = \sigma(\{X_t\}_{t \ge l})$.
		The strong mixing coefficients of $\{X_t\}_{t> 0}$ are denoted by $\{\alpha_t\}_{t \ge 0}$ with definition as what follows
		\[
		\alpha_0 = 1/2
		\quad \text{and} \quad
		\alpha_t = \sup_{k \in \mathbb{N}} \alpha(\FM^{\mathrm{l}}_k,\FM^{\mathrm{u}}_{k+t})
		\quad \text{for any} \quad t \ge 1.
		\]
	\end{defn}

	\begin{lem}[Theorem 6.3 in \citet{rio2013inequalities}]
		\label{lem:fuk_nagaev}
		Let $\{X_t\}_{t>0}$ be a sequence of real-valued and centered random variables and $\{\alpha_t\}_{t\ge 0}$ be the corresponding strong mixing coefficients. 
		Suppose that, for some $p\ge 2$, $\sup_{t > 0}\EB|X_t|^p < \infty$. Then with $S_k = \sum_{t=1}^k X_t$, we have
		\[
		\EB\left(\sup\limits_{1\le k\le n}|S_k|^p\right) \le a_p \left(\sum_{i=1}^n \sum_{j=1}^n\left|\operatorname{Cov}\left(X_i, X_j\right)\right|\right)^\frac{p}{2} + nb_p\int_0^1 \left[\alpha^{-1}(u)\wedge n\right]^{p-1}Q^p(u)du,
		\]
		where
		\[
		Q := \sup\limits_{t>0}Q_{X_t}, \quad a_p = p4^{p+1}(p+1)^{p/2} \quad \text{ and } \quad  b_p = \frac{p}{p-1}4^{p+1}(p+1)^{p-1}.
		\]
	\end{lem}

Lemma~\ref{lem:fuk_nagaev} replies on the concept of strong mixing coefficients which we introduce in Definition~\ref{def:strong}.
	By Lemma~\ref{lem:mixing}, we know that the the strong mixing coefficients of $\{\xi_t\}_{t \ge0}$ is mixing exponentially fast.
		With this result, we can compute the bounds in Lemma~\ref{lem:fuk_nagaev} as follows.
	\begin{lem}[Fast mixing]
		\label{lem:mixing}
		Under Assumption~\ref{asmp:markov-noise}, the strong mixing coefficients of $\{\xi_t\}_{t \ge0}$ vanishes exponentially fast, that is, $\alpha_t \le \kappa \rho^t$ with $\kappa > 0$ and $\rho \in [0, 1)$ given in Assumption~\ref{asmp:markov-noise}.
	\end{lem}
	
	We first compute that for any $i < j$,
	\begin{align*}
		\mathrm{Cov}(X_i, X_j) 
		&= \EB (X_i- \EB X_i)(X_j -\EB X_j)\\
		&\overset{(a)}{=} \EB \left[ (X_i- \EB X_i) \EB[X_j -\EB X_j|\FM_i] \right] \\
		&\overset{(b)}{=} \EB (X_i- \EB X_i) (\PM^{j-i} X_i-\EB X_j)\\
		&=\EB [(X_i- \EB X_i)(\PM^{j-i}X_i- q^{\star})] \\
	    &\overset{(c)}{\le} \EB|X_i- \EB X_i|  \cdot \kappa \rho^{j-i} \sup_{\xi}|q(\xi) - q^{\star}| \\
		& \le \kappa M_1M_{\infty} \rho^{j-i},
	\end{align*}
	where $(a)$ uses the law of total expectation and the notation $\FM_i = \sigma(\{\xi_t\}_{t \le i})$, $(b)$ uses the equality $ \EB[X_j|\FM_i]=\PM^{j-i} X_i$ due to the Markov property, and $(c)$ follows from Lemma~\ref{lem:geo-con}.
	Therefore,
	\begin{align}
		\ssum{i}{1}{T}\ssum{j}{1}{T}|\mathrm{Cov}(X_i, X_j)| &= \ssum{i}{1}{T}\EB|X_i- \EB X_i|^2 + 2\sum\limits_{1\le i < j\le n}|\mathrm{Cov}(X_i, X_j)| \nonumber \\
		&\precsim TM_2^2 + 2\rho\kappa M_1 M_{\infty}\sum\limits_{1\le i < j\le T}\rho^{j-i} \nonumber \\
		& = T M_2^2 + 2\rho\kappa M_1M_{\infty}\ssum{i}{1}{T-1}\ssum{k}{0}{T-i-1}\rho^{k} \nonumber \\
		&\le T\left( M_2^2 + \frac{2\rho\kappa M_1M_{\infty}}{1-\rho}\right) \le T\left( M_2^2 + 2\kappa M_1M_{\infty} t_{\mathrm{mix}} \right).
		\label{eq:sum-covaraince}
	\end{align}
	Now, we apply Lemma~\ref{lem:fuk_nagaev} with $p = 2$ and obtain
	\begin{align*}
		&\EB\sup\limits_{t\le T}\left|\ssum{i}{0}{t}\{X_i - \EB X_i\}\right| \le \left\{\EB\sup\limits_{t\le T}\left|\ssum{i}{0}{t}\{X_i - \EB X_i\}\right|^2\right\}^{\frac{1}{2}}\\
		&\precsim \left\{\ssum{i}{1}{T}\ssum{j}{1}{T}|\mathrm{Cov}(X_i,X_j)| + T\int_0^1\alpha^{-1}(u)Q(u)^2du\right\}^{\frac{1}{2}}\\
		&\overset{(a)}{\le} \left\{T\left(M_2^2 + 2\kappa M_1 M_{\infty} t_{\mathrm{mix}}\right) + T\int_0^1\left(\ssum{j}{0}{\infty}\mathbbm{1}_{u<\alpha_j}\right)Q(u)^2du\right\}^{\frac{1}{2}}\\
		& = \left\{T\left(M_2^2 +  2\kappa M_1 t_{\mathrm{mix}} \right) + T\ssum{j}{0}{\infty}\int_0^{\alpha_j}Q(u)^2du\right\}^{\frac{1}{2}}\\
		&\overset{(b)}{\le} \left\{T\left(M_2^2 +  2\kappa M_1 M_{\infty} t_{\mathrm{mix}} \right) + \frac{1+l}{l - 1} M_{1+l}^2
		T\ssum{j}{0}{\infty}\alpha_j^{\frac{l-1}{1+l}}\right\}^{\frac{1}{2}}\\
		&\overset{(c)}{\le} \left\{T\left(M_2^2 + 2\kappa M_1M_{\infty} t_{\mathrm{mix}} \right) + \frac{\kappa^{\frac{l - 1}{1 + l}}}{1 - \rho} M_{1+l}^2
		\left(\frac{1+l}{l - 1}\right)^2T\right\}^{\frac{1}{2}}\\
		&\precsim T^{\frac{1}{2}}\left\{M_2^2 +  t_{\mathrm{mix}} \left(\kappa M_1M_{\infty} +\kappa^{\frac{l - 1}{1 + l}} M_{1+l}^2\left(\frac{1+l}{l - 1}\right)^2\right)\right\}^{\frac{1}{2}}\\
		&\overset{(d)}{\precsim} \sqrt{T(M_2^2 +  \kappa t_{\mathrm{mix}} \left( M_1 M_{\infty}+ M_{\infty}^2 \right) )} 
		\precsim \sqrt{T(1+\tmix )} \overset{(e)}{\le}  \sqrt{T \tmix }
	\end{align*}
	where $(a)$ holds due to the bound~\eqref{eq:sum-covaraince} for the sum of covariance, and $(b)$ holds due to the inequality~\eqref{eq:Q-bound}, and $(c)$ uses Lemma~\ref{lem:mixing} and the inequality that $\left( 1-\rho^{\frac{\delta-1}{\delta+1}}\right)^{-1} \le \frac{1}{1-\rho} \frac{\delta+1}{\delta-1}$, $(d)$ follows by setting $l \to \infty$, and $(e)$ uses the fact that $\tmix \ge 1$ when $\tmix > 0$.
\end{proof}

In the end, we provide the proof for Lemma~\ref{lem:mixing}.
\begin{proof}[Proof of Lemma~\ref{lem:mixing}]
	From Section 3 in~\citep{bradley2005basic}, we know that if $\{\xi_t\}_{t > 0}$ is a (not necessarily stationary) Markov chain, then by the Markov property and an elementary argument, 
	\[
	\alpha_t = \sup_{k \in \mathbb{N}}\alpha(\sigma(\xi_k), \sigma(\xi_{k+t})).
	\]
	By Definition~\ref{def:mix}, it follows that
	\[
	\alpha(\sigma(\xi_k), \sigma(\xi_{k+t})) 
	= 2 \sup \left\{ \mathrm{Cov}(1_{\xi_k \in A}, 1_{\xi_{k+t} \in B}): \text{both} \ A, B \ \text{measurable} \right\}.
	\]
	In the following, we fix $k \in \mathbb{N}$ and two measurable sets $A, B$.
	For simplicity, we denote $h_1(\xi_k) = 1_{\xi_k \in A} - \PB(\xi_k \in A)$ and $h_2(\xi_{k+t}) = 1_{\xi_{k+t} \in B} - \PB(\xi_{k+t} \in B)$.
	It then follows that
	\begin{align*}
		\mathrm{Cov}(1_{\xi_k \in A}, 1_{\xi_{k+t} \in B})
		&= \EB h_1(\xi_k) h_2(\xi_{k+t})
		= \EB[h_1(\xi_k)\EB[ h_2(\xi_{k+t})| \FM_k ]]\\
		&=\EB [h_1(\xi_k) \PM^t h_2(\xi_{k})]\\
		&=\EB [h_1(\xi_k) (\PM^t h_2(\xi_{k})-\EB_{\xi \sim \pi} h_2(\xi))] +  \EB h_1(\xi_k) \cdot \EB_{\xi \sim \pi} h_2(\xi)\\
		&\overset{(a)}{=}\EB [h_1(\xi_k) (\PM^t h_2(\xi_{k})-\EB_{\xi \sim \pi} h_2(\xi))] \\
		&\le \EB |h_1(\xi_k)| \cdot |\PM^t h_2(\xi_{k})-\EB_{\xi \sim \pi} h_2(\xi)|
		\overset{(b)}{\le}  \EB |h_1(\xi_k)| \cdot \kappa \rho^t  \le \kappa \rho^t,
	\end{align*}
	where $(a)$ uses $\EB h_1(\xi_k)=0$ and $(b)$ uses Lemma~\ref{lem:geo-con} and the fact that both $h_1(\cdot)$ and $h_2(\cdot)$ are uniformly bounded by 1.
	Taking maximum over all $k \in \mathbb{N}$ and measurable sets $A, B$, we conclude that
	$\alpha_t \le \kappa \rho^t$.
\end{proof}

\section{Omitted proof in Section~\ref{sec:inference}}

This section collects omitted proofs in Section~\ref{sec:inference}.

\subsection{Proof of Theorem~\ref{thm:fclt-c}}
\begin{proof}[Proof of Theorem~\ref{thm:fclt-c}]
	One can show that $\vertiii{\ph_T - \phc_T} = o_{\PB}(1)$ by noting the equality $\vertiii{\ph_T - \phc_T} = \frac{1}{\sqrt{T}} \sup_{n \in [T]}  \|\x_t-\x^*\|$ and the fact that
	\[
	\frac{1}{T}\EB  \sup_{t \in [T]}  \|\x_t-\x^*\|^2  \le \frac{1}{T} \sum_{t=1}^T \EB  \|\x_t-\x^*\|^2  \precsim \frac{\log T}{T} \sum_{t=1}^T \eta_t \to 0.
	\]
	Hence, we know that $\phc_T \overset{w}{\to} \Bpsi$ in the Skorokhod topology.
	That is for any bounded and $\dS$-continuous functional $h: \BDD \to \RB$, we have $\EB h(\phc_T) \to \EB h(\Bpsi)$.
	Note that any bounded and $\vertiii{\cdot}$-continuous functional $h: \BCD \to \RB$ can be viewed as a bounded and $\dS$-continuous functional $\BDD \to \RB$.
	Hence, $\EB h(\phc_T) \to \EB h(\Bpsi)$ holds for any bounded and $\vertiii{\cdot}$-continuous functional $h: \BCD \to \RB$.
	It is equivalent to $\phc_T \overset{w}{\to} \Bpsi$ in the uniform topology.
\end{proof}

\subsection{Proof of Theorem~\ref{thm:abs-error}}
\begin{proof}[Proof of Theorem~\ref{thm:abs-error}]
	Recall that $\phi_T = \ThetaSym^\top \phc_T$ and $\psi =\ThetaSym^\top \Bpsi$.
	Let $B_x := \left\{  \phi: |f_m(\phi)| > x \right\}$ and $\epsP = \dP(\ThetaSym^\top\phc_T,  \ThetaSym^\top \Bpsi)$.
	From Proposition~\ref{prop:functional}, the functional $f_m$ is continuous such that $B_x$ is a measurable set in its Borel $\sigma$-field $\BCMO$.
	By the definition of the L\'evy-Prokhorov distance in $\BCO$, we have
	\[
	\PB(\phi_T \in B_x) \le \PB( \psi \in B_x^{\epsP}) + \epsP
	\quad \text{and} \quad
	\PB(\phi_T \in B_x^c) \le \PB(\psi \in (B_x^c)^{\epsP}) + \epsP
	\]
	where $B_x^{\eps}$ is the $\eps$-neighborhood of $B_x$ defined as following and $B_x^c$ is the complementary set of $B_x$,
	\[
	B_x^{\eps} = \left\{
	\phi_1  \in \BCO: \exists \phi_2 \in \BCO~\text{such that}~\vertiii{\phi_1-\phi_2} \le \eps~\text{and}~\phi_2 \in B_x
	\right\}.
	\]
	%	Since $f_m$ is scale-invariant, we have that $f_m(\psi) \overset{d}{=} f_m(W)$.
	Then, it follows that
	\begin{gather}
		\PB( |f_m(\phi_T)| > x) -\PB(|f_m(\psi)| > x) \le \PB(\psi \in B_x^{\epsP}, \psi \notin B_x) + \epsP,  \label{eq:upper} \\
	\PB(|f_m(\psi)| > x) -	\PB( |f_m(\phi_T)| > x) \le \epsP + \PB(\psi \in B_x, \psi \notin (B_x^c)^{\epsP}) .\label{eq:lower}
	\end{gather}
	
	We rewrite $f_m (\phi)= \frac{\phi(1)}{h_m(\phi)}$ where $h_m (\phi) = \sqrt[m]{\int_0^1 (\phi(r)-r\phi(1))^mdr}$ denotes the integral functional.
	By the Minkowski inequality, we know that $h_m(\phi)$ is a $1$-Lipschitz $\vertiii{\cdot}$-continuous functional in the sense that for any $\phi_1, \phi_2 \in \BCMO$, $|h_m(\phi_1)-h_m(\phi_2)| \le \vertiii{\phi_1-\phi_2}$.
	Furthermore, we have
	\begin{prop}
		\label{prop:con}
		When $h_m(\phi_1) \ge z, h_m(\phi_2) \ge z$ and $|f_m(\phi_1)| \le x$, one can show that
		\[
		|f_m(\phi_1) - f_m(\phi_2)| \le  \frac{1+x}{z} \vertiii{\phi_1-\phi_2}.
		\]
	\end{prop}
	\begin{proof}[Proof of Proposition~\ref{prop:con}]
		It follows that
		\begin{align*}
			|f_m(\phi_1) - f_m(\phi_2)|  
			&\le \left| \frac{\phi_1(1)}{h_m(\phi_1)} - \frac{\phi_1(1)}{h_m(\phi_2)}\right|
			+  \left| \frac{\phi_2(1)}{h_m(\phi_2)} - \frac{\phi_2(1)}{h_m(\phi_2)}\right|\\
			&\le  \left| \frac{\phi_1(1)}{h_m(\phi_1)} \right| \cdot  \frac{|h_m(\phi_1)-h_m(\phi_2)|}{|h_m(\phi_2)|} +  \frac{|\phi_2(1)-\phi_1(1)|}{|h_m(\phi_2)|}\\
			&\le \frac{x}{z} \vertiii{\phi_1-\phi_2} +  \frac{1}{z} \vertiii{\phi_1-\phi_2} =  \frac{1+x}{z} \vertiii{\phi_1-\phi_2}.
		\end{align*}
	\end{proof}
	
	We then proceed to simplify~\eqref{eq:upper}. It follows that
	\begin{align*}
		\PB&(\psi \in B_x^{\epsP}, \psi \notin B_x)
		= \PB\left( |f_m(\psi)| \le x~\text{and}~\exists \TW~\text{satisfying}~\vertiii{\TW-\psi} \le \epsP, |f_m(\TW)| > x\right)\\
		&\le \PB\left( |f_m(\psi)| \le x~\text{and}~\exists \TW~\text{satisfying}~\vertiii{\TW-\psi} \le \epsP, |f_m(\TW)| > x, h_m(\psi) \ge z, h_m(\TW) \ge z\right)\\
		&\qquad  + \PB\left(|f_m(\psi)| \le x~\text{and}~\forall \TW~\text{satisfying}~\vertiii{\TW-\psi} \le \epsP, h_m(\TW) < z\right) \\
		&\qquad +  \PB(|f_m(\psi)| \le x~\text{and}~h_m(\psi) < z)  \\
		&\le \PB\left(  x -  \frac{x+1}{z} \epsP \le |f_m(\psi)| \le x  \right) + 2 \PB \left( |f_m(\psi)| \le x~\text{and}~h_m(\psi) \le z \right)\\
		&= r(|f_m(\psi)|, x) \cdot \frac{x+1}{z} \cdot \epsP  +  2 \PB \left( |f_m(\psi)| \le x~\text{and}~h_m(\psi) \le z \right)+ o(\epsP),
%			&\le \PB\left(  x -  \frac{x+1}{z} \epsP \le |f_m(\psi)| \le x  \right) + 2 \PB \left(h_m(\psi) \le z  \right),
	\end{align*}
	where the second inequality uses Proposition~\ref{prop:con} and the $1$-Lipschitz $\vertiii{\cdot}$-continuity of $h_m$ and the last inequality uses the definition of differentiability.
	
	By a similar argument, for any $z > \epsP$, we simplify~\eqref{eq:lower} to
	\begin{align*}
		\PB&(\psi \in B_x, \psi \notin (B_x^c)^{\epsP})
		= \PB\left( |f_m(\psi)| > x~\text{and}~\forall \TW~\text{satisfying}~\vertiii{\TW-\psi} \le \epsP, |f_m(\TW)| > x\right)\\
		&\le \PB\left( |f_m(\psi)| > x~\text{and}~\forall \TW~\text{satisfying}~\vertiii{\TW-\psi} \le \epsP, |f_m(\TW)| > x, h_m(\psi) \ge z-\epsP, h_m(\TW) \ge z-\epsP \right)\\
		&\qquad + \PB\left(|f_m(\psi)| > x~\text{and}~\exists \TW~\text{satisfying}~\vertiii{\TW-\psi} \le \epsP, h_m(\TW) < z-\epsP\right) \\
		&\qquad + \PB(|f_m(\psi)| > x~\text{and}~h_m(\psi) < z-\epsP)  \\
		&\le \PB\left(  x \le |f_m(\psi)| \le  x + \frac{x+1}{z-\epsP}  \epsP\right) + 2 \PB \left(|f_m(\psi)| > x~\text{and}~ h_m(\psi) \le z \right)\\
		&= r(|f_m(\psi)|, x) \cdot \frac{x+1}{z-\epsP} \cdot \epsP  +  2 \PB \left( |f_m(\psi)| > x~\text{and}~h_m(\psi) \le z \right)+ o(\epsP),\\
		&= r(|f_m(\psi)|, x) \cdot \frac{x+1}{z} \cdot \epsP  +  2 \PB \left( |f_m(\psi)| > x~\text{and}~h_m(\psi) \le z \right)+ o(\epsP).
%				&\le \PB\left(  x \le |f_m(\psi)| \le  x + \frac{x+1}{z}  \epsP\right) + 2 \PB \left(h_m(\psi) \le z + \epsP \right).
	\end{align*}
	Combing these bounds for~\eqref{eq:upper} and~\eqref{eq:lower}, we have for any $z > 0$
	\[
	|\PB( |f_m(\phi_T)| > x) -\PB(|f_m(\psi)| > x)| \le  r(|f_m(\psi)|, x) \cdot \frac{x+1}{z}  \cdot \epsP + 2 \cdot \mathrm{Prob}_m(x, z)  + o(\epsP).
	\]
	where
	\[
	\mathrm{Prob}_m(x, z) = \max \left\{
	\PB \left( |f_m(\psi)| > x~\text{and}~h_m(\psi) \le z \right), \PB \left( |f_m(\psi)| \le x~\text{and}~h_m(\psi) \le z \right)
	\right\}.
	\]
		Let $\omega=\|\ThetaSym^\top \sG^{-1}\sS^{1/2}\|_2$.
		We then have that $\psi \overset{d}{=} \omega W$. 
		On one hand, we note that $r(|f_m(\psi)|, x) = 2 \cdot r(f_m(\psi), |x|) = 2 \cdot r(f_m(W), |x|)$ due to the symmetry of the probability density function of $f_m(\psi)$ and its scale-invariance, i.e., $f_m(\psi) \overset{d}{=} f_m( \omega W) = f_m(W)$.
		On the other hand,
		we have $h_m(\psi) \overset{d}{=} \omega h_m(W)$.
		Therefore,
		\[
		\mathrm{Prob}_m(x, z) = \max \left\{
		\PB \left( |f_m(W)| > x~\text{and}~h_m(W) \le \frac{z}{\omega} \right), \PB \left( |f_m(W)| \le x~\text{and}~h_m(W) \le \frac{z}{\omega} \right)
		\right\}
		\]
	Finally,we complete the proof by replacing $z$ with ${z}{\omega}$ and still denote the last equation as $\mathrm{Prob}_m(x, z)$ with a slight abuse of notation.
\end{proof}

\subsection{Proof of Corollary~\ref{cor:rate}}

\begin{proof}[Proof of Corollary~\ref{cor:rate}]
	We omit the dependency on $m$ for simplicity.
%By $r(h(W), x) =  a \cdot  x^{b} + o(x^{b})$, we have when $x \to 0$,
%\[
%\frac{r(h(W), x) -  a \cdot  x^{b} }{x^b} = o(1).
%\]
%As a result, by intermediate value theorem, there exists $z \in (0, y)$ such that when $y \to 0$,
%\[
%\frac{\int_0^y (r(h(W), x) -  a \cdot  x^{b} ) d x}{y^{1+b}} = \frac{z^b}{y^b}  \cdot \frac{r(h(W), z) -  a \cdot  z^{b} }{z^b} = o(1).
%\]
%Therefore, we have $\PB(h(W) \le x) = \int_0^y r(h(W), x) dx= \frac{a}{b+1} x^{b+1} + o(x^{b+1}) $.
%We then complete the proof by setting $z = \left(  \frac{r(f_m(W), x) \cdot (x+1)  \omega^{b+1}}{a}\epsP \right)^{\frac{1}{b+2}}$.
The corollary follows by noting $\mathrm{Prob}_m(x, z) \le \PB(h_m(W) \le z) =  a_m \cdot  z^{b_m} + o(z^{b_m})$ for any $x > 0$ and using the particular choice of $z = \left(  \frac{r(f_m(W), x) \cdot (x+1)  \omega^{b_m}}{a_m}\epsP \right)^{\frac{1}{b_m+1}}$.

\end{proof}

\section{Additional experimental details}

\paragraph{Further details for Table~\ref{table:linear}}
Each time we initialize $\x_0$ as a zero vector, set $\eta_t = d^{-0.5} t^{-0.505}$, and always abandon the first $5\%$ iterates for a warm up.
We set $d=10$ and $\rho_{\eps} = 0.9$ in all experiments.
The bootstrap method discards the first $400$ samples as a warm up.
According to~\citet{ramprasad2021online}, we set the step size as $\eta_t = 0.75 \cdot t^{-0.75}$ and use $B \in \{10, 100, 200\}$.

%\paragraph{Further details for Table~\ref{table:logistic}}
%The model is given by 
%\[
%\a_t \overset{i.i.d.}{\sim} \NM(\0, \sI_d),~y_t = \mathrm{Sigmoid}(\langle \a_t, \x^{\star} \rangle) + \zeta_t,~\zeta_t = \rho_{\eps}\cdot \zeta_{t-1} 
%+\eps_t,  \eps_t \overset{i.i.d.}{\sim} \sqrt{d} \cdot \mathrm{Uniform}(\mathbb{B}_{d-1}),
%\]
%where $\mathrm{Sigmoid}(x) =\frac{e^x}{1+e^x}$ is the sigmoid function.
%The step size is set  $\eta_t = 2 \cdot t^{-0.505}$.
%We set $d=10$ and $\rho_{\eps} = 0.9$ in all experiments.
%Since nonlinear regression takes more iterations to achieve the nominal coverage rate, we set $T = 10^5$.

\paragraph{Details bout Figure~\ref{fig:mdp}}
The random MDP is generated in a similar way as~\citep{li2021polyak}.
In particular, for each $(s,a)$ pair, the random reward $R(s,a)\sim \NM(r(s, a), 1)$ is normally distributed with the mean $r(s, a)$ sampled from $[0, 1]$ uniformly initially and the transition probability $P(s'|s,a)=u(s')/\sum_{s}u(s)$, where $u(s)\overset{i.i.d.}{\sim}\UM(0,1)$. 
We choose the MDP size to be $|\SM|=|\AM|=5$ and $\gamma = 0.6$.
More iterations are required to conduct statistical inference in larger MDPs with larger $\gamma$.
We choose a zero initial Q-value function.
We abandon the first $4000$ iterates as a warm up and use the following $50000$ iterates to conduct statistical inference.
We repeat the process for $200$ times and use the polynomial step size $\eta_t=(t+1)^{-0.51}$ and zero initial point each time.

\paragraph{Details bout Figure~\ref{fig:logistic}}
We abandon the first $3000$ iterates as a warm-up and use the following $40000$ iterates to conduct statistical inference.
Here we set $d=5$.
Both $\a_0$ and $\x_0$ are initialized as zero vectors.
Larger $d$ requires more iterations and more carefully parameter tuning to produce comparable performance.
We set the step size as $\eta_t = t^{-0.501}$ for all the experiments in this figure.
The target parameter is $\ThetaSym^\top\x^{\star}$ where $\ThetaSym = (1, \cdots, 1)^\top/\sqrt{d} \in \RB^d$ and $\x^{\star}$'s coordinates evenly spread in the interval $[0, 1]$.

\paragraph{Details bout Figure~\ref{fig:logistic-sensitivity}}
The problem dimension is $d=5$ where both $\a_0$ and $\x_0$ are initialized as zero vectors.
The target parameter is $\ThetaSym^\top\x^{\star}$ where $\ThetaSym = (1, \cdots, 1)^\top/\sqrt{d} \in \RB^d$ and $\x^{\star}$'s coordinates evenly spread in the interval $[0, 1]$.
For experiments in the first row, we abandon the first $3000$ iterates as a warm-up and use the following $50000$ iterates to conduct statistical inference.
The step size $\eta_t = t^{-\alpha}$.
For experiments in the second row, we again abandon the first $3000$ iterates as a warm-up and use the following $50000$ iterates to conduct statistical inference.
The step size $\eta_t = \eta t^{-0.501}$.
For experiments in the last row, we again abandon the first $N$ iterates as a warm-up and use the following $50000$ iterates to conduct statistical inference.
The step size $\eta_t =  t^{-0.501}$.
